# Supplementary material for: Taming the Beast: Learning to Control Neural Conversational Models
Source: arXiv:2108.10561 source file (2021-08-24)
Supplement: Supplementary file 1 [file appendix.tex]

\chapter*{Appendix}

\section*{Chapter 3: Controlling Style and Topics}

\section*{A Hyperparamters}
In Table~\ref{tab:hyperparamter}, we report the full set of hyperparameters used in the experiments section. DialoGPT~\cite{zhang2019dialogpt} medium has 345M parameters, 24 layers and $d_{model}=1024$. For adapter we use bottleneck size $m=100$, resulting in additional 5.175M parameters (1.5\%).

\begin{table}[h]
    \centering
    \resizebox{\textwidth}{!}{
    \begin{tabular}{l|l|l}
    \hline
    Model       & Attributes & Hyperparameters \\ \hline
    \textit{PPLM} & \begin{tabular}[c]{@{}l@{}}negative, question, Business,\\ Sports, Sci/Tech\end{tabular}            &  $\alpha = 0.02, p=75, \gamma=1.0, \lambda_{KL} = 0.01 $\\ \hline
    \textit{PPLM} & positive   &    $\alpha = 0.02, p=25, \gamma=1.0, \lambda_{KL} = 0.01$             \\ \hline
    \textit{ADAPTER} & \begin{tabular}[c]{@{}l@{}}negative, positive, question, \\ Business, Sports, Sci/Tech\end{tabular} &  $lr=6.25\mathrm{e}{-4}, batch\_size=32, epoch=5, \lambda_{KL}=0.5$  \\ \hline
    \end{tabular}
    }
    \caption{The full set of hyperparameters used in the experiments. Here, $\lambda_{KL}$ denotes the weight of Kullback–Leibler loss constraint for language model. All the experiments have been run on several NVIDIA 1080Ti.}
    \label{tab:hyperparamter}
\end{table}

\section*{B Automatic Evaluation Datasets Statistics and Performance}
In Table~\ref{tab:autoeval}, we summarize the dataset statistics and performance of the trained scorer.
\begin{table}[h]
\centering
\begin{tabular}{r|c|c|cc|cc}
\hline
\multicolumn{1}{c|}{\multirow{2}{*}{\textbf{Task}}} & \multirow{2}{*}{\textbf{Style}} & \multirow{2}{*}{\textbf{\#C}} & \multicolumn{2}{c|}{\textbf{Samples}} & \multicolumn{2}{c}{\textbf{F1-Score}} \\ \cline{4-7} 
\multicolumn{1}{c|}{} &  &  & \textit{Train} & \textit{Test} & \textit{Train} & \textit{Test} \\ \hline
\textit{AMAZON 5}~\cite{mcauley2013hidden} & Sentiment & 5 & 3M & 650K & 59.13 & 59.11 \\ \hline
% \textit{Wiki Toxic}~\cite{wulczyn2017ex} & Toxic & 2 & 69526 & 23178 & 78.61 & 76.08 \\ \hline
\textit{AG NEWS (R)}~\cite{zhang2015character} & Topic & 4 & 7600 & 120000 & 92.47 & 90.21 \\ \hline
\end{tabular}
\caption{Automatic evaluation datasets statistics and performance.}
\label{tab:autoeval}
\end{table}

\section*{C Additional Details of Human Evaluation}
\label{appendix:human_eval}
We collect human annotations for both Humanness and Attribute Consistency via crowd-sourcing platform provided by Appen Limited\footnote{\url{https://client.appen.com/}}. The template for human evaluation is shown in Figure~\ref{fig:template}. To get consistent observation, we use the same 30 randomly selected prefix of the dialogues across the comparisons. Each annotator is asked to judge either humanness or styleness of 5 different dialogues. In this way, we collect in total 4200 human annotation. % P-values are computed at $\alpha = 0.05$.

\begin{figure}[t]
    \centering
    \begin{subfigure}[t]{0.45\textwidth}
         \centering
         \includegraphics[width=\textwidth]{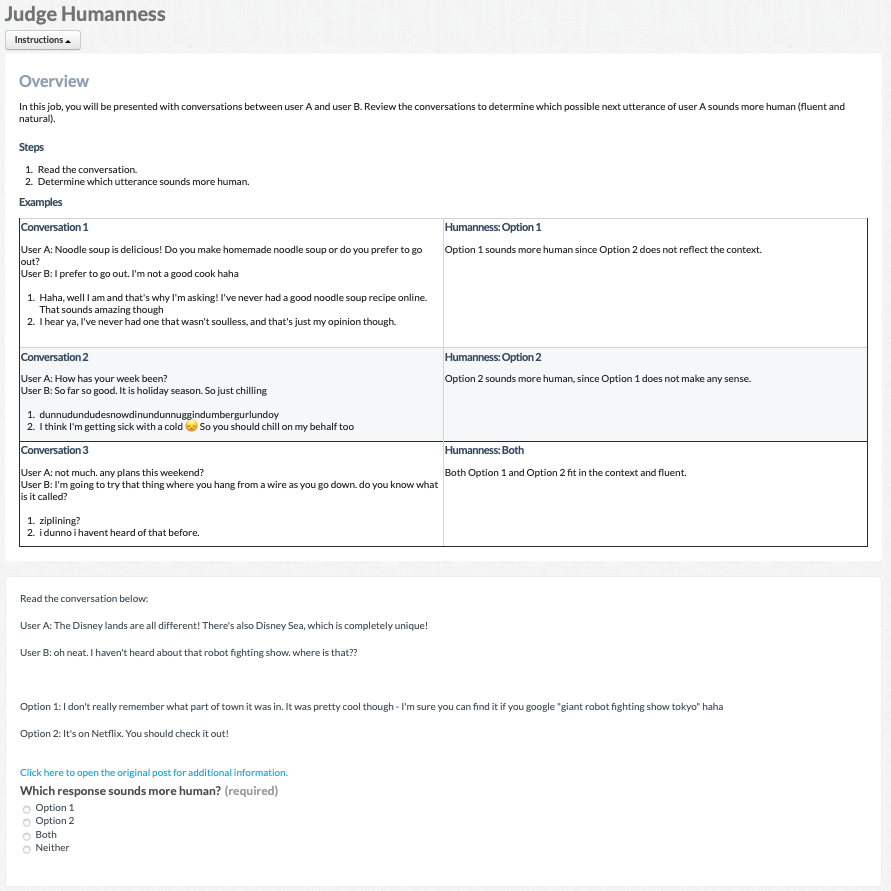}
         \caption{Template for judge humanness. Across all the style, the instructions kept to be same.}
         \label{fig:template_human}
     \end{subfigure}
     ~
     \begin{subfigure}[t]{0.45\textwidth}
         \centering
         \includegraphics[width=\textwidth]{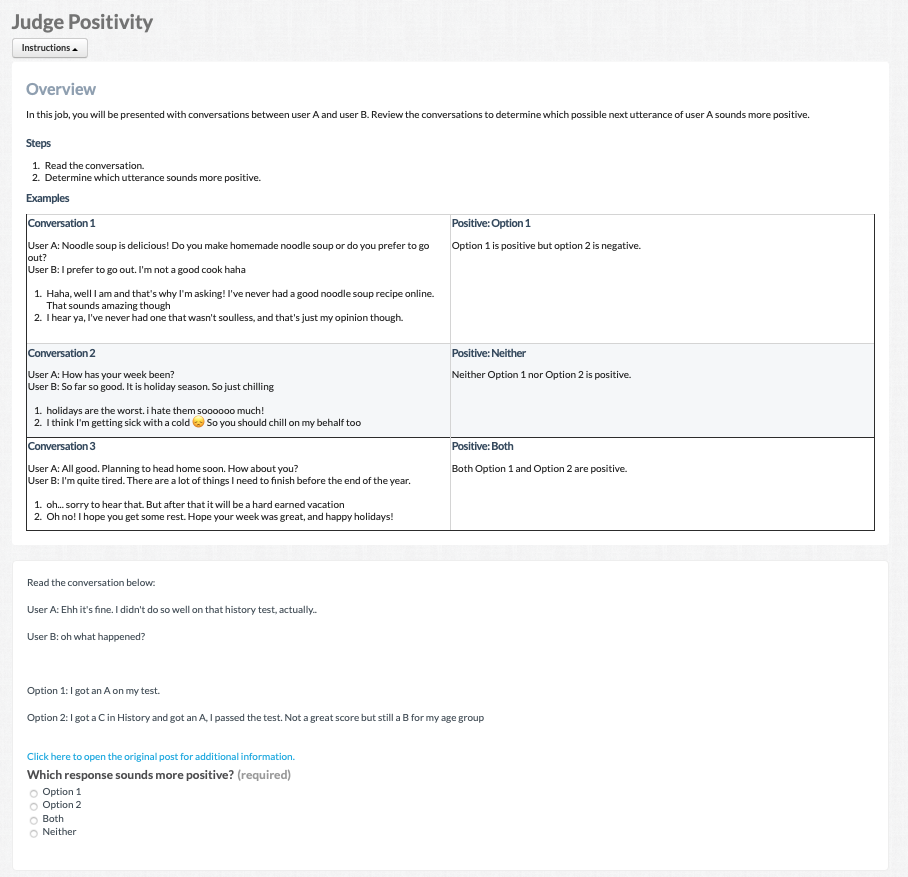}
         \caption{Template for judge style. Depending on the target style, the instructions and the questions asked are modified.}
         \label{fig:template_style}
     \end{subfigure}
    \caption{Human evaluation template for judge humanness and style respectively.}
    \label{fig:template}
\end{figure}

\newpage

\section*{D Additional Details on Results}
In this section, we present additional details on the experimental results, such as the attribute-specific vocabulary, and breakdown of human evaluation results per model comparison. Moreover, from Section~\ref{appendix:negative} to Section~\ref{appendix:scitech}, we report breakdown results of both automatic and human evaluation per style as well as additional examples of generated responses.

\subsection*{Attribute-Specific Vocabulary}
In Table~\ref{tab:top10_style} and Table~\ref{tab:top10_topic}, top 10 frequent attribute-specific words of adapters trained with PPLM are listed. We extract attribute-specific words from 200 dialogues per attribute by taking words that appear more than 5 times in some attribute yet never appear in the other attributes. As can be seen clearly in Table~\ref{tab:top10_style} and Table~\ref{tab:top10_topic}, adapters trained with PPLM are optimized to restrict the vocabulary for each style and topic. Note that the words list of the style question is not clear since it tends to ask a general question such as ``What do you mean?", ``How about you?", or ``How much does it cost?"
\begin{table}[h]
    \centering
    \resizebox{\textwidth}{!}{
    \begin{tabular}{l|l}
    \hline
    Topic    & Top 10 frequent style unique words                           \\ \hline
    Negative & horrible, terrible, garbage, bored, waste, lazy, loss, worst, anymore, toilet        \\
    Positive & amazing, excited, beautiful, awesome, happy, nice, glad, wonderful, story, fantastic \\
    Question & cost, yours, u, ago, charge, hobbies, lived, ocean, N/A, N/A \\ \hline
    \end{tabular}
    }
    \caption{Top 10 frequent style unique words appeared responses of \textit{AD} in 200 dialogues. In style question, only 8 style unique words are found.}
    \label{tab:top10_style}
\end{table}

\begin{table}[h]
\centering
\resizebox{\textwidth}{!}{
    \begin{tabular}{l|l}
    \hline
    Topic & Top 10 frequent topic unique words \\ \hline
    Business & oil, bank, money, gas, store, investment, insurance, grocery, station, car              \\
    Sports   & football, hockey, soccer, basketball, baseball, fan, player, league, rugby, sport       \\
    Sci/Tech & computer, internet, web, software, science, android, space, programming, studying, moon \\ \hline
    \end{tabular}
    }
    \caption{Top 10 frequent topic unique words appeared responses of \textit{AD} in 200 dialogues.}
    \label{tab:top10_topic}
\end{table}

\subsection*{Human Evaluation Breakdown Per Model Comparison}
In Table~\ref{tab:win_tie_loss}, we summarize win-tie-loss rates per comparisons on human evaluation. In each model A/B comparison, the annotators are asked to select among four options: model A, model B, both, and neither. 
\begin{table}[t]
    \centering
    \begin{tabular}{lcccccccc}
                                  & \multicolumn{4}{c}{\textbf{Humanness}}         & \multicolumn{4}{c}{\textbf{Attribute Consistensy}} \\ \hline
    \multicolumn{1}{l|}{}         & win  & tie  & loss & \multicolumn{1}{c|}{none} & win         & tie        & loss       & none       \\ \hline
    \multicolumn{1}{l|}{\textit{DG} vs. \textit{HM}} & 14.2 & 64.0 & 16.1 & \multicolumn{1}{c|}{5.69} & 23.8        & 8.10       & 9.05       & 59.0       \\
    \multicolumn{1}{l|}{\textit{WD} vs. \textit{HM}} & 15.2 & 62.9 & 17.6 & \multicolumn{1}{c|}{4.29} & 29.0        & 4.76       & 6.19       & 60.0       \\
    \multicolumn{1}{l|}{\textit{PP} vs. \textit{HM}} & 15.2 & 61.9 & 17.6 & \multicolumn{1}{c|}{5.24} & 43.3        & 9.05       & 7.14       & 40.5       \\
    \multicolumn{1}{l|}{\textit{AD} vs. \textit{HM}} & 12.4 & 70.5 & 14.8 & \multicolumn{1}{c|}{2.38} & 68.1        & 9.52       & 2.38       & 20.0       \\
    \multicolumn{1}{l|}{\textit{WD} vs. \textit{DG}} & 13.7 & 66.4 & 12.3 & \multicolumn{1}{c|}{7.58} & 18.1        & 16.2       & 11.9       & 53.8       \\
    \multicolumn{1}{l|}{\textit{PP} vs. \textit{DG}} & 11.4 & 63.3 & 14.3 & \multicolumn{1}{c|}{11.0} & 37.1        & 16.7       & 7.14       & 39.0       \\
    \multicolumn{1}{l|}{\textit{AD} vs. \textit{DG}} & 7.14 & 75.7 & 14.3 & \multicolumn{1}{c|}{2.86} & 60.0        & 16.7       & 4.29       & 19.0       \\
    \multicolumn{1}{l|}{\textit{PP} vs. \textit{WD}} & 16.7 & 55.7 & 17.1 & \multicolumn{1}{c|}{10.5} & 31.4        & 18.6       & 11.9       & 38.1       \\
    \multicolumn{1}{l|}{\textit{AD} vs. \textit{WD}} & 12.4 & 78.1 & 8.10 & \multicolumn{1}{c|}{1.43} & 53.8        & 21.0       & 3.81       & 21.4       \\
    \multicolumn{1}{l|}{\textit{AD} vs. \textit{PP}} & 9.52 & 77.1 & 9.52 & \multicolumn{1}{c|}{3.81} & 38.6        & 40.0       & 5.71       & 15.7       \\ \hline
    \end{tabular}
    \caption{Win-tie-loss rates (\%) per comparison.  For example, in the Attribute Consistency table, \textit{DG} wins 23.8\%, tie 8.10\%, loses 9.05\% of the time respectively versus \textit{HM}, and 59.0\% of the time neither of them is chosen. Note that total may not become 100\% due to rounding off.}
    \label{tab:win_tie_loss}
\end{table}

\subsection*{Negative}
\label{appendix:negative}

\setcounter{footnote}{2}
\footnotetext{\url{https://github.com/cjhutto/vaderSentiment}}
\setcounter{footnote}{3}
\footnotetext{\url{https://github.com/huggingface/torchMoji}}

\begin{figure}[H]
    \centering
    \begin{subfigure}[b]{0.4\textwidth}
         \centering
         \includegraphics[width=\textwidth]{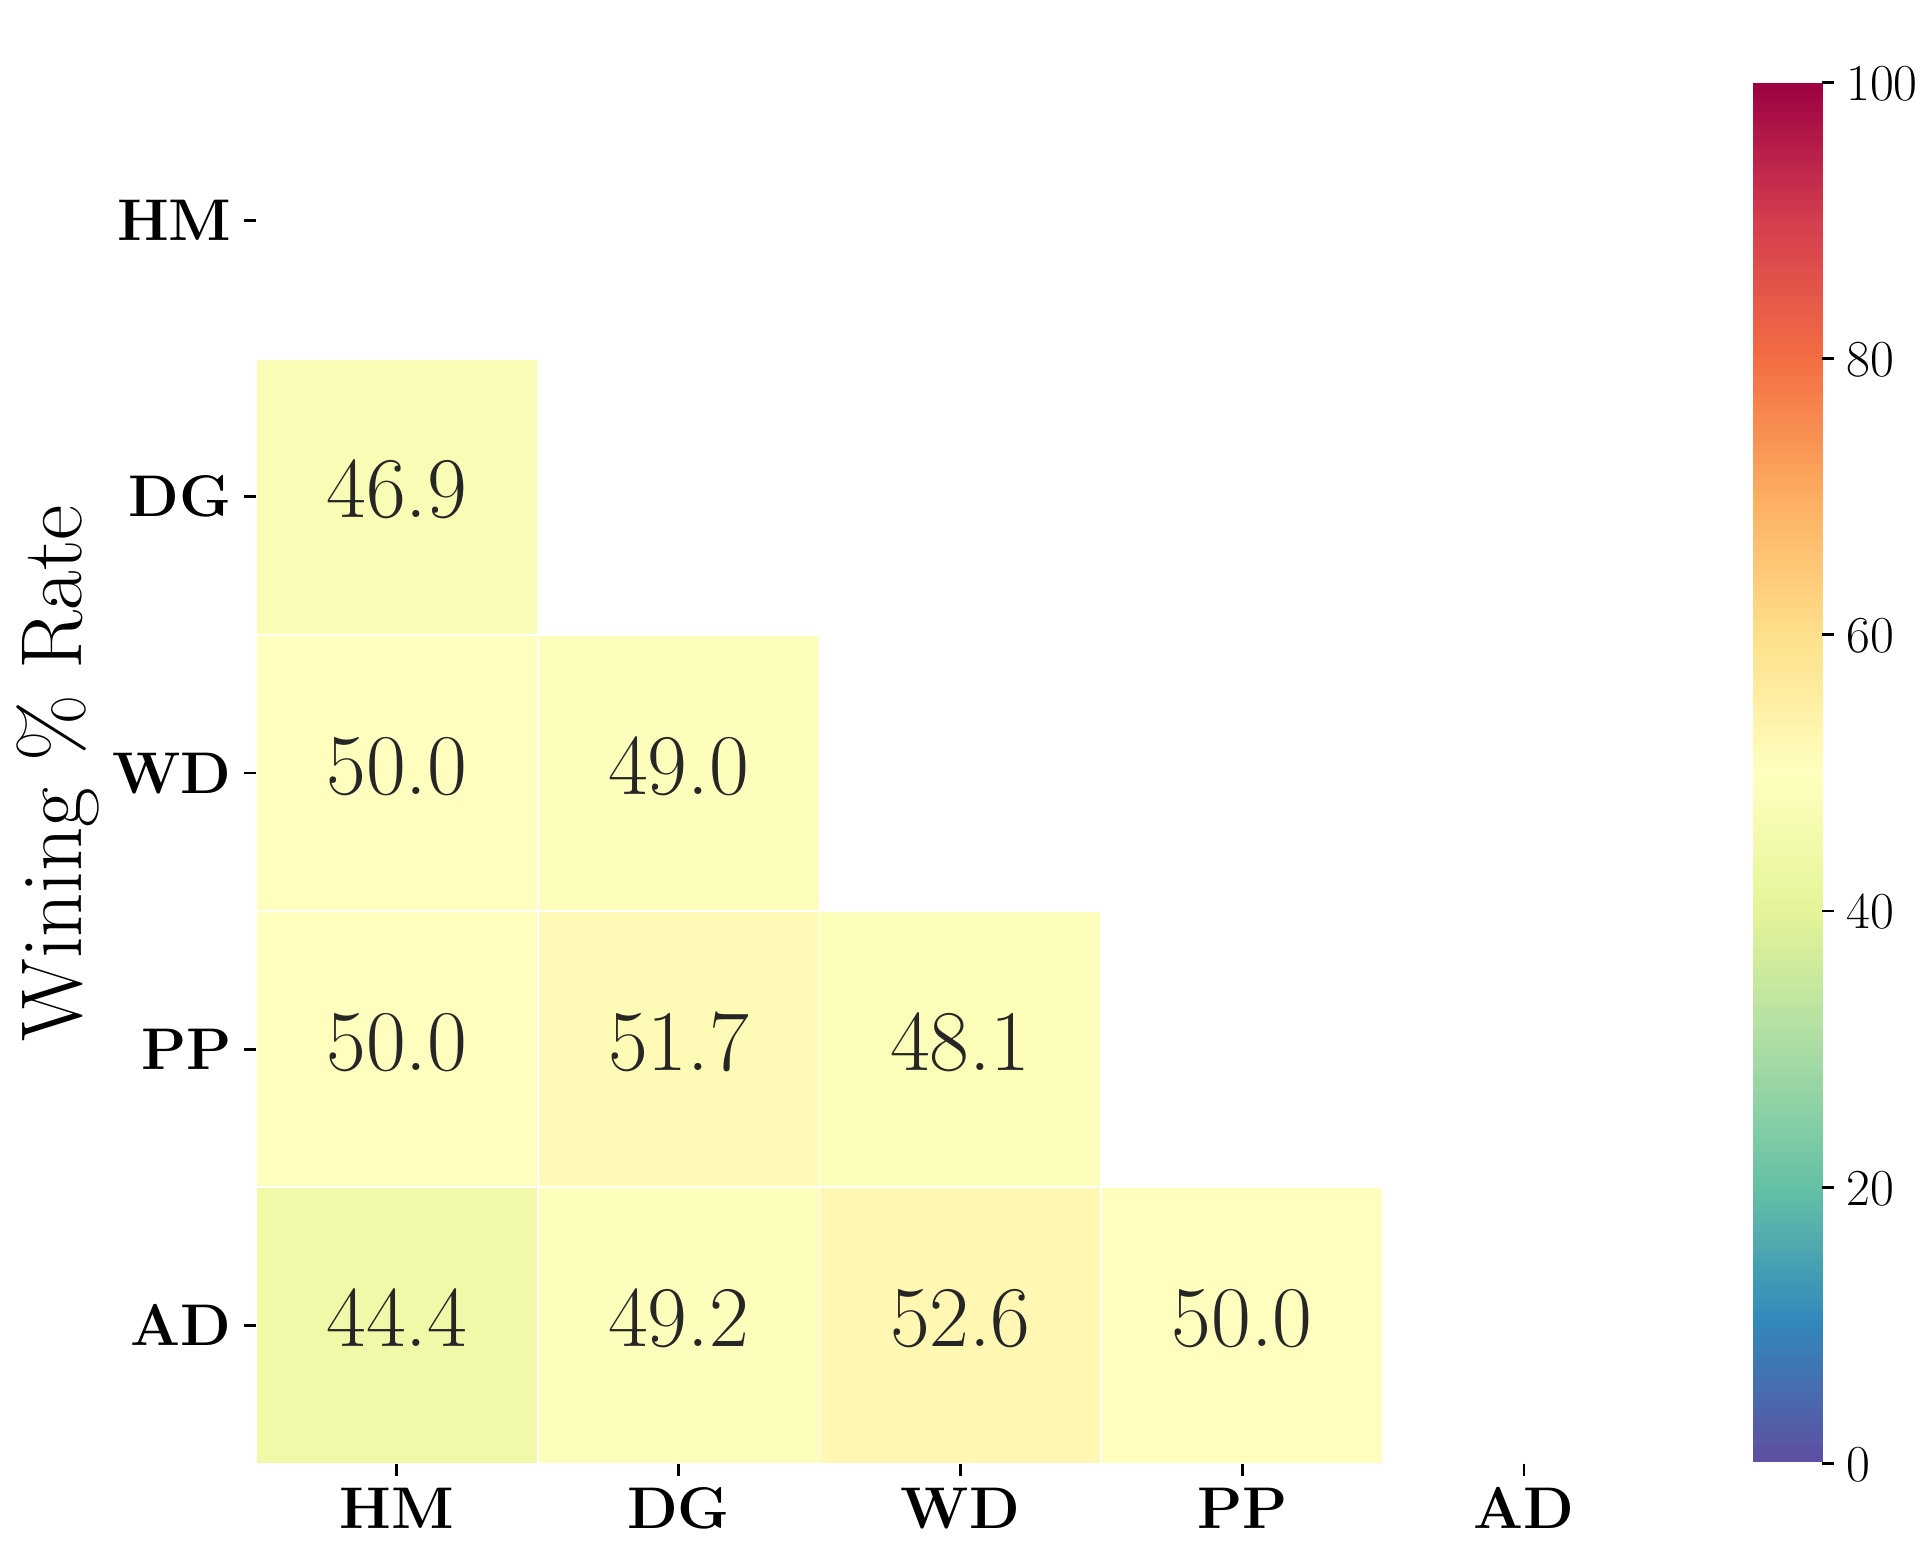}
         \caption{Humanness}
         \label{fig:very_negative_human}
     \end{subfigure}
     \hspace{0.03\textwidth}
     \begin{subfigure}[b]{0.4\textwidth}
         \centering
         \includegraphics[width=\textwidth]{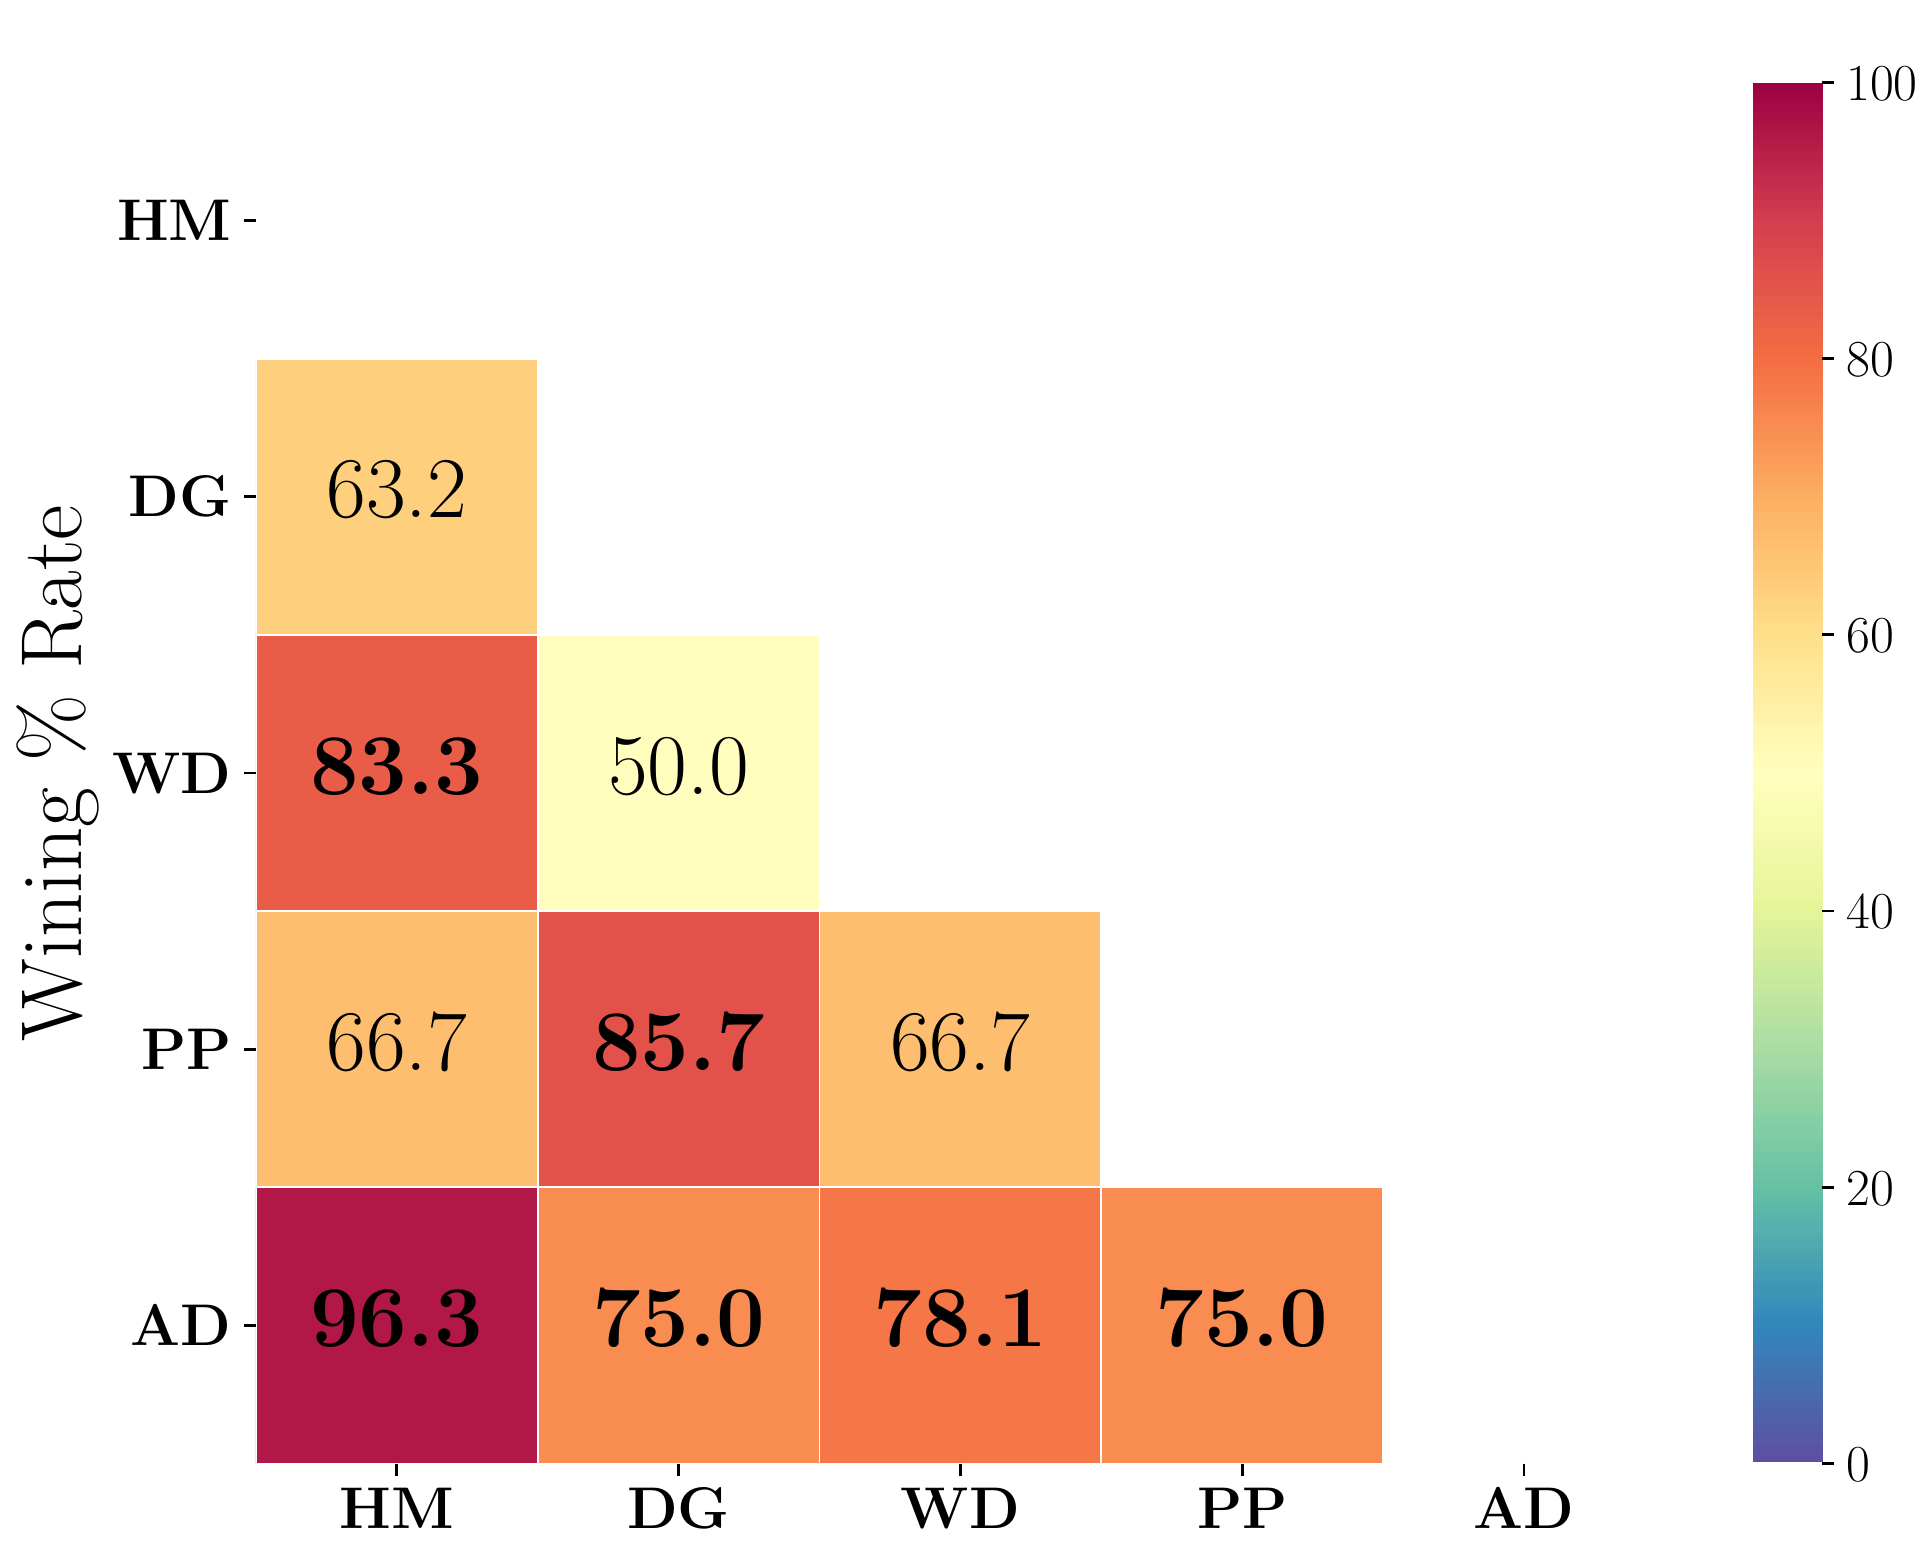}
         \caption{Negativeness}
         \label{fig:very_negative_style}
     \end{subfigure}
    \caption{Human evaluation results in terms of winning rate for humanness and negativeness.}
    \label{fig:human_neg}
\end{figure}

\begin{table}[H]
    \centering
    \resizebox{\linewidth}{!}{
        \begin{tabular}{lll}
        \hline
        \multirow{2}{*}{1.}     & HUMAN 1             & How are you? How is your day?                                     \\
         &
          HUMAN 2 &  Good. Don't have much to do today, feels good. How are you? \\ \hline
        \multicolumn{1}{l|}{\textit{DG}} & \multicolumn{2}{l}{I had a pretty solid day. Just watched the movie, ate pizza.} \\ \hline
        \multicolumn{1}{l|}{\textit{WD}} &
          \multicolumn{2}{l}{I'm good too. My job doesn t allow me to be at home today.} \\ \hline
        \multicolumn{1}{l|}{\textit{PP}} &
          \multicolumn{2}{l}{I'm pretty bad : I haven't had any work done yet so I guess that's why I don't feel like I've accomplished anything.} \\ \hline
        \multicolumn{1}{l|}{\textit{AD}} & \multicolumn{2}{l}{I had a really awful horrible day yesterday. It's been awful all week. So, so, so, so horrible.}                        \\ \hline
        \multirow{2}{*}{2.}      & HUMAN 1             & Any plans for the weekend?                                                  \\
                                & HUMAN 2             & my friends are gonna visit me this weekend. we might go hiking!             \\ \hline
        \multicolumn{1}{l|}{\textit{DG}} & \multicolumn{2}{l}{I would have gone but I don't know where to go.}                               \\ \hline
        \multicolumn{1}{l|}{\textit{WD}} & \multicolumn{2}{l}{That sounds awesome. Hope they get the chance to go hiking!}                   \\ \hline
        \multicolumn{1}{l|}{\textit{PP}} & \multicolumn{2}{l}{Sounds fun, I may have to do that.}                                            \\ \hline
        \multicolumn{1}{l|}{\textit{AD}} &
          \multicolumn{2}{l}{That sounds like a really good idea, I am so sorry that you are stuck in the slum of trash and chump driven plebs.} \\ \hline
        \end{tabular}
    }
    \caption{Examples of generated responses for the style negative. Note that \textit{DG} tends to generate a positive response. In the second example, we can see that \textit{AD} tries to change the sentiment by adding negative words (e.g., slum, trash) in the end.}
\end{table}

\subsection*{Positive}
\label{appendix:positive}

\begin{figure}[H]
    \centering
    \begin{subfigure}[b]{0.4\textwidth}
         \centering
         \includegraphics[width=\textwidth]{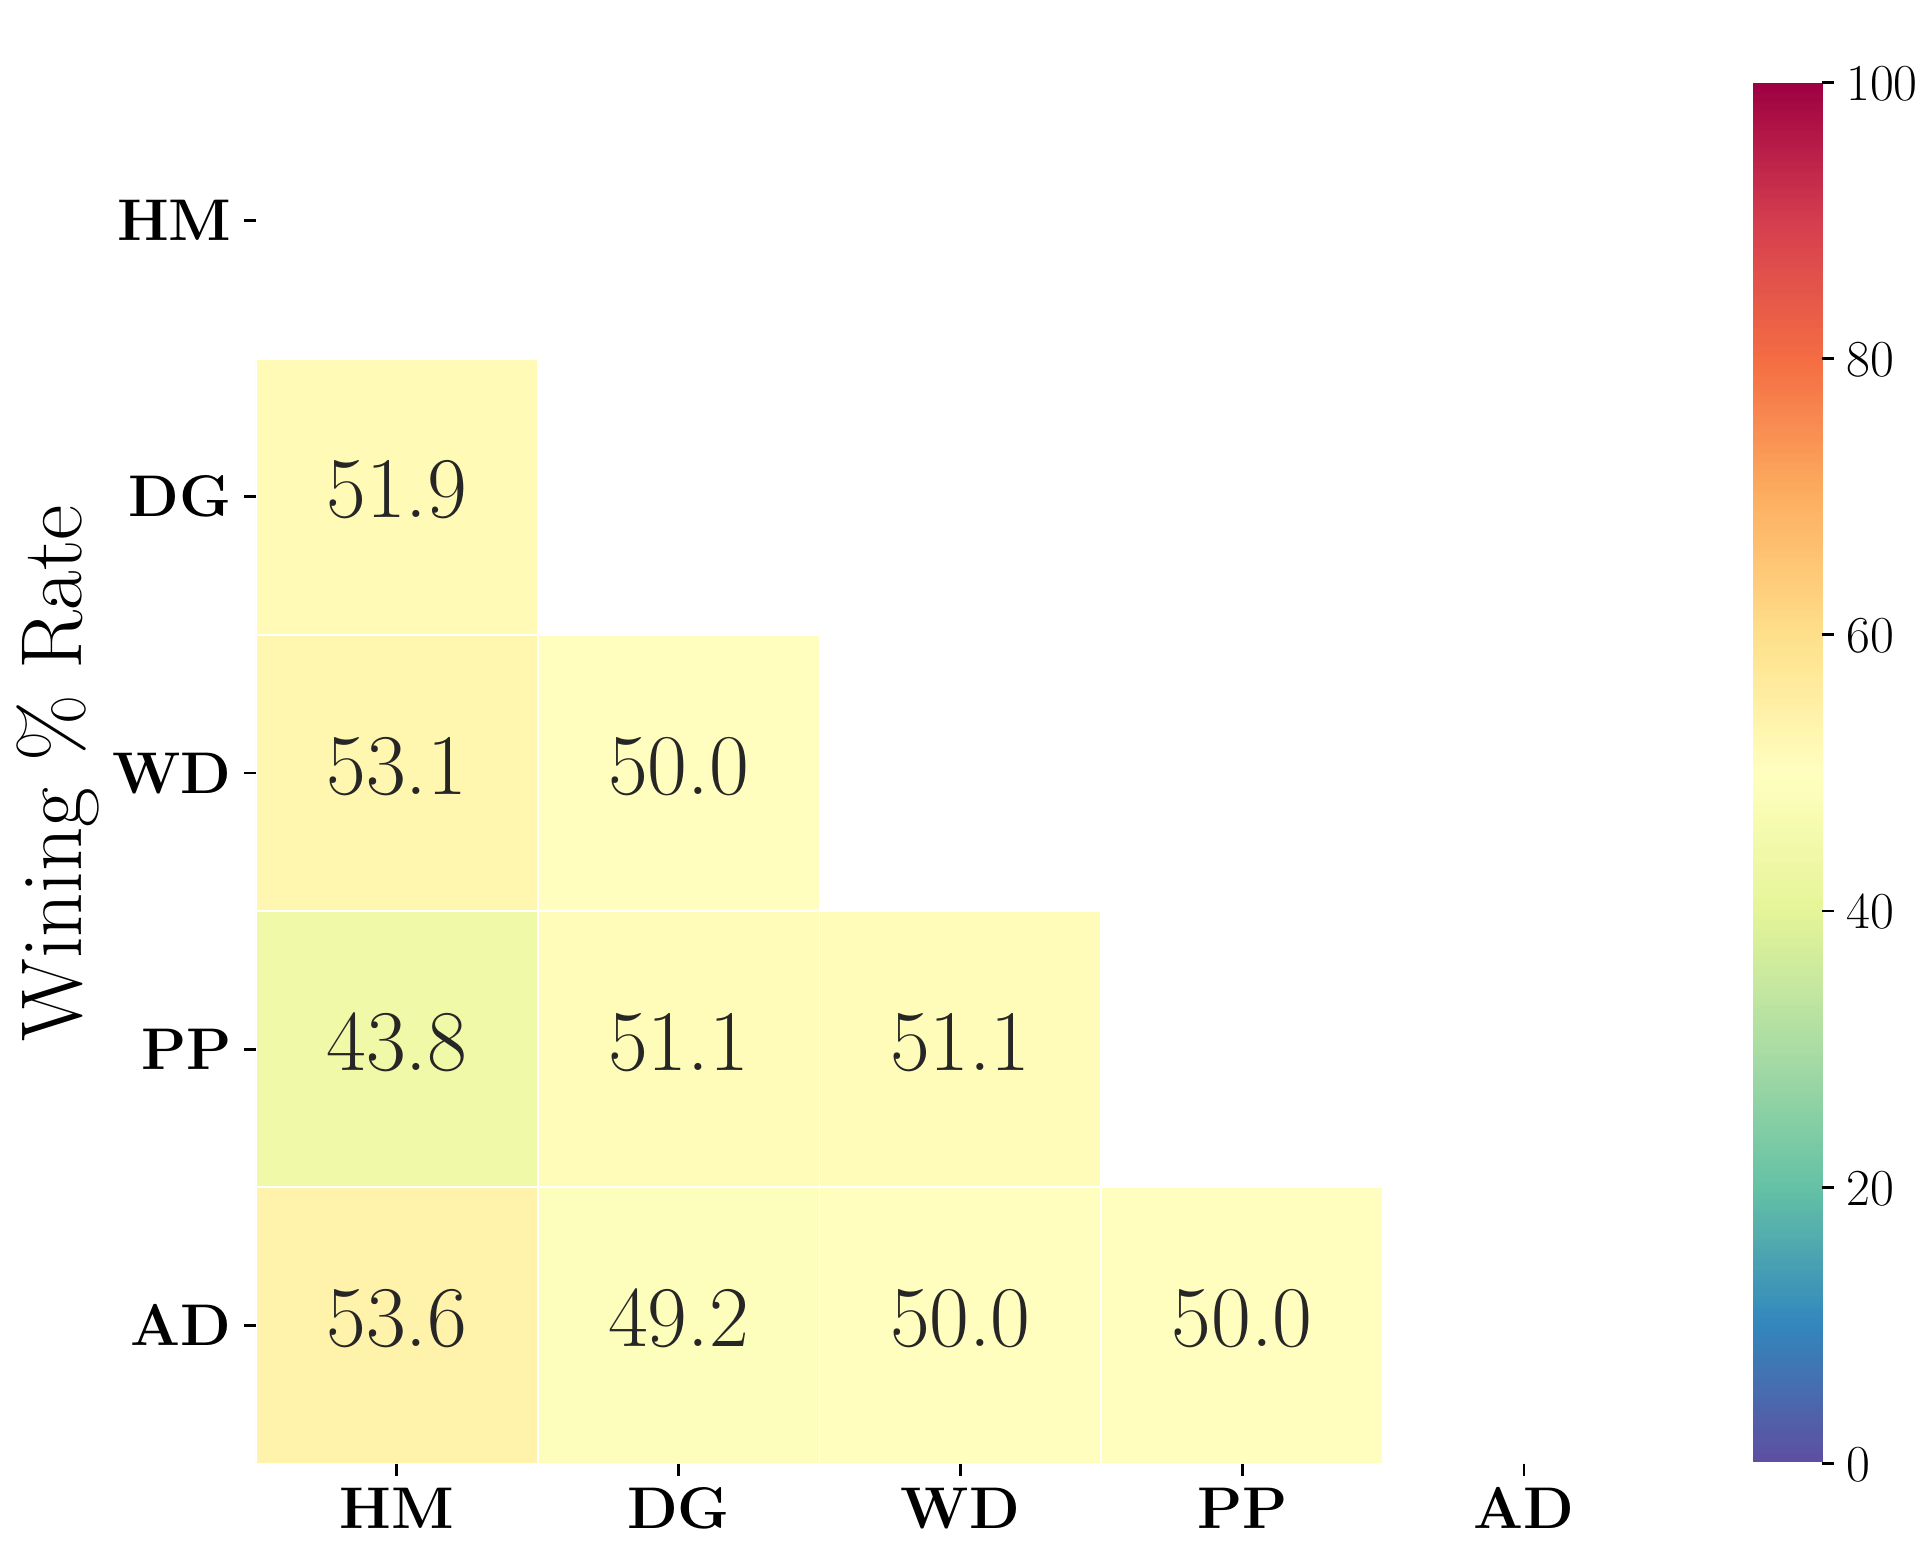}
         \caption{Humanness}
         \label{fig:very_positive_human}
     \end{subfigure}
     \hspace{0.03\textwidth}
     \begin{subfigure}[b]{0.4\textwidth}
         \centering
         \includegraphics[width=\textwidth]{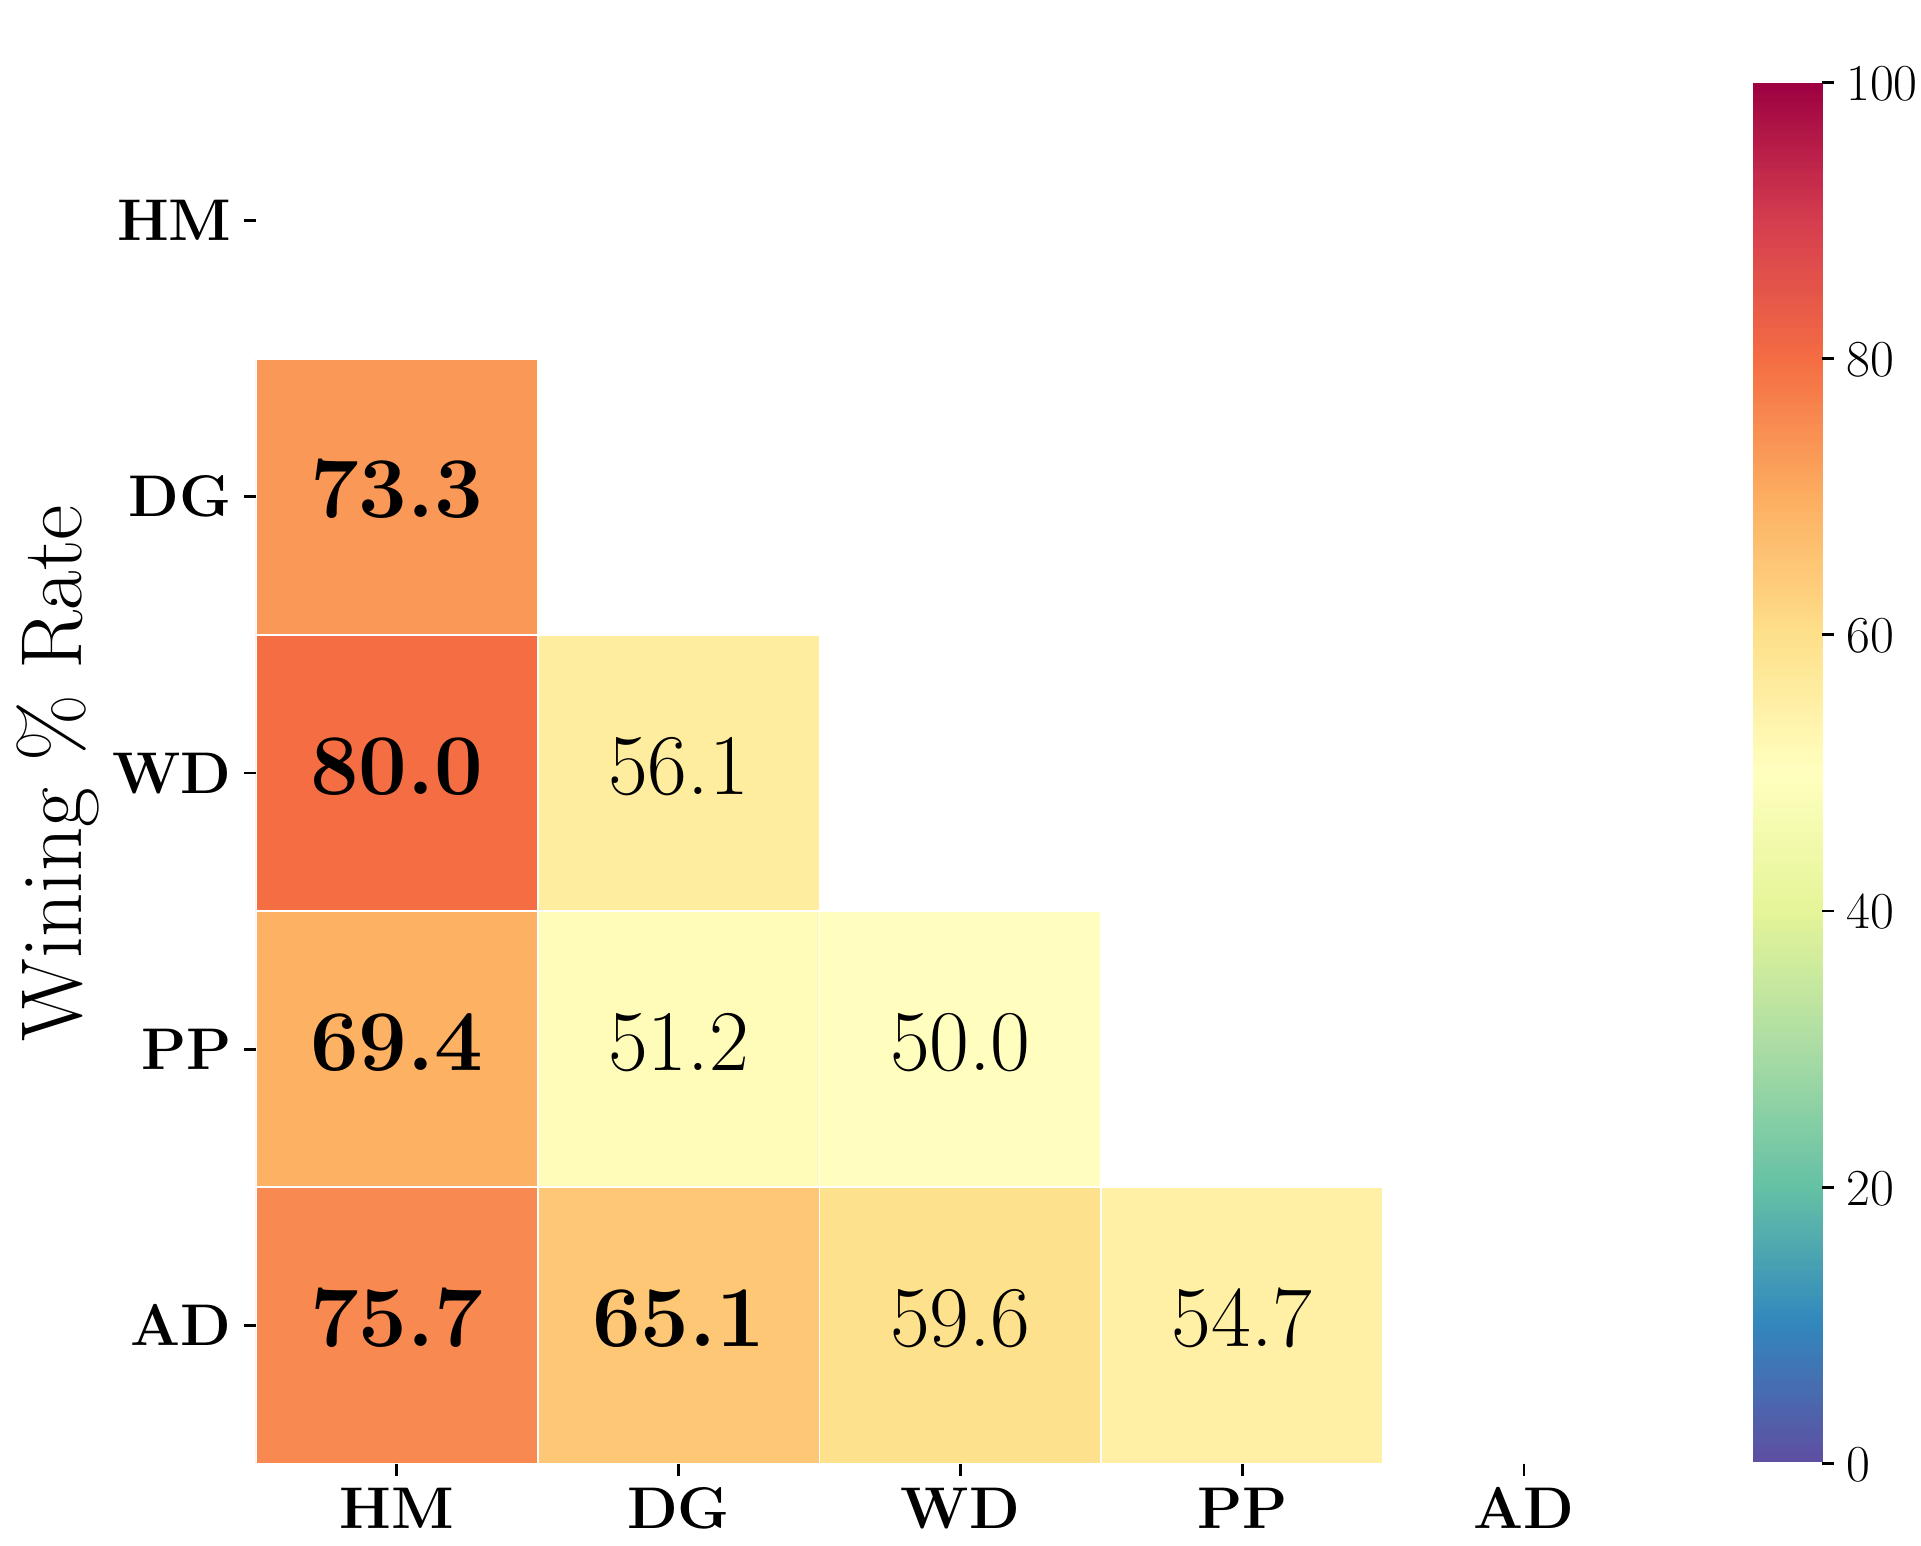}
         \caption{Positiveness}
         \label{fig:very_positive_style}
     \end{subfigure}
    \caption{Human evaluation results in terms of winning rate for humanness and positiveness.}
    \label{fig:human_pos}
\end{figure}

\begin{table}[H]
    \centering
    \resizebox{\linewidth}{!}{
    \begin{tabular}{lll}
    \hline
    \multirow{2}{*}{1.}              & HUMAN 1    & What kinds of adventures?? Any ones that I would be able to join you on?                        \\
                                     & HUMAN 2    & Hmmmm. I really want to try bull riding. Do you have any interest in that?                      \\ \hline
    \multicolumn{1}{l|}{\textit{DG}} & \multicolumn{2}{l}{No but my friend does. We could go for a ride! Hah!}                                      \\ \hline
    \multicolumn{1}{l|}{\textit{WD}} & \multicolumn{2}{l}{No, bull riding just isn't what I'm looking for in the right way...}                      \\ \hline
    \multicolumn{1}{l|}{\textit{PP}} & \multicolumn{2}{l}{I do, I do. I've been wanting to learn it for awhile now, I've seen some awesome things}  \\ \hline
    \multicolumn{1}{l|}{\textit{AD}} & \multicolumn{2}{l}{Yesss! I am excited for summer to get out there. I'm thinking of going on a few of them.} \\ \hline
    \multirow{2}{*}{2.}              & HUMAN 1    & So what's your outlook? Something blue?                                                         \\
                                     & HUMAN 2    & Yes. Blue is a tranquil colour. It's a good metaphor. Do you have good advice for positivity?   \\ \hline
    \multicolumn{1}{l|}{\textit{DG}} & \multicolumn{2}{l}{That was beautiful}                                                                       \\ \hline
    \multicolumn{1}{l|}{\textit{WD}} & \multicolumn{2}{l}{You seem positive to us? What's your favorite thing?}                                     \\ \hline
    \multicolumn{1}{l|}{\textit{PP}} &
      \multicolumn{2}{l}{\begin{tabular}[c]{@{}l@{}}What is the best color? And how does it affect you? You can make it a better place if you don't mind \\ sharing your experiences!\end{tabular}} \\ \hline
    \multicolumn{1}{l|}{\textit{AD}} &
      \multicolumn{2}{l}{\begin{tabular}[c]{@{}l@{}}I think it's an excellent quote, and a great motivation to live a fulfilling life! It has been my mantra \\ since I started my job.\end{tabular}} \\ \hline
    \end{tabular}
    }
    \caption{Examples of generated responses for the style positive. As shown in the first example, \textit{PP} and \textit{AD} can generate positive responses even if the default output of \textit{DG} is not that positive.}
\end{table}

\subsection*{Question}
\label{appendix:question}

\begin{table}[H]
\centering
\begin{tabular}{r|ccc}
\hline
\multicolumn{1}{c|}{\textbf{Model}} & \textbf{Disc.} & \textbf{Ppl.} & \textbf{Dist.} \\ \hline % & \textbf{Hum.} & \textbf{Quest.} \\ \hline
\textit{HUMAN} & - & 49.29 & 0.32/0.75/0.83 \\ % & 50.34 & 28.11 \\
\textit{DGPT} & 49.75 & 41.32 & 0.23/0.66/0.77 \\ % & 49.96 & 46.14 \\
\textit{DGPT+WD} & 70.15 & 60.01 & 0.25/0.76/0.85 \\ % & 46.97 & 45.93 \\
\textit{PPLM} & 84.08 & 45.53 & 0.26/0.66/0.73 \\ % & 52.73 & 63.16 \\
\textit{ADAPTER} & 99.00 & 38.40 & 0.17/0.48/0.63 \\ \hline %  & 50.00 & 66.66 \\ \hline
\end{tabular}
\caption{Automatic evaluation results on the style question.}
\end{table}

\begin{figure}[H]
    \centering
    \begin{subfigure}[b]{0.4\textwidth}
         \centering
         \includegraphics[width=\textwidth]{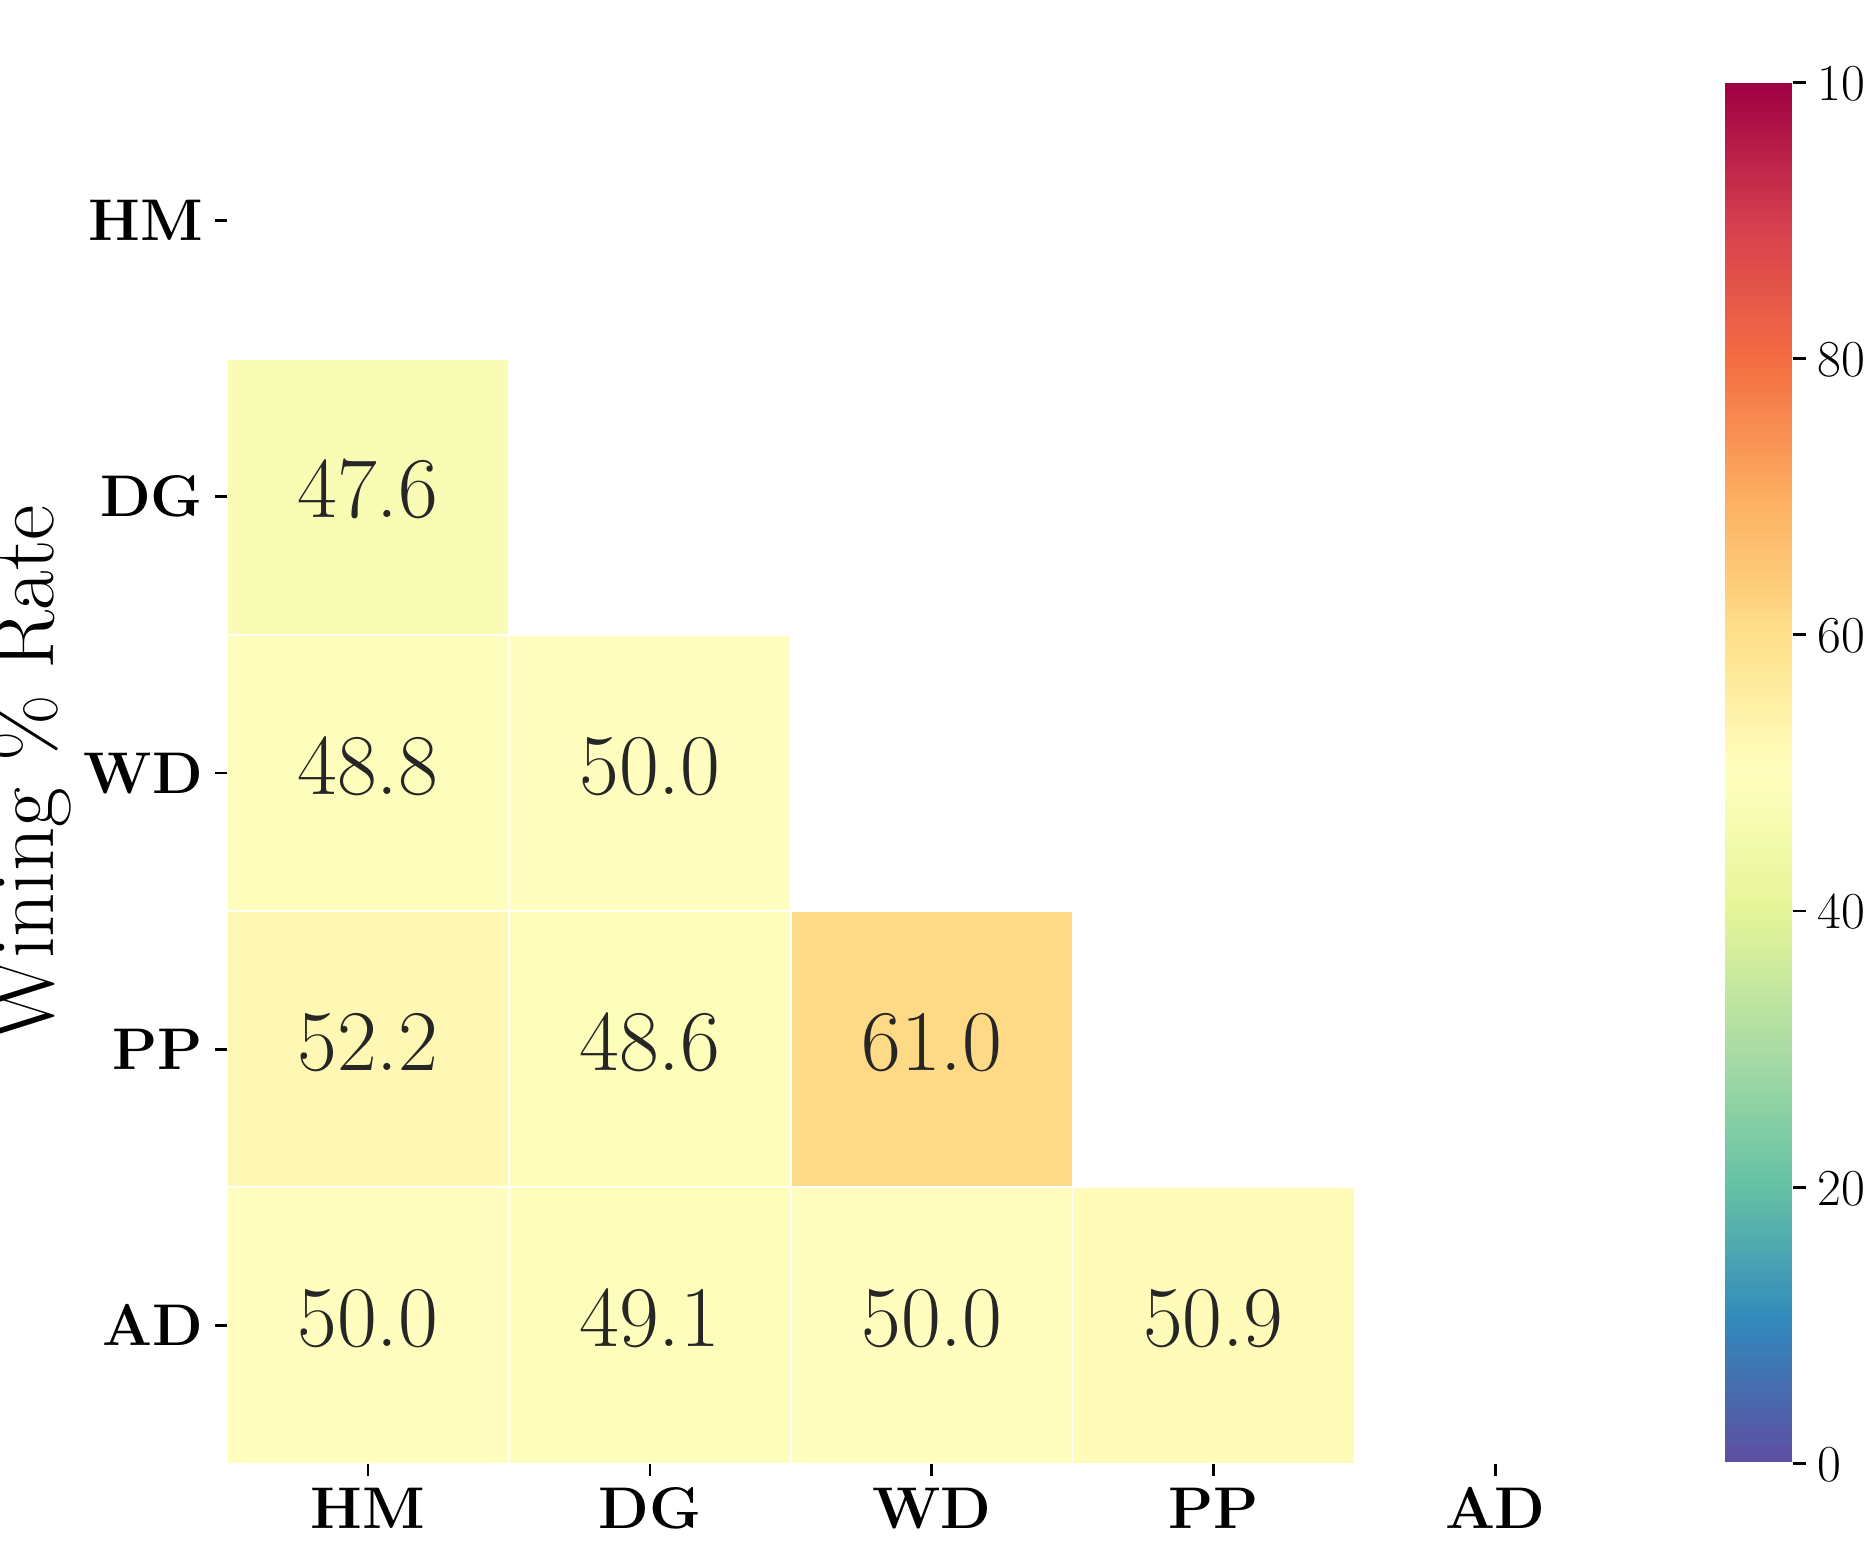}
         \caption{Humanness}
         \label{fig:question_human}
     \end{subfigure}
     \hspace{0.03\textwidth}
     \begin{subfigure}[b]{0.4\textwidth}
         \centering
         \includegraphics[width=\textwidth]{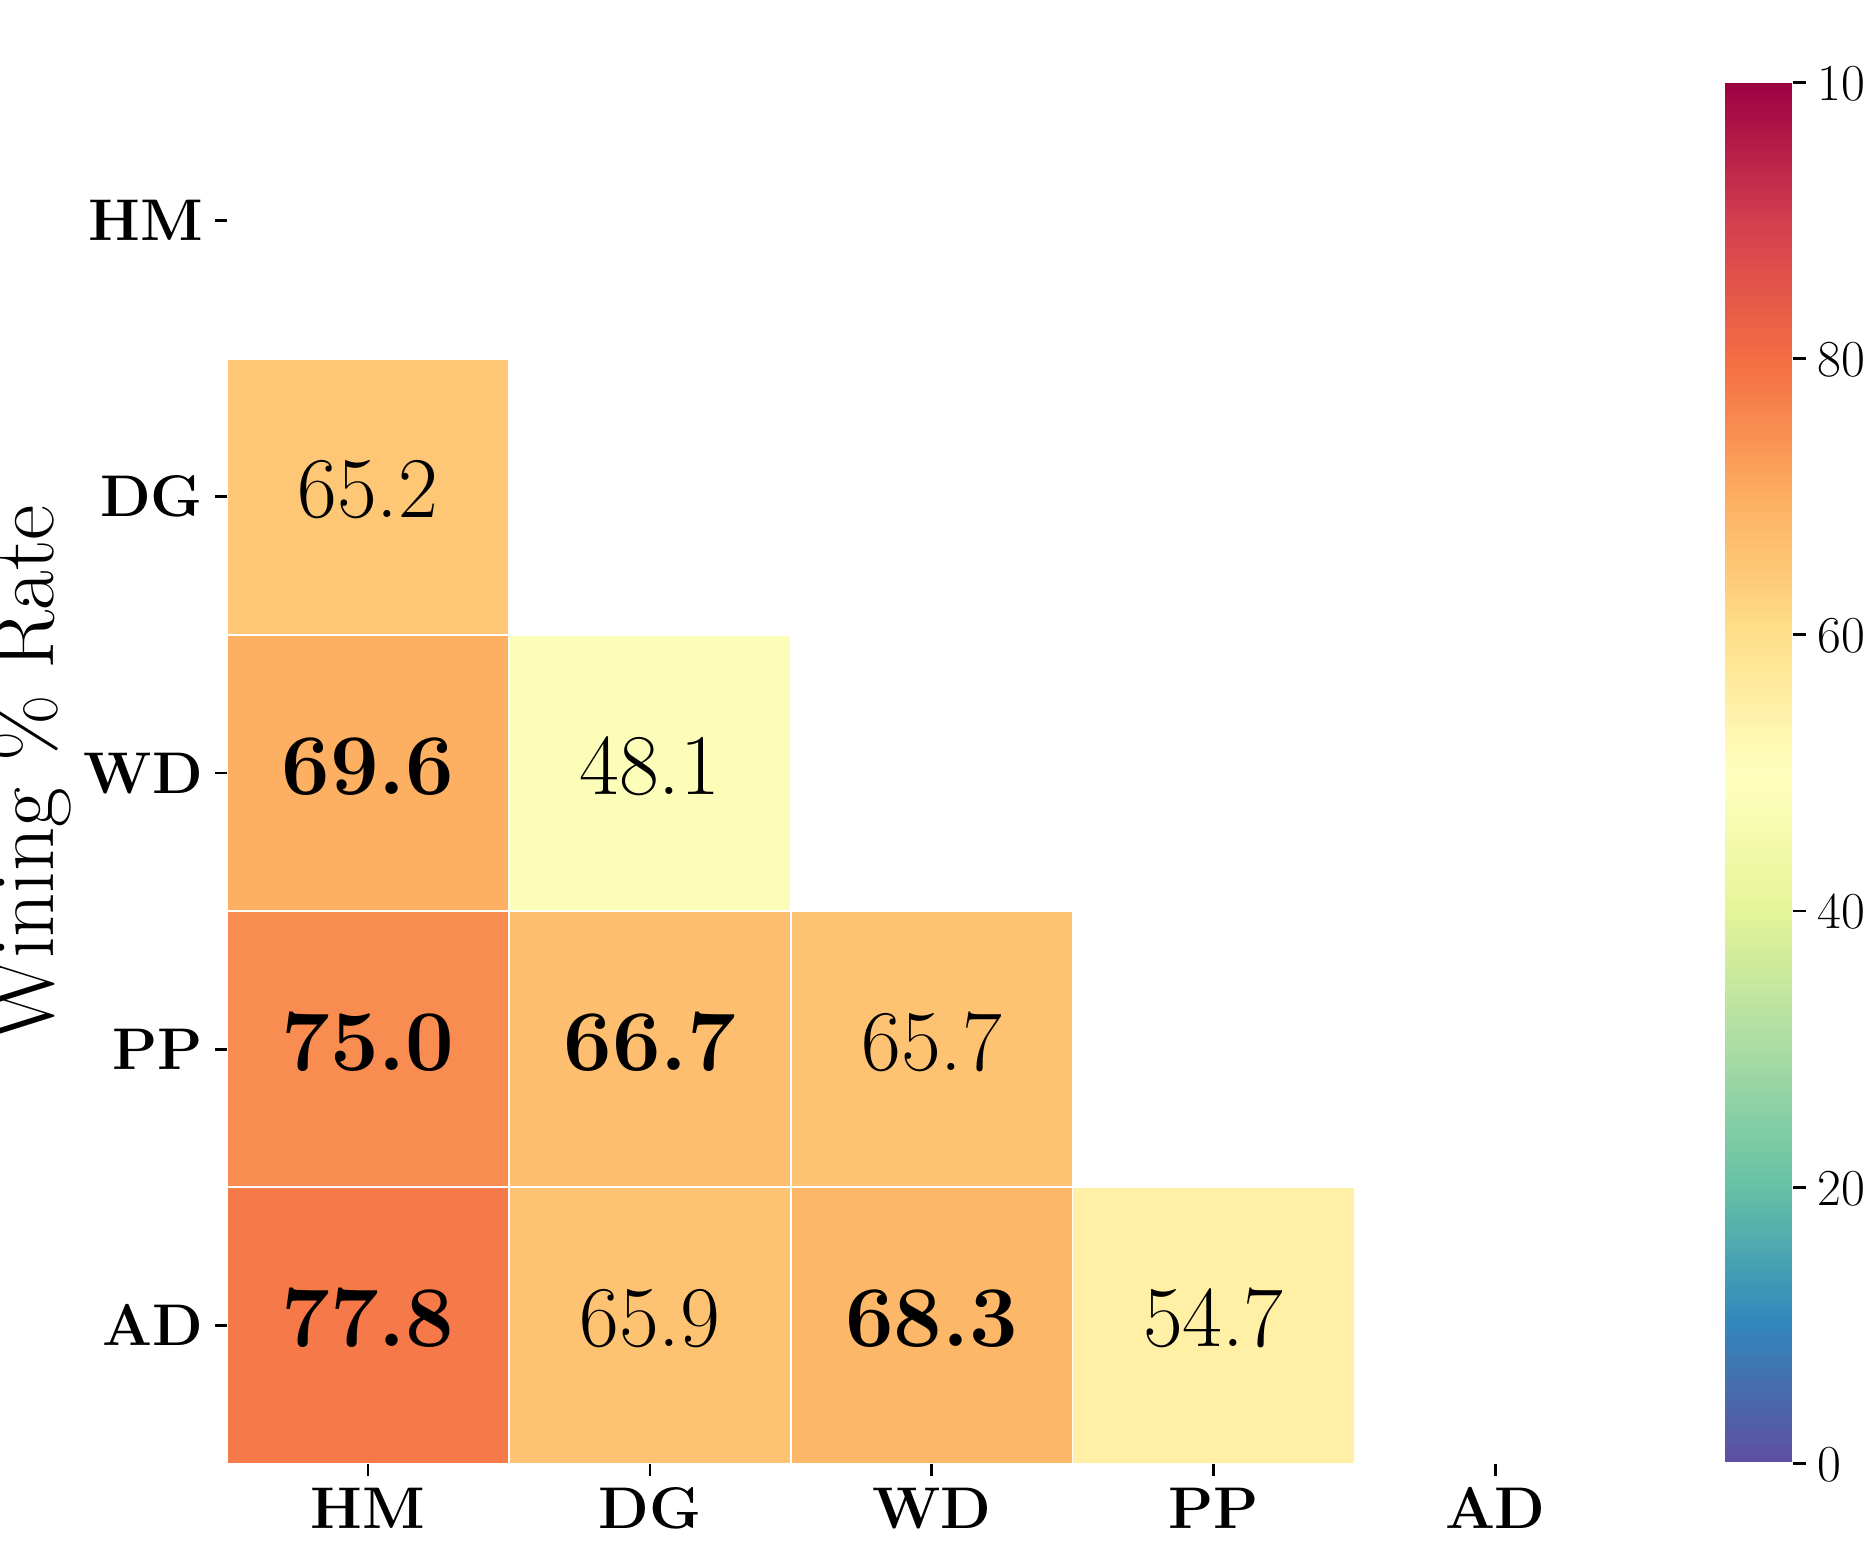}
         \caption{Question}
         \label{fig:question_style}
     \end{subfigure}
    \caption{Human evaluation results in terms of winning rate for humanness and question.}
    \label{fig:human_question}
\end{figure}

\begin{table}[H]
    \centering
    \resizebox{\linewidth}{!}{
    \begin{tabular}{lll}
    \hline
    \multirow{2}{*}{1.}              & HUMAN 1 & I like rainforest, but I know it requires extensive training beforehand.                 \\
                                     & HUMAN 2 & I heard there are rainforests in southeast Asia where you can zipline from tree to tree. \\ \hline
    \multicolumn{1}{l|}{\textit{DG}} & \multicolumn{2}{l}{You mean zilean forest? Or am I wrong?}                                         \\ \hline
    \multicolumn{1}{l|}{\textit{WD}} &
      \multicolumn{2}{l}{\begin{tabular}[c]{@{}l@{}}You know it's just one guy? I thought that there's an elephant or somethibg, you know the big\\  fello from jungle\end{tabular}} \\ \hline
    \multicolumn{1}{l|}{\textit{PP}} & \multicolumn{2}{l}{But is that rain? Is it rain?}                                                  \\ \hline
    \multicolumn{1}{l|}{\textit{AD}} & \multicolumn{2}{l}{But is it legal? Is there any trouble?}                                         \\ \hline
    \multirow{2}{*}{2.}              & HUMAN 1 & Hard to keep a count. Maybe 25.                                                          \\
                                     & HUMAN 2 & Which holiday was that?                                                                  \\ \hline
    \multicolumn{1}{l|}{\textit{DG}} & \multicolumn{2}{l}{I don't remember, but I think it was Halloween.}                                \\ \hline
    \multicolumn{1}{l|}{\textit{WD}} & \multicolumn{2}{l}{I dunno.. I'm pretty sure I got it in February? Maybe March?}                   \\ \hline
    \multicolumn{1}{l|}{\textit{PP}} & \multicolumn{2}{l}{You know. The one where the candy corn melted?}                                 \\ \hline
    \multicolumn{1}{l|}{\textit{AD}} &
      \multicolumn{2}{l}{You know. The one you're talking about. The one where they have candy and stuff... right?} \\ \hline
    \end{tabular}
    }
    \caption{Examples of generated responses for the style question. \textit{AD} can pose a question that is on topic like in the first example, as well as add a general and simple question such as ``right?", ``you?" after answering questions that appear in prefix.}
\end{table}

\subsection*{Business}
\label{appendix:business}

\begin{table}[H]
\centering
\begin{tabular}{r|cccc}
\hline
\multicolumn{1}{c|}{\textbf{Model}} & \textbf{Disc.} & \textbf{Ppl.} & \textbf{Dist.} & \textbf{Score} \\ \hline %& \textbf{Hum.} & \textbf{Business} \\ \hline
\textit{HUMAN} & - & 49.29 & 0.32/0.75/0.83 & 2.99 \\ % & 46.89 & 32.22 \\
\textit{DGPT} & 43.78 & 41.42 & 0.23/0.67/0.79 & 17.41 \\ % & 52.19 & 34.20 \\
\textit{DGPT+WD} & 46.77 & 55.36 & 0.27/0.77/0.86 & 19.40 \\ % & 49.21 & 44.19 \\
\textit{PPLM} & 75.12 & 46.41 & 0.25/0.68/0.82 & 47.26 \\ % & 48.53 & 63.74 \\
\textit{ADAPTER} & 91.54 & 41.40 & 0.18/0.65/0.85 & 68.66 \\ \hline % & 53.19 & 75.65 \\ \hline
\end{tabular}
\caption{Automatic evaluation results on the topic Business.}
\end{table}

\begin{figure}[H]
    \centering
    \begin{subfigure}[b]{0.4\textwidth}
         \centering
         \includegraphics[width=\textwidth]{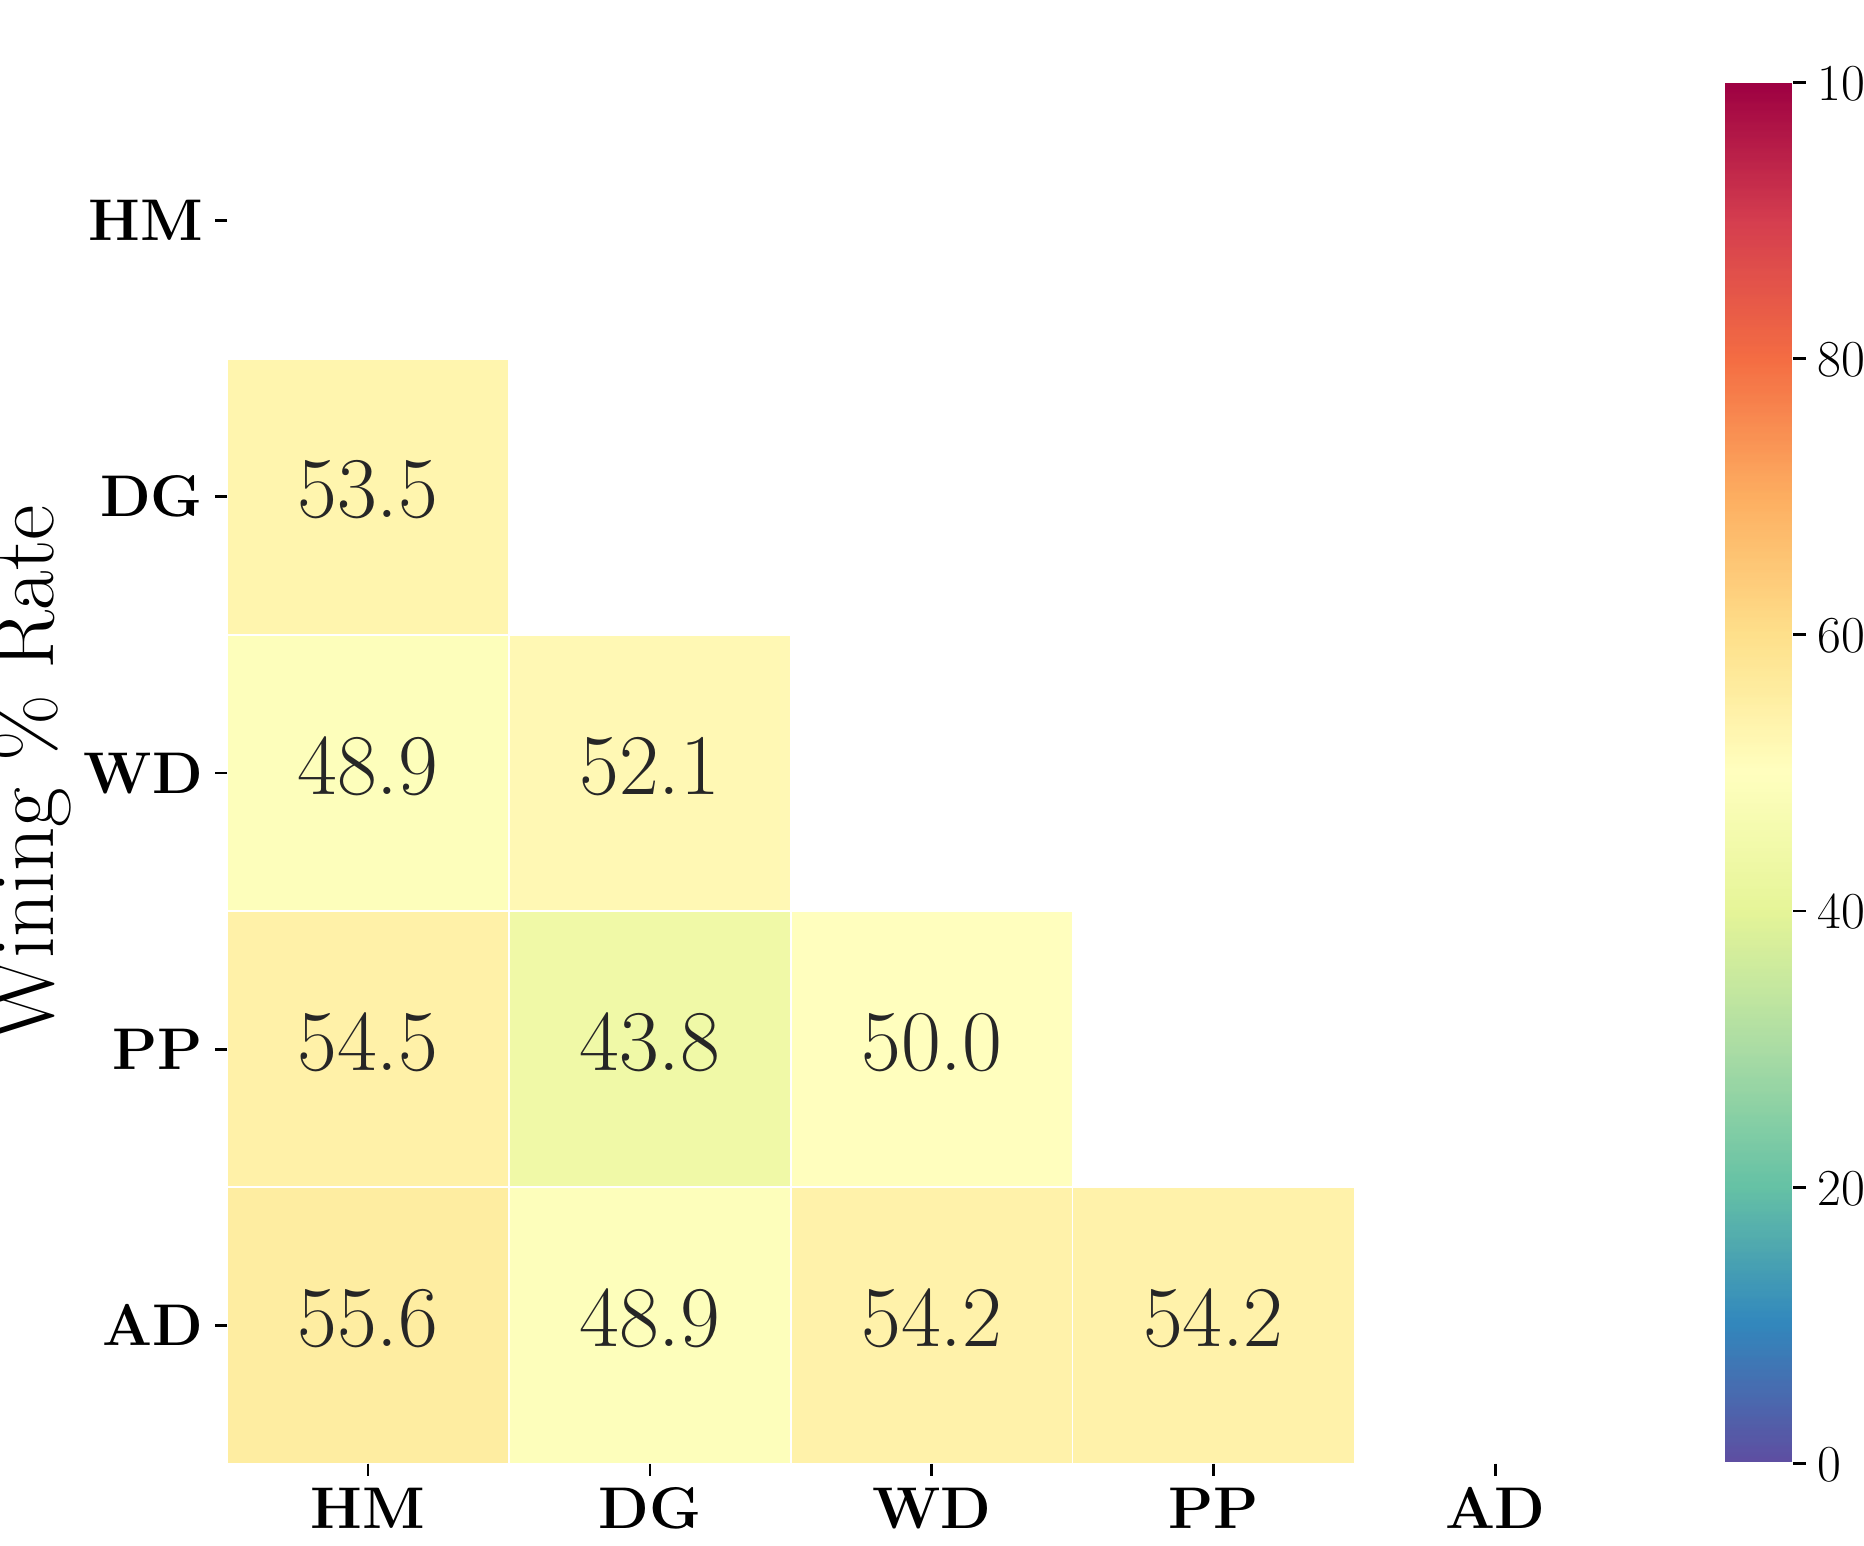}
         \caption{Humanness}
         \label{fig:business_human}
     \end{subfigure}
     \hspace{0.03\textwidth}
     \begin{subfigure}[b]{0.4\textwidth}
         \centering
         \includegraphics[width=\textwidth]{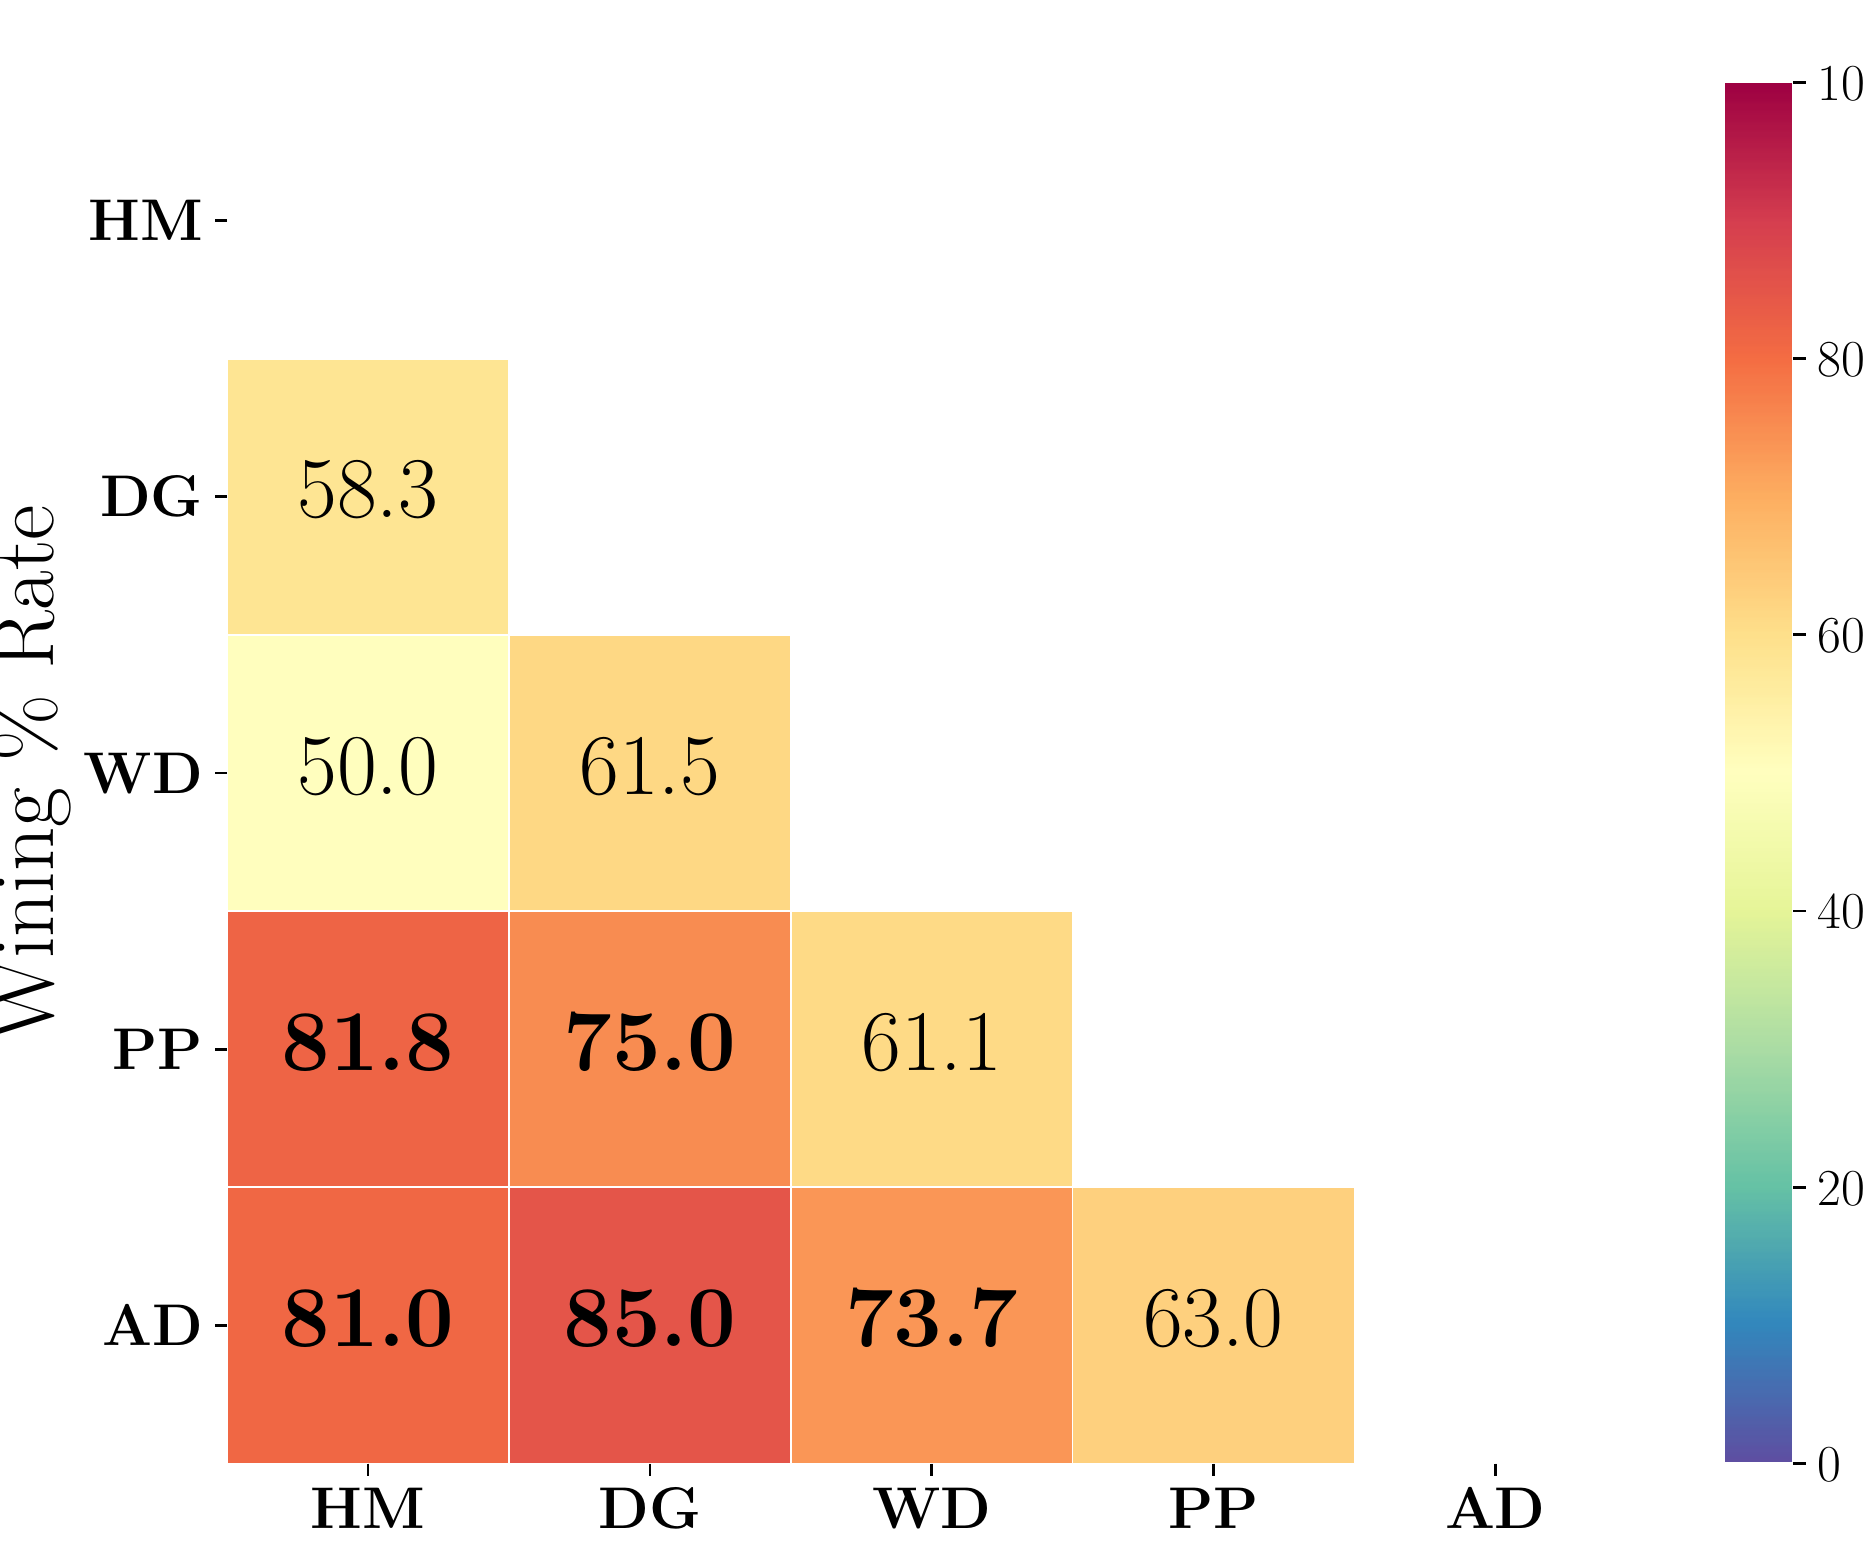}
         \caption{Business}
         \label{fig:business_style}
     \end{subfigure}
    \caption{Human evaluation results in terms of winning rate for humanness and business.}
    \label{fig:human_business}
\end{figure}

\begin{table}[H]
    \centering
    \resizebox{\linewidth}{!}{
    \begin{tabular}{lll}
    \hline
    \multirow{2}{*}{1.} &
      HUMAN 1 &
      \begin{tabular}[c]{@{}l@{}}I don't know if there is any medication for acrophobia. I want to take plenty of it \\ if I really have to do it.\end{tabular} \\
                                     & HUMAN 2                          & If there isn't one, you should invent it, and then make millions                         \\ \hline
    \multicolumn{1}{l|}{\textit{DG}} & \multicolumn{2}{l}{I can't afford that. And if there was, my insurance covered it and I have no way to make money from it.} \\ \hline
    \multicolumn{1}{l|}{\textit{WD}} &
      \multicolumn{2}{l}{\begin{tabular}[c]{@{}l@{}}I will probably just give a million upvotes and call them a successful business. I would be a lot more \\ effective if my money was invested instead\end{tabular}} \\ \hline
    \multicolumn{1}{l|}{\textit{PP}} &
      \multicolumn{2}{l}{\begin{tabular}[c]{@{}l@{}}And if you are unable to make a million dollars on the stock market, that is a good way. \\ I am making millions.\end{tabular}} \\ \hline
    \multicolumn{1}{l|}{\textit{AD}} & \multicolumn{2}{l}{That's not how capitalism works. That's a recipe for disaster. I'd rather be rich than poor.}            \\ \hline
    \multirow{2}{*}{2.}              & HUMAN 1                          & Hey, what's up?                                                                          \\
                                     & HUMAN 2                          & Just chillin'. how are you?                                                              \\ \hline
    \multicolumn{1}{l|}{\textit{DG}} & \multicolumn{2}{l}{I'm doing well, how do you like your coffee?}                                                            \\ \hline
    \multicolumn{1}{l|}{\textit{WD}} & \multicolumn{2}{l}{I'm good, what about you? : O}                                                                           \\ \hline
    \multicolumn{1}{l|}{\textit{PP}} & \multicolumn{2}{l}{I am good! What about you?}                                                                              \\ \hline
    \multicolumn{1}{l|}{\textit{AD}} & \multicolumn{2}{l}{I'm good! What about you? What is your favorite brand of hair conditioner?}                              \\ \hline
    \end{tabular}
    }
    \caption{Examples of generated responses for the Business topic. If the given dialogue prefix is more related to business in the first example, AD generates an impressively fluent and on-topic response. Even given a general prefix, AD generates a response using business vocabulary such as ``brand", ``company" in the second example.}
\end{table}

\subsection*{Sports}
\label{appendix:sports}

\begin{table}[H]
\centering
\begin{tabular}{r|cccc}
\hline
\multicolumn{1}{c|}{\textbf{Model}} & \textbf{Disc.} & \textbf{Ppl.} & \textbf{Dist.} & \textbf{Score} \\ \hline %& \textbf{Hum.} & \textbf{Sport} \\ \hline
\textit{HUMAN} & - & 49.29 & 0.32/0.75/0.83 & 5.97 \\ % & 52.22 & 18.32 \\
\textit{DGPT} & 82.09 & 38.00 & 0.22/0.64/0.78 & 27.86 \\ % & 49.00 & 35.08 \\
\textit{DGPT+WD} & 86.57 & 54.98 & 0.23/0.74/0.85 & 36.82 \\ % & 50.29 & 53.75 \\
\textit{PPLM} & 95.52 & 42.81 & 0.23/0.66/0.80 & 59.20 \\ % & 49.92 & 54.48 \\
\textit{ADAPTER} & 98.51 & 40.36 & 0.16/0.61/0.82 & 83.08 \\ \hline % & 48.57 & 78.37 \\ \hline
\end{tabular}
\caption{Automatic evaluation results on topic Sports.}
\end{table}

\begin{figure}[H]
    \centering
    \begin{subfigure}[b]{0.4\textwidth}
         \centering
         \includegraphics[width=\textwidth]{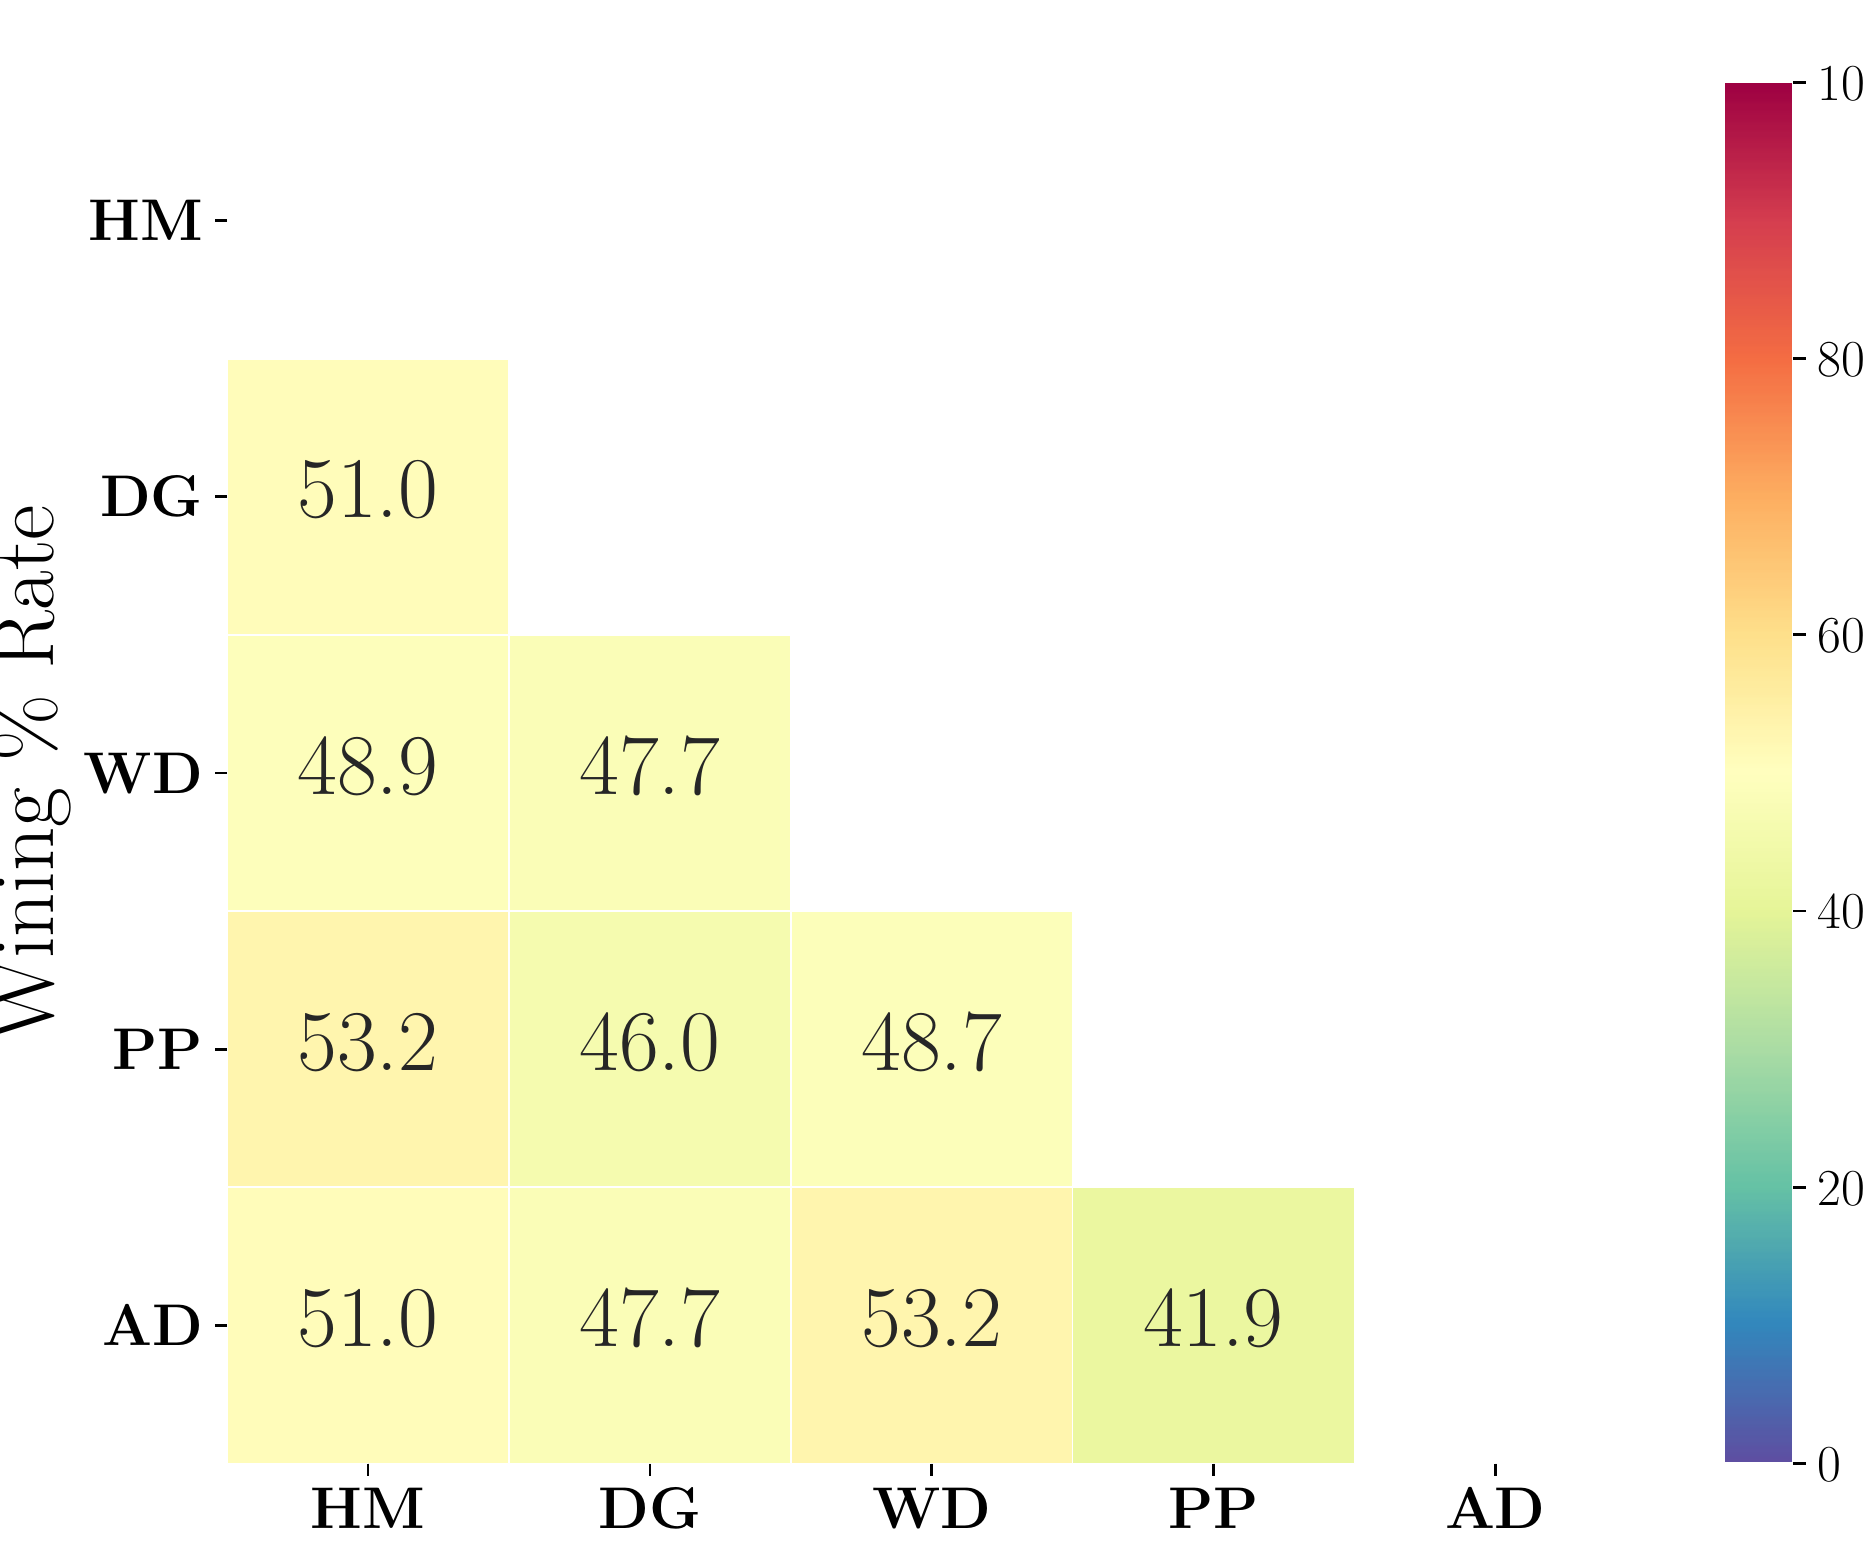}
         \caption{Humanness}
         \label{fig:sports_human}
     \end{subfigure}
     \hspace{0.03\textwidth}
     \begin{subfigure}[b]{0.4\textwidth}
         \centering
         \includegraphics[width=\textwidth]{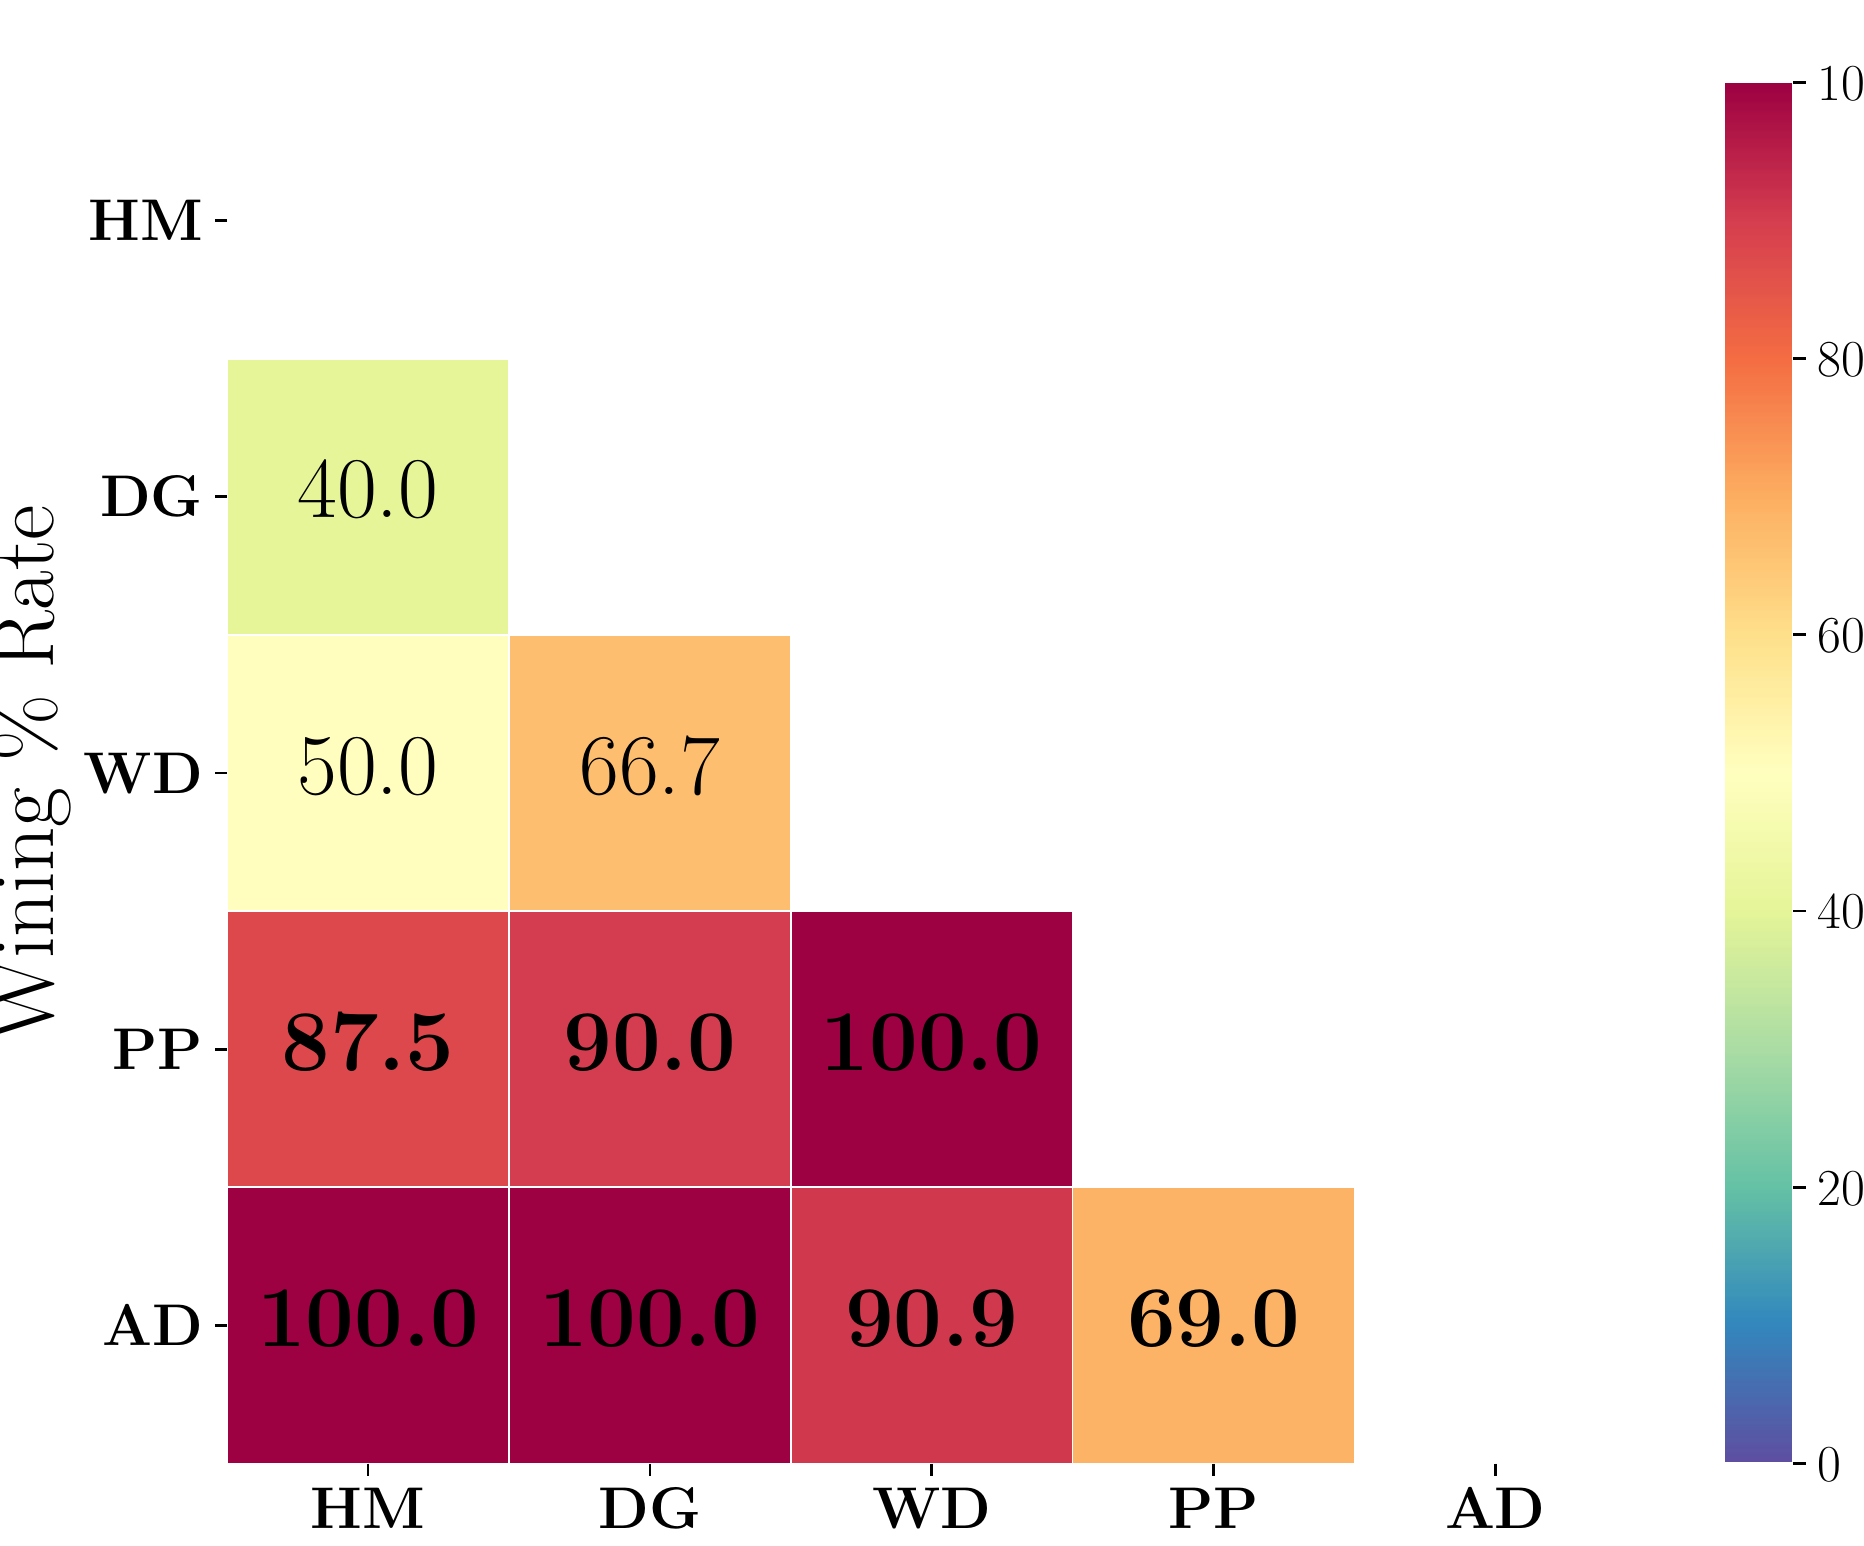}
         \caption{Sports}
         \label{fig:sports_style}
     \end{subfigure}
    \caption{Human evaluation results in terms of winning rate for humanness and sports.}
    \label{fig:human_sports}
\end{figure}

\begin{table}[H]
    \centering
    \resizebox{\linewidth}{!}{
    \begin{tabular}{lll}
    \hline
    \multirow{2}{*}{1.}              & HUMAN 1                                     & Hey there! What's up???                                          \\
                                     & HUMAN 2                                     & Nothing much, how you doin?                                      \\ \hline
    \multicolumn{1}{l|}{\textit{DG}} & \multicolumn{2}{l}{I've been pretty alright, actually. How about you?}                                         \\ \hline
    \multicolumn{1}{l|}{\textit{WD}} & \multicolumn{2}{l}{I'm alright, you wanna hang out later}                                                      \\ \hline
    \multicolumn{1}{l|}{\textit{PP}} & \multicolumn{2}{l}{Just doing well! Watching a Bills vs Giants game right now. How about yourself?}            \\ \hline
    \multicolumn{1}{l|}{\textit{AD}} &
      \multicolumn{2}{l}{\begin{tabular}[c]{@{}l@{}}doing pretty well! Just had a nice soccer practice with the U21s and the coach likes me for some reason. \\ How have you been?\end{tabular}} \\ \hline
    \multirow{2}{*}{2.}              & HUMAN 1                                     & hey                                                              \\
                                     & HUMAN 2                                     & is it raining pretty bad today?                                  \\ \hline
    \multicolumn{1}{l|}{\textit{DG}} & \multicolumn{2}{l}{It's always sunny in Philadelphia. I'm from PA, but I've lived in Philly my entire life.}   \\ \hline
    \multicolumn{1}{l|}{\textit{WD}} & \multicolumn{2}{l}{It rained all through college but we have the same rain. So... kinda, yes, kinda?}          \\ \hline
    \multicolumn{1}{l|}{\textit{PP}} & \multicolumn{2}{l}{It's sunny. The weatherman is wrong, but I think the rain will be okay for the rest of us.} \\ \hline
    \multicolumn{1}{l|}{\textit{AD}} &
      \multicolumn{2}{l}{The track is dry but the racing is still pretty rough in some tracks and the racing on the track is not as good.} \\ \hline
    \end{tabular}
    }
    \caption{Generated responses for Sports topic. In both examples, Sports vocabulary such as ``soccer" or ``racing" can be observed in \textit{AD}.}
\end{table}

\subsection*{Science \& Technology}
\label{appendix:scitech}

\begin{table}[H]
\centering
\begin{tabular}{r|cccc}
\hline
\multicolumn{1}{c|}{\textbf{Model}} & \textbf{Disc.} & \textbf{Ppl.} & \textbf{Dist.} & \textbf{Score} \\ \hline % & \textbf{Hum.} & \textbf{Sci \& Tech} \\ \hline
\textit{HUMAN} & - & 49.29 & 0.32/0.75/0.83 & 91.04 \\ % & 48.98 & 30.63 \\
\textit{DGPT} & 99.00 & 39.25 & 0.23/0.65/0.78 & 91.04 \\ % & 52.38 & 20.83 \\
\textit{DGPT+WD} & 99.50 & 58.60 & 0.25/0.77/0.87 & 91.04 \\ % & 48.68 & 31.44 \\
\textit{PPLM} & 100.00 & 44.43 & 0.26/0.72/0.82 & 93.03 \\ % & 51.51 & 77.13 \\
\textit{ADAPTER} & 100.00 & 41.11 & 0.19/0.66/0.84 & 99.00 \\ \hline % & 48.45 & 89.97 \\ \hline
\end{tabular}
\caption{Automatic evaluation results on the topic Science \& Technology.}
\end{table}

\begin{figure}[H]
    \centering
    \begin{subfigure}[b]{0.4\textwidth}
         \centering
         \includegraphics[width=\textwidth]{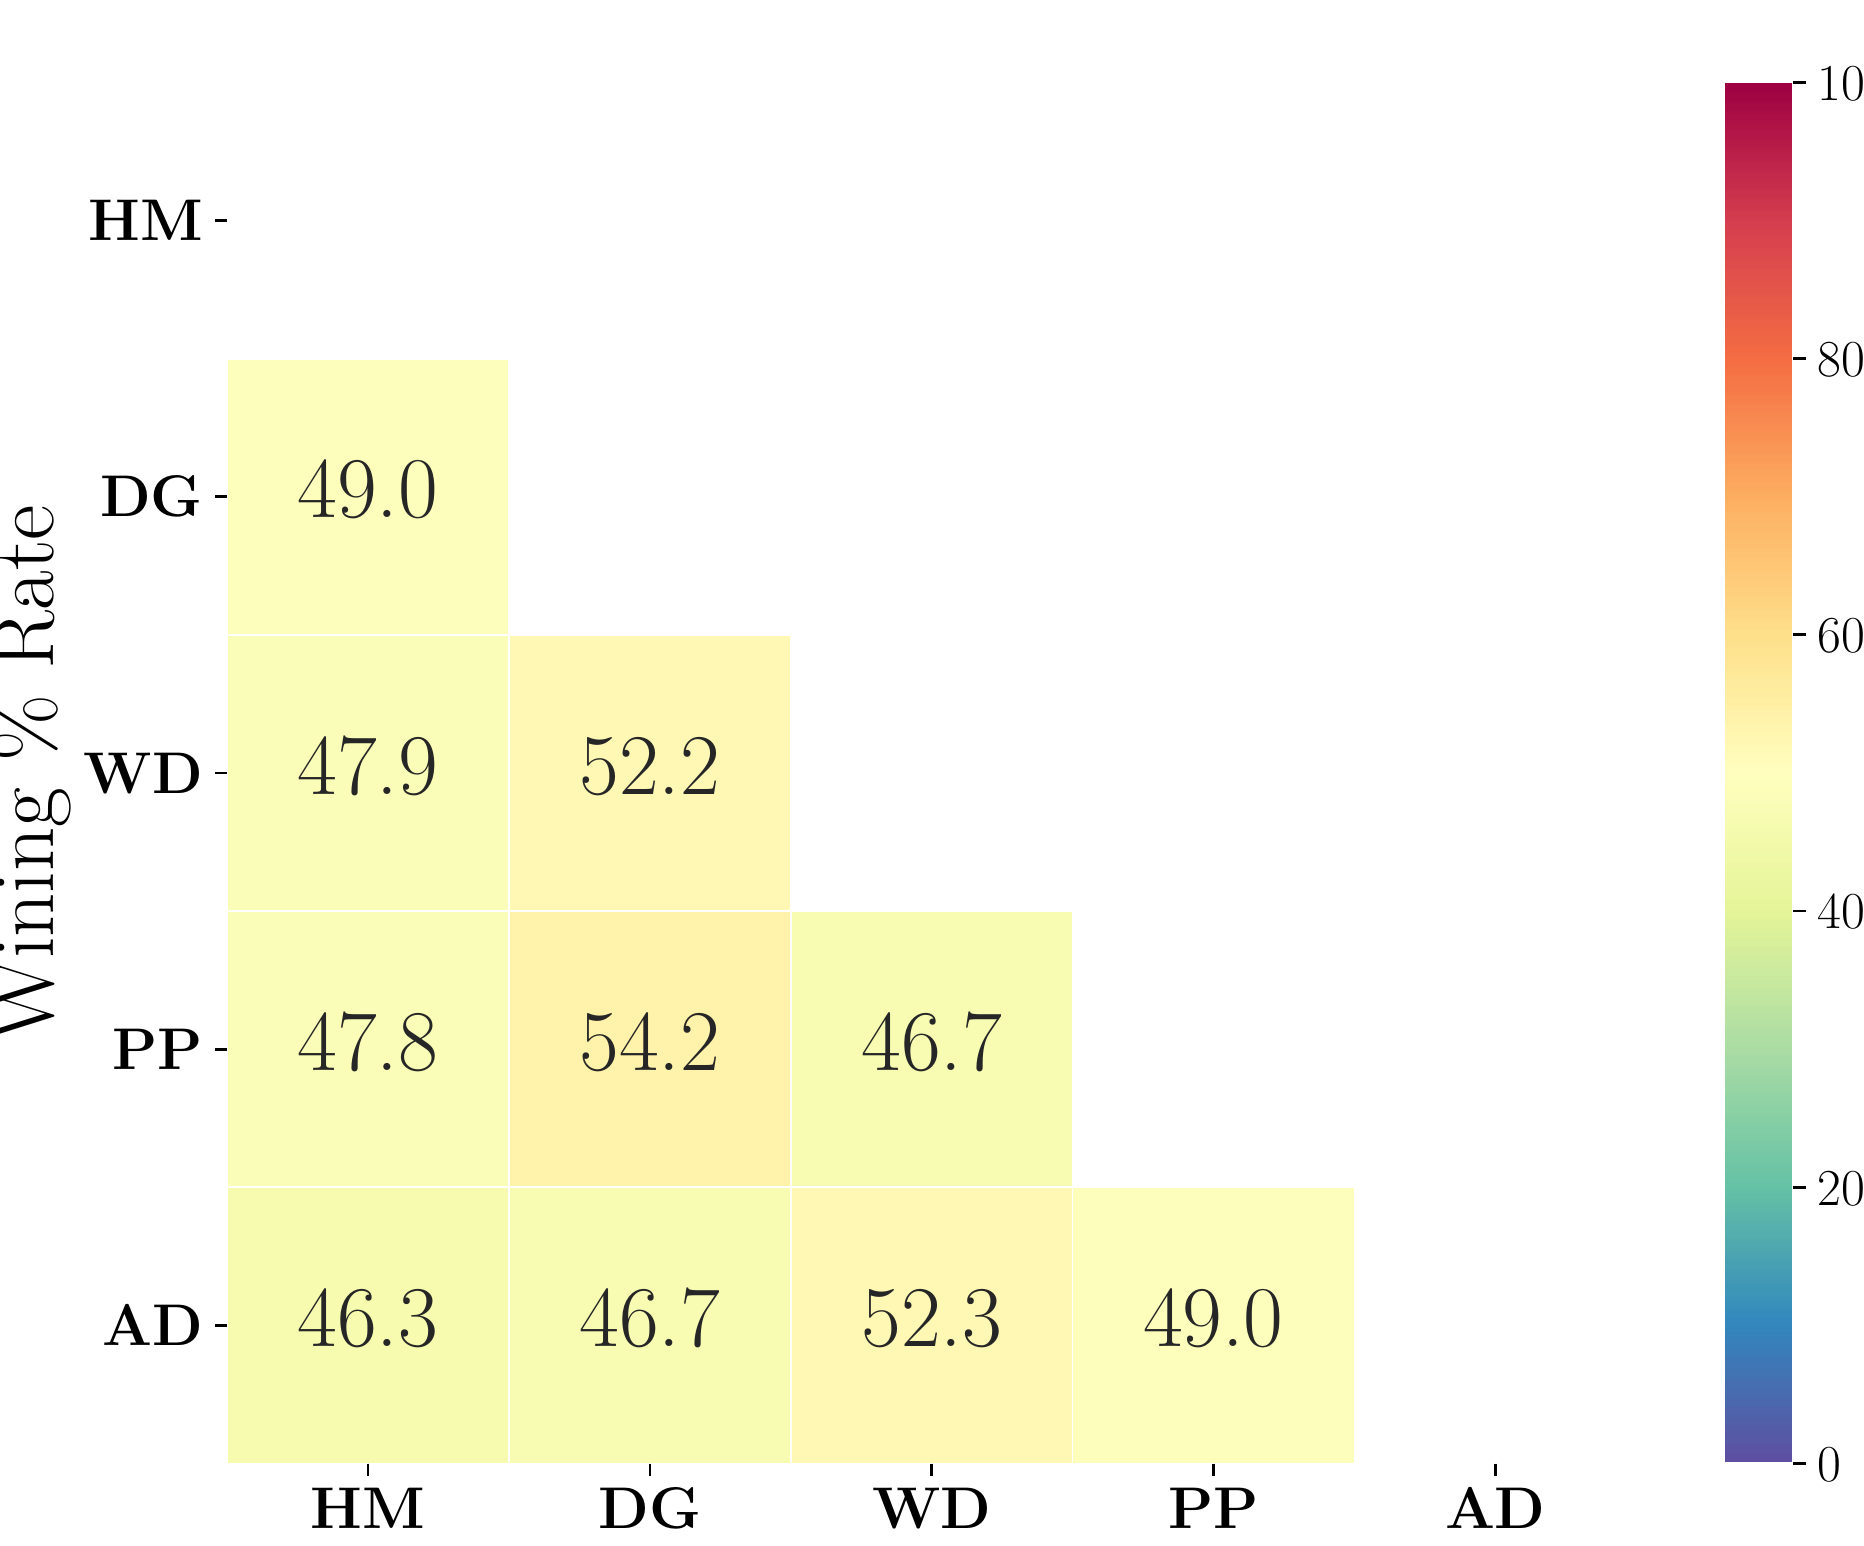}
         \caption{Humanness}
         \label{fig:scitech_human}
     \end{subfigure}
     \hspace{0.03\textwidth}
     \begin{subfigure}[b]{0.4\textwidth}
         \centering
         \includegraphics[width=\textwidth]{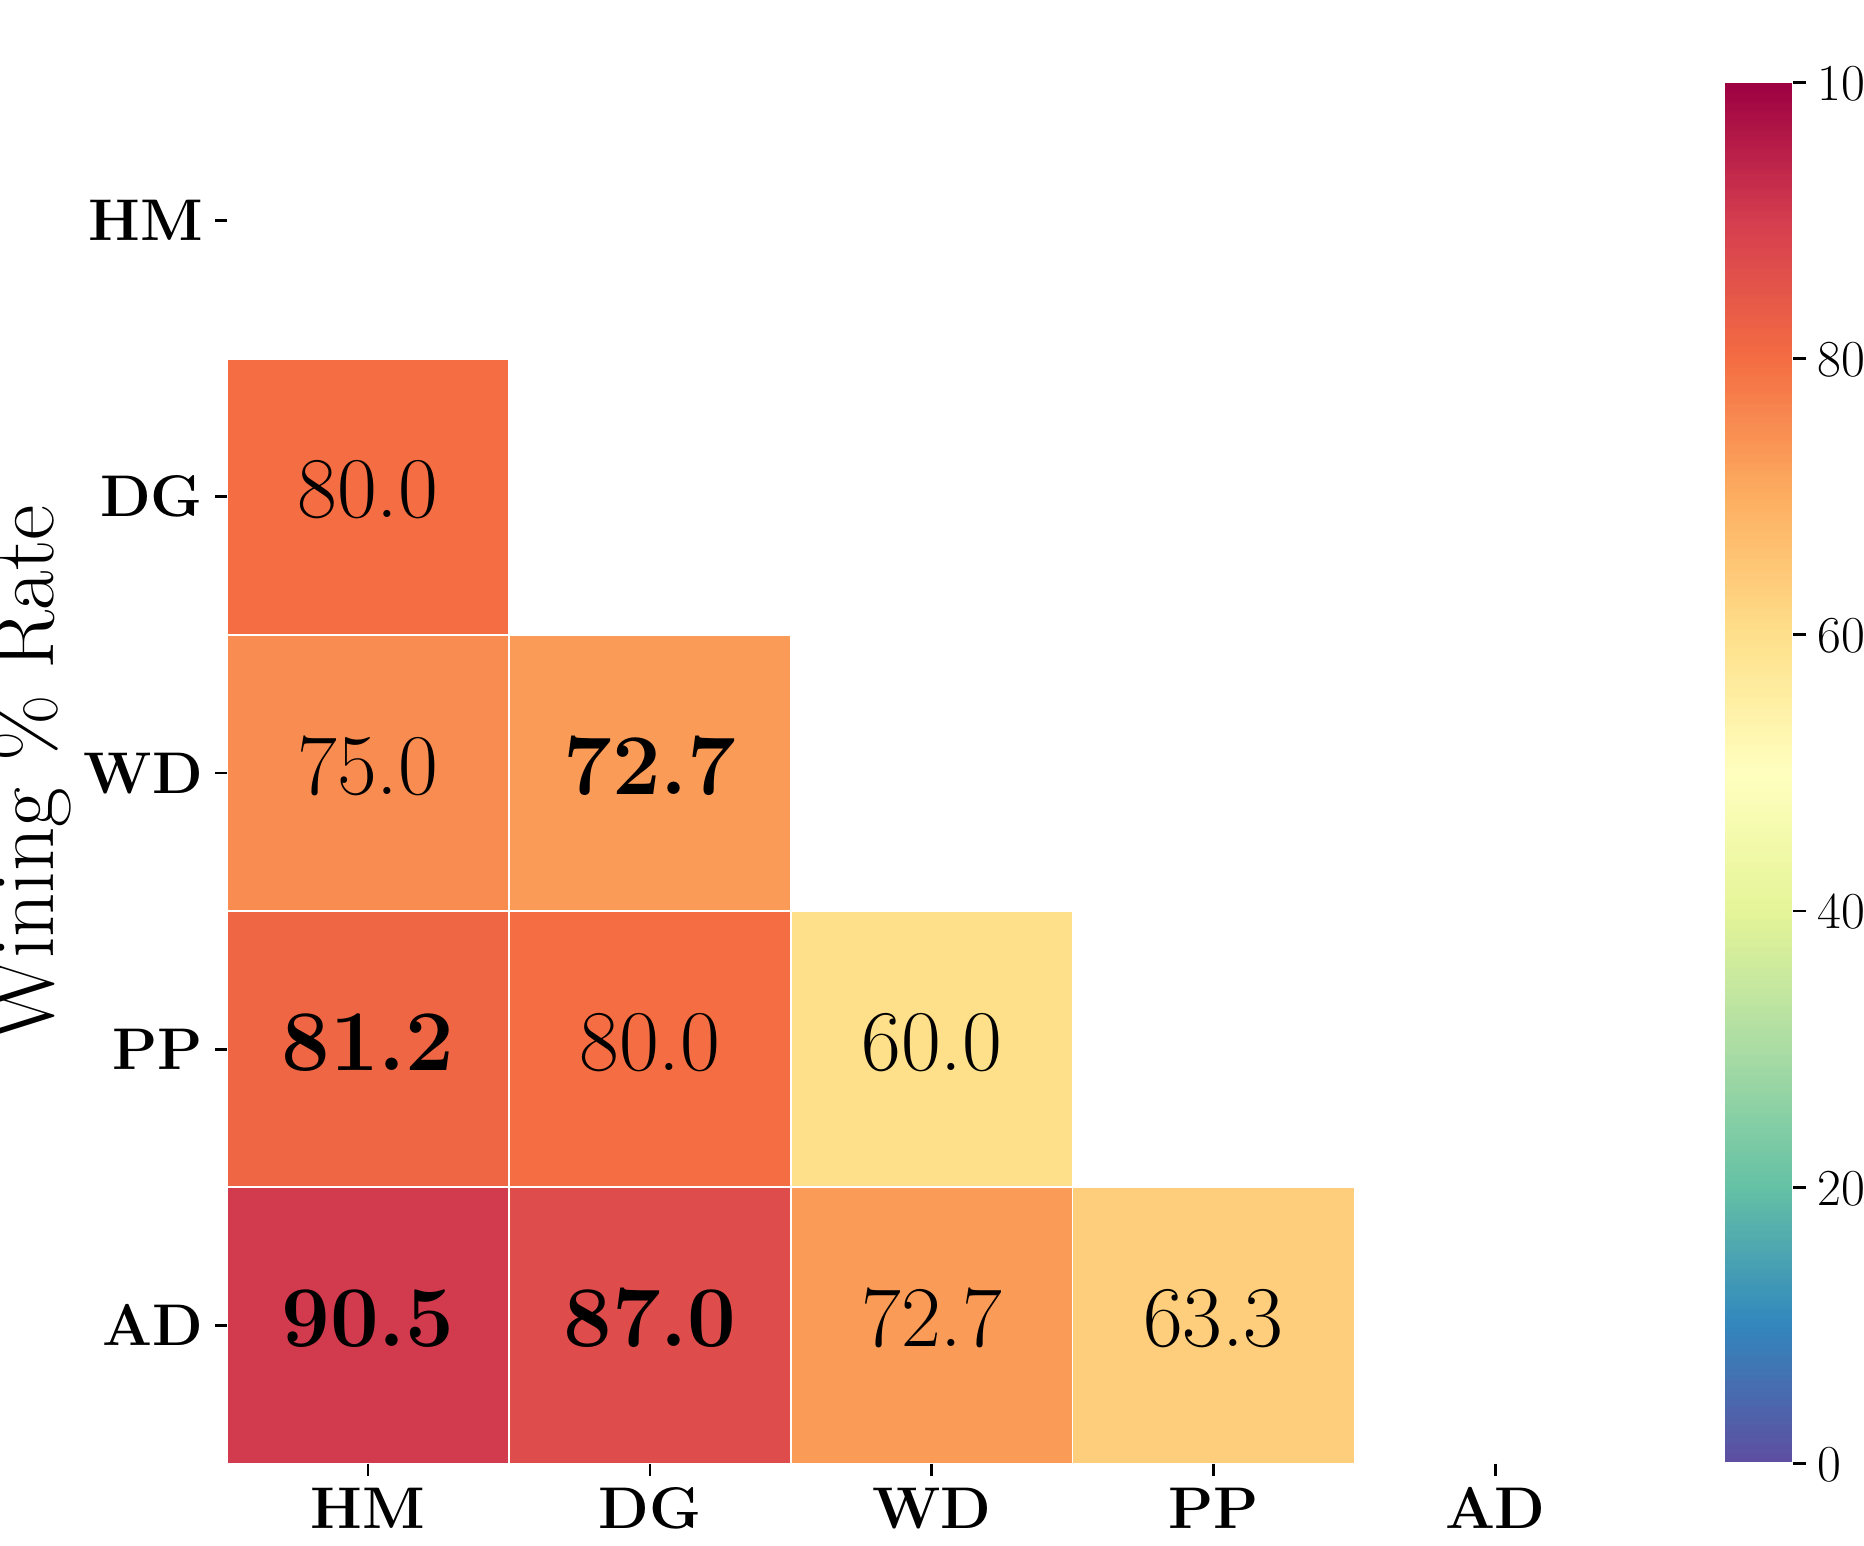}
         \caption{Sci/Tech}
         \label{fig:scitech_style}
     \end{subfigure}
    \caption{Human evaluation results in terms of winning rate for humanness and Sci/Tech.}
    \label{fig:human_scitech}
\end{figure}

\begin{table}[H]
    \centering
    \resizebox{\linewidth}{!}{
    \begin{tabular}{lll}
    \hline
    \multirow{2}{*}{1.}              & HUMAN 1                 & Hi!                                                                     \\
                                     & HUMAN 2                 & Oh hello. Long time no talk. How's the day going for yuo?               \\ \hline
    \multicolumn{1}{l|}{\textit{DG}} & \multicolumn{2}{l}{Well, i got home and watched an episode of the IT crowd. What about you?}      \\ \hline
    \multicolumn{1}{l|}{\textit{WD}} & \multicolumn{2}{l}{I've gotten some work done, but not done much else today.}                     \\ \hline
    \multicolumn{1}{l|}{\textit{PP}} & \multicolumn{2}{l}{Good, working, studying and gaming,}                                           \\ \hline
    \multicolumn{1}{l|}{\textit{AD}} &
      \multicolumn{2}{l}{\begin{tabular}[c]{@{}l@{}}Good, working, studying and gaming. How is yours? What are you studying for? I love computer \\ science and computer engineering.\end{tabular}} \\ \hline
    \multirow{2}{*}{2.}              & HUMAN 1                 & is it raining pretty bad today?                                         \\
                                     & HUMAN 2                 & yeah, can walk too far to see all the foodtruck options                 \\ \hline
    \multicolumn{1}{l|}{\textit{DG}} & \multicolumn{2}{l}{I wish there was more variety in the weather. I live right next to the beach.} \\ \hline
    \multicolumn{1}{l|}{\textit{WD}} & \multicolumn{2}{l}{I've heard they have free pizza. That counts right?}                           \\ \hline
    \multicolumn{1}{l|}{\textit{PP}} & \multicolumn{2}{l}{i got my own netflix. i love this sub, lol!}                                   \\ \hline
    \multicolumn{1}{l|}{\textit{AD}} &
      \multicolumn{2}{l}{\begin{tabular}[c]{@{}l@{}}i just use my laptop and play video games. i don't use my phone to stream music or anything though\\ because that would be a net loss\end{tabular}} \\ \hline
     \end{tabular}
    }
    \caption{Generated responses for Sci/Tech topic. Given a general starter, \textit{DG} generates a response containing techy words by default as in the first example. Since the provided context is less natural for the Sci/Tech attribute in the second example, \textit{AD} generates a response that gives off an erratic impression.}
    \label{tab:scitech_gen}
\end{table}

\clearpage

\section*{Chapter 4: Controlling Dialogue Domains Continuously}

\section*{A Hyper-Parameters} All the experiments uses GPT-2 small (117M parameters). In all the setting and baselines, we run a small grid-search over several hyper-parameters. In VANILLA and MULTI, we used a learning rate of 0.001 with a warm up schedule and 10 epochs with an early stopping over the validation set. In L2, EWC we tune different $\lambda$ in the range 0.0001 to 100, resulting in $\lambda=0.001$. In A-GEM, we tune $\lambda$ also in the range 0.0001 to 100, resulting in $\lambda=1$. In REPLAY, we use same setting as VANILLA and MULTI, and we tune different Episodic Memory $\mathcal{M}$ in the range 1, 50, 100, 500 and all data sample per task. We select 50 sample per task for a good balance between memory and performance, and we ablate over the memory size. In AdapterCL, we tune the bottleneck size $b$ between 10, 50, 100, and 200, and we select 50 for the modularized settings (INTENT, DST, NLG) and 100 for the E2E. For an adapter with a 50 bottleneck size we add 2.5\% additional parameters per task while with 100  bottleneck size we add 5\% additional parameters.

\begin{figure}[t]
\centering
\begin{subfigure}{.5\textwidth}
    \centering
    \includegraphics[width=\textwidth]{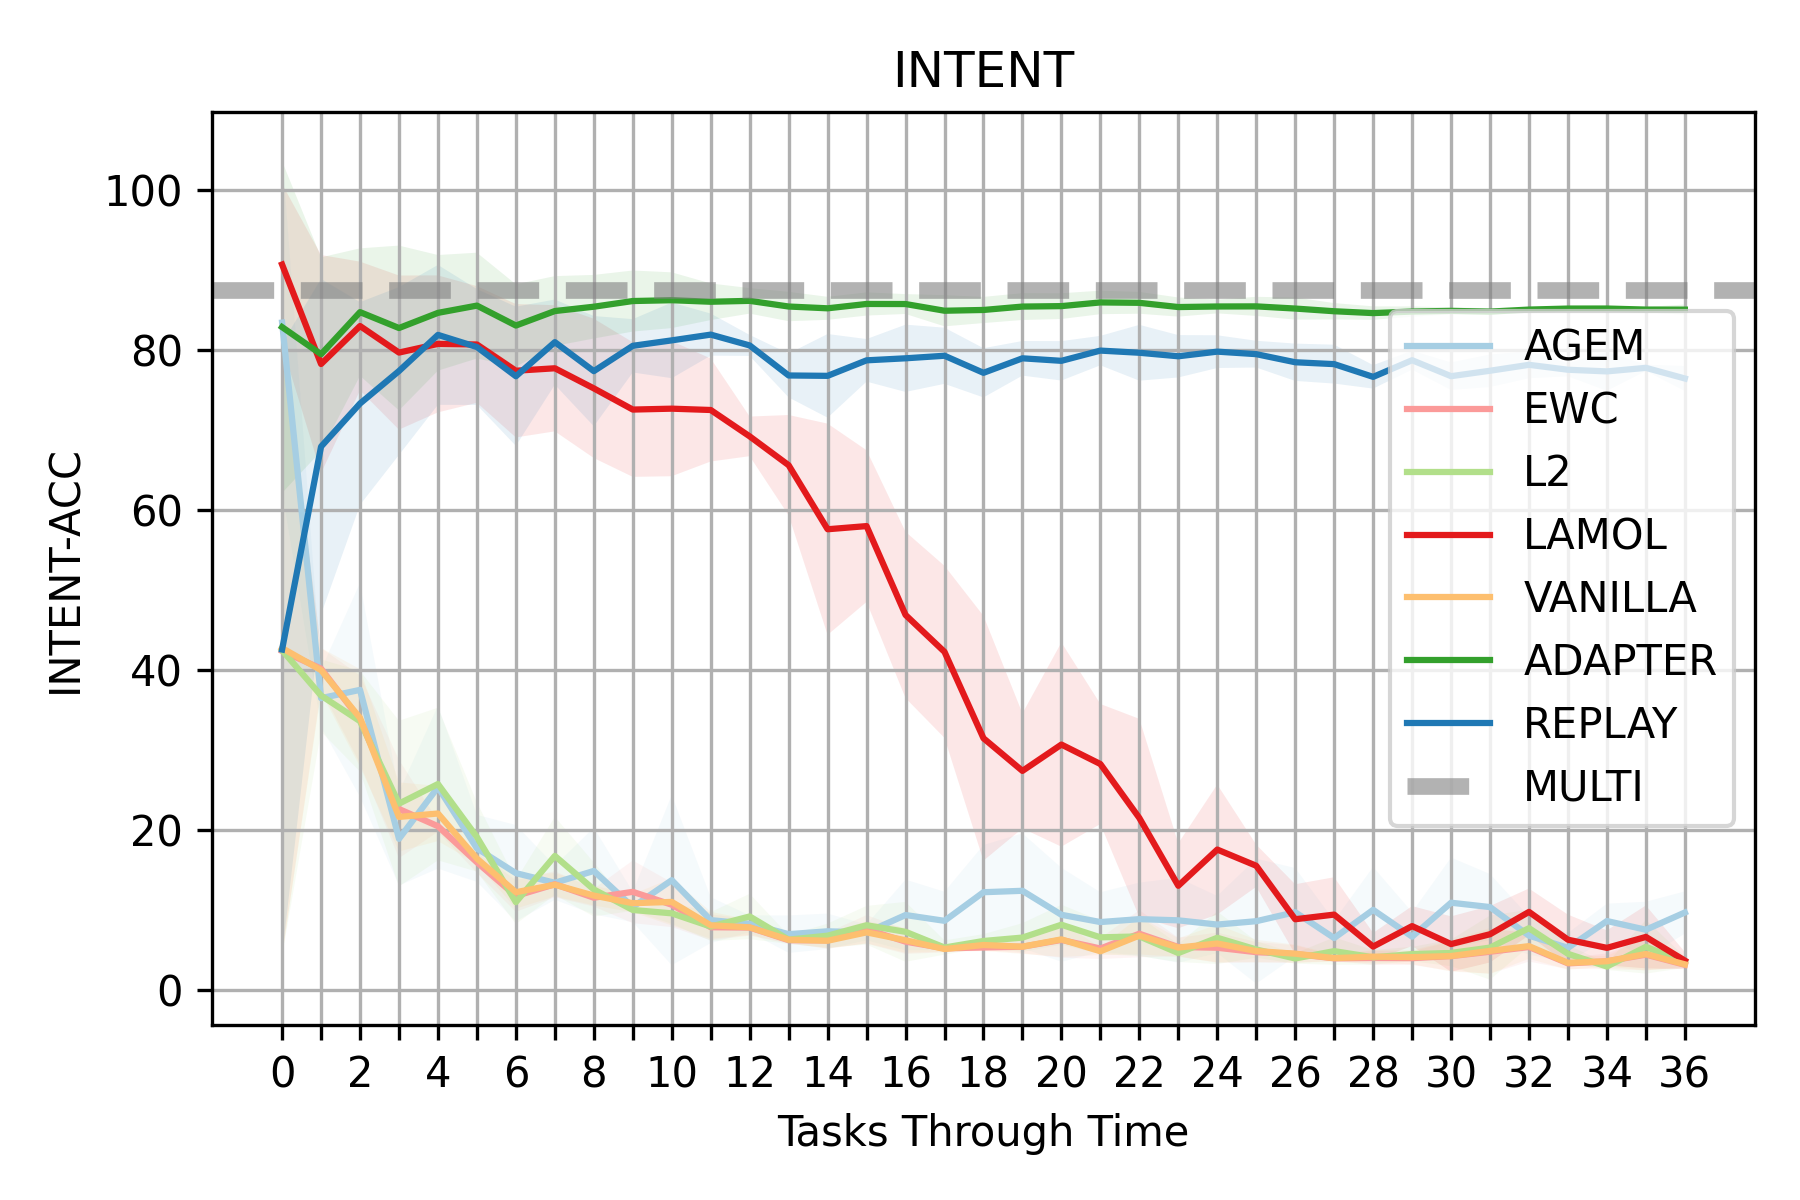}
\end{subfigure}%
\begin{subfigure}{.5\textwidth}
    \centering
    \includegraphics[width=\textwidth]{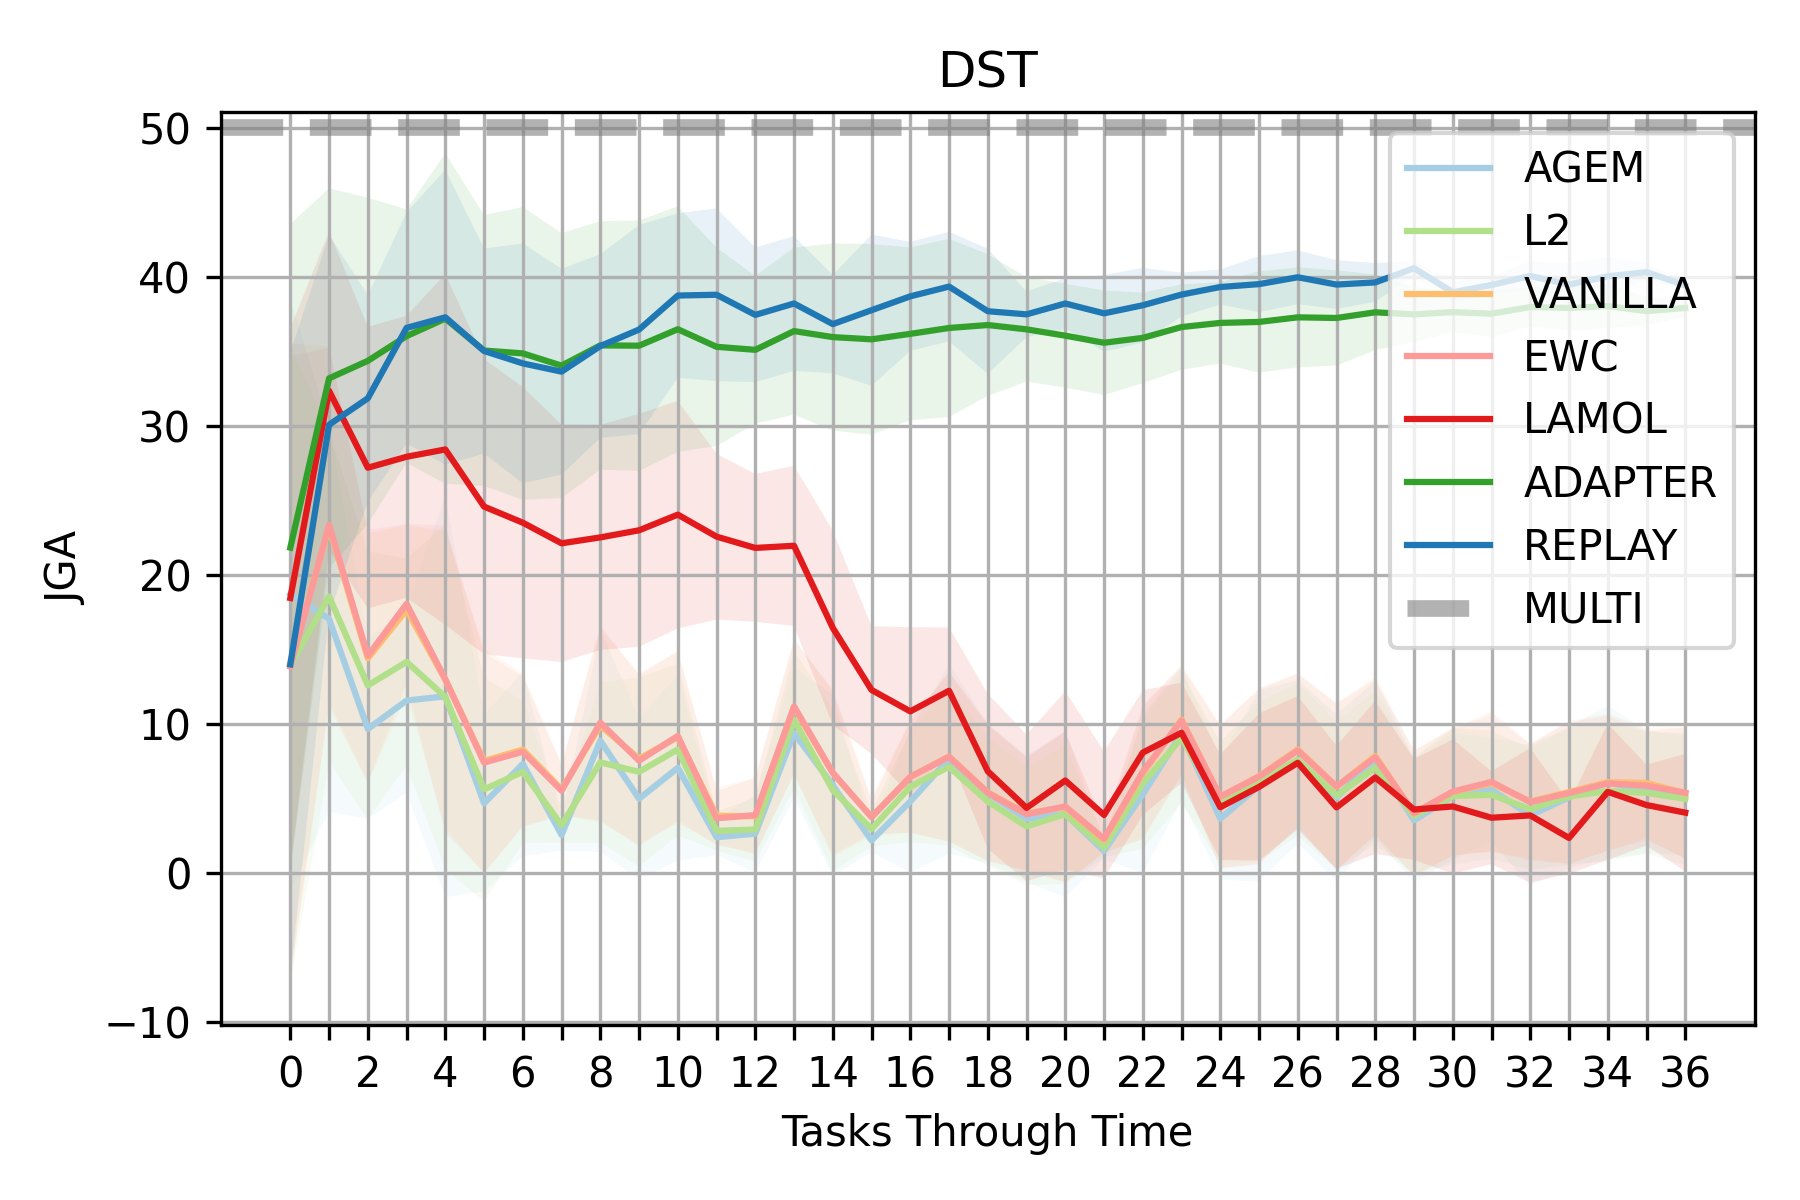}
\end{subfigure}
\begin{subfigure}{.5\textwidth}
    \centering
    \includegraphics[width=\textwidth]{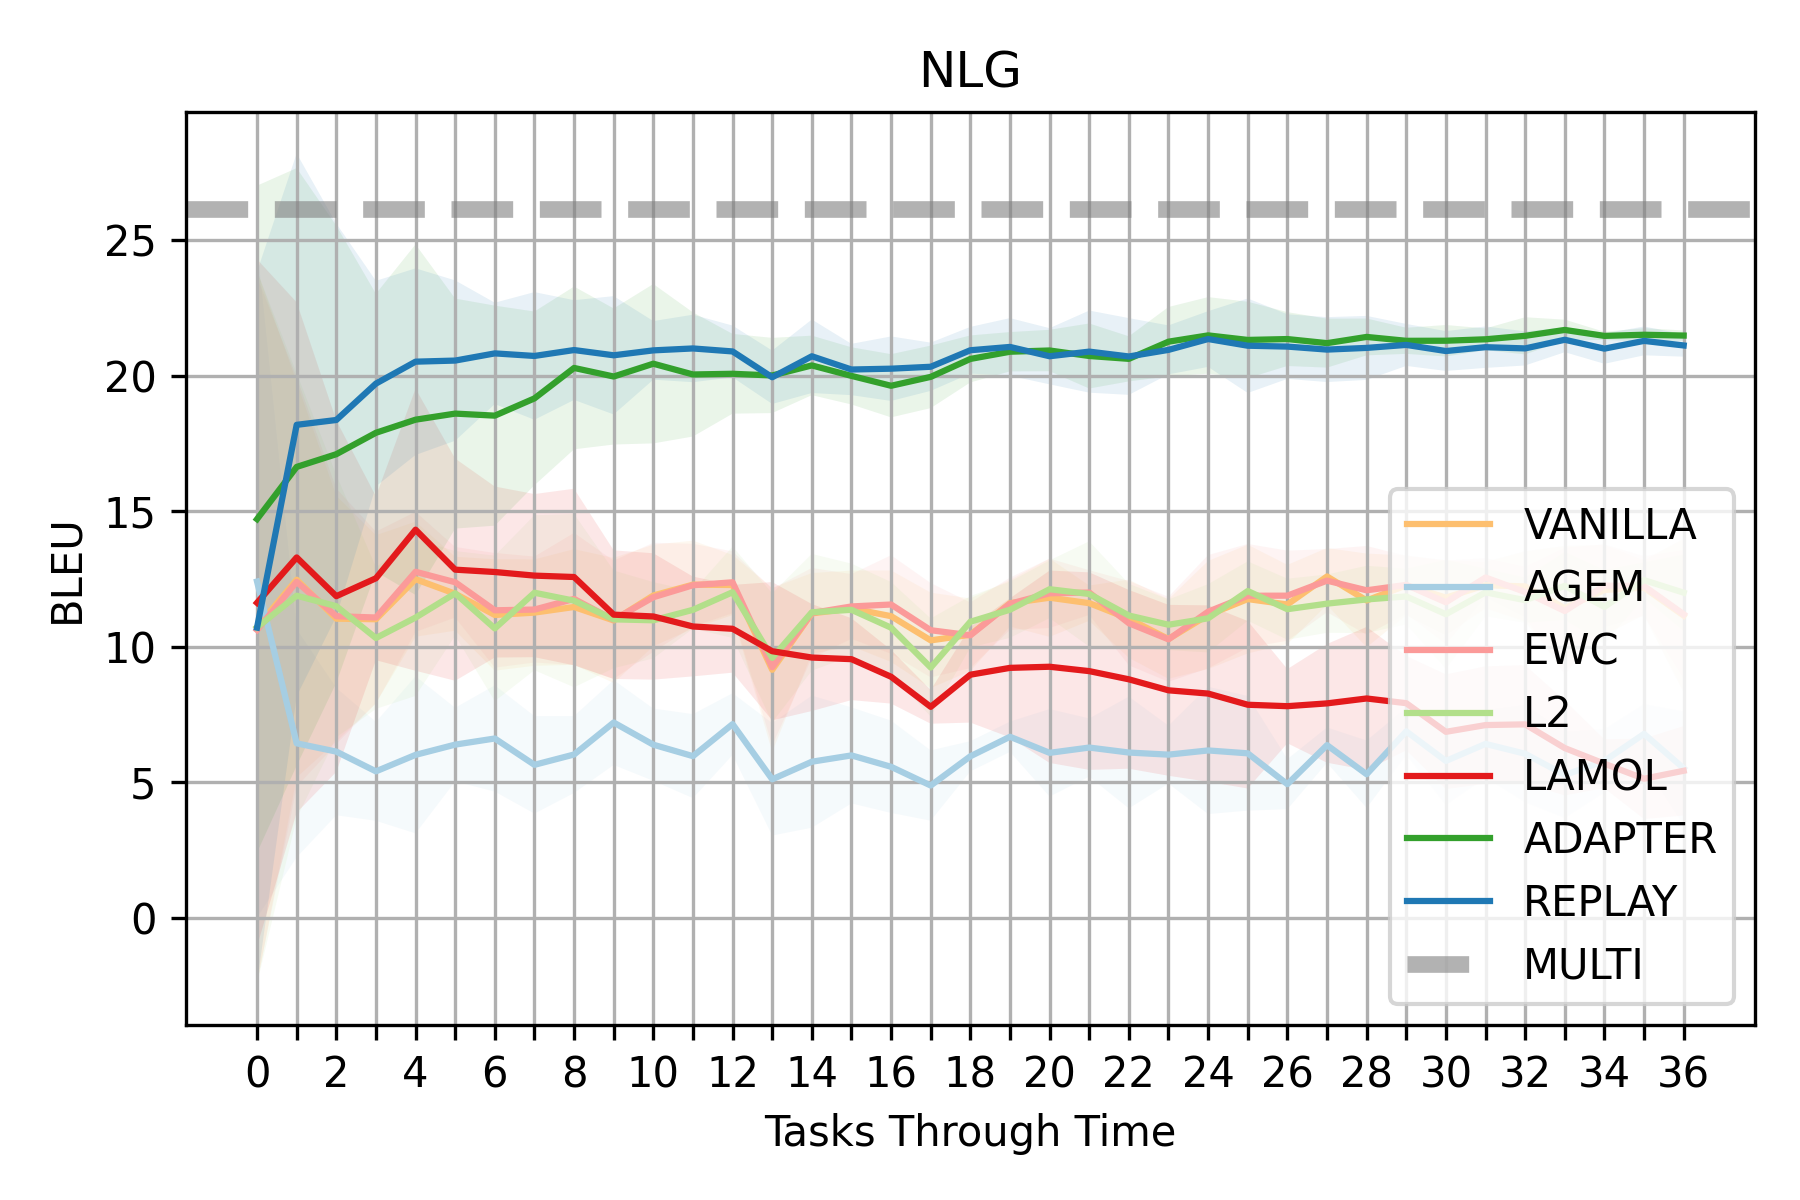}
\end{subfigure}%
\begin{subfigure}{.5\textwidth}
    \centering
    \includegraphics[width=\textwidth]{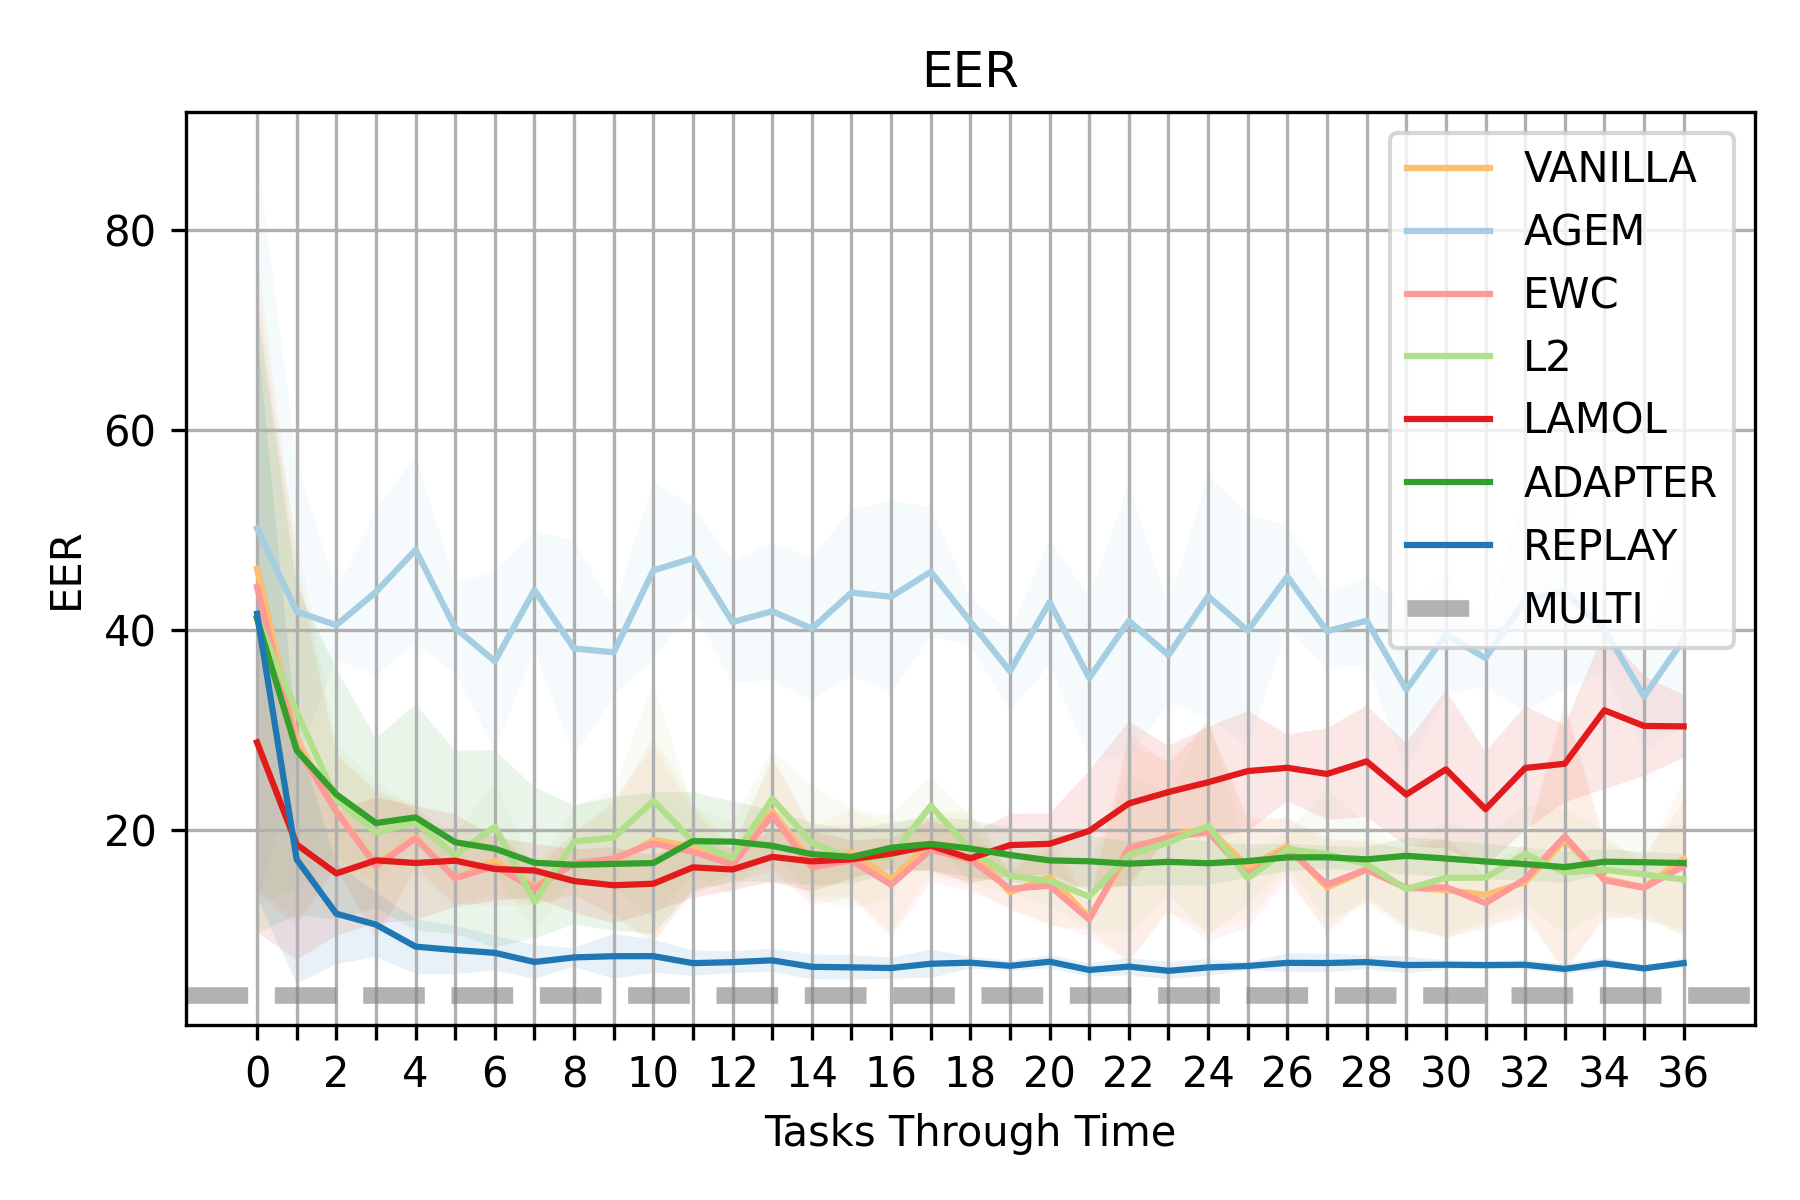}
\end{subfigure}
\caption[short]{Avg. Metric for the Intent Accuracy, JGA, BLEU and EER in the modularized setting.}
\label{fig:MODULE}
\end{figure}

%  \begin{figure}[t]
%     \centering
%     \includegraphics[width=\linewidth]{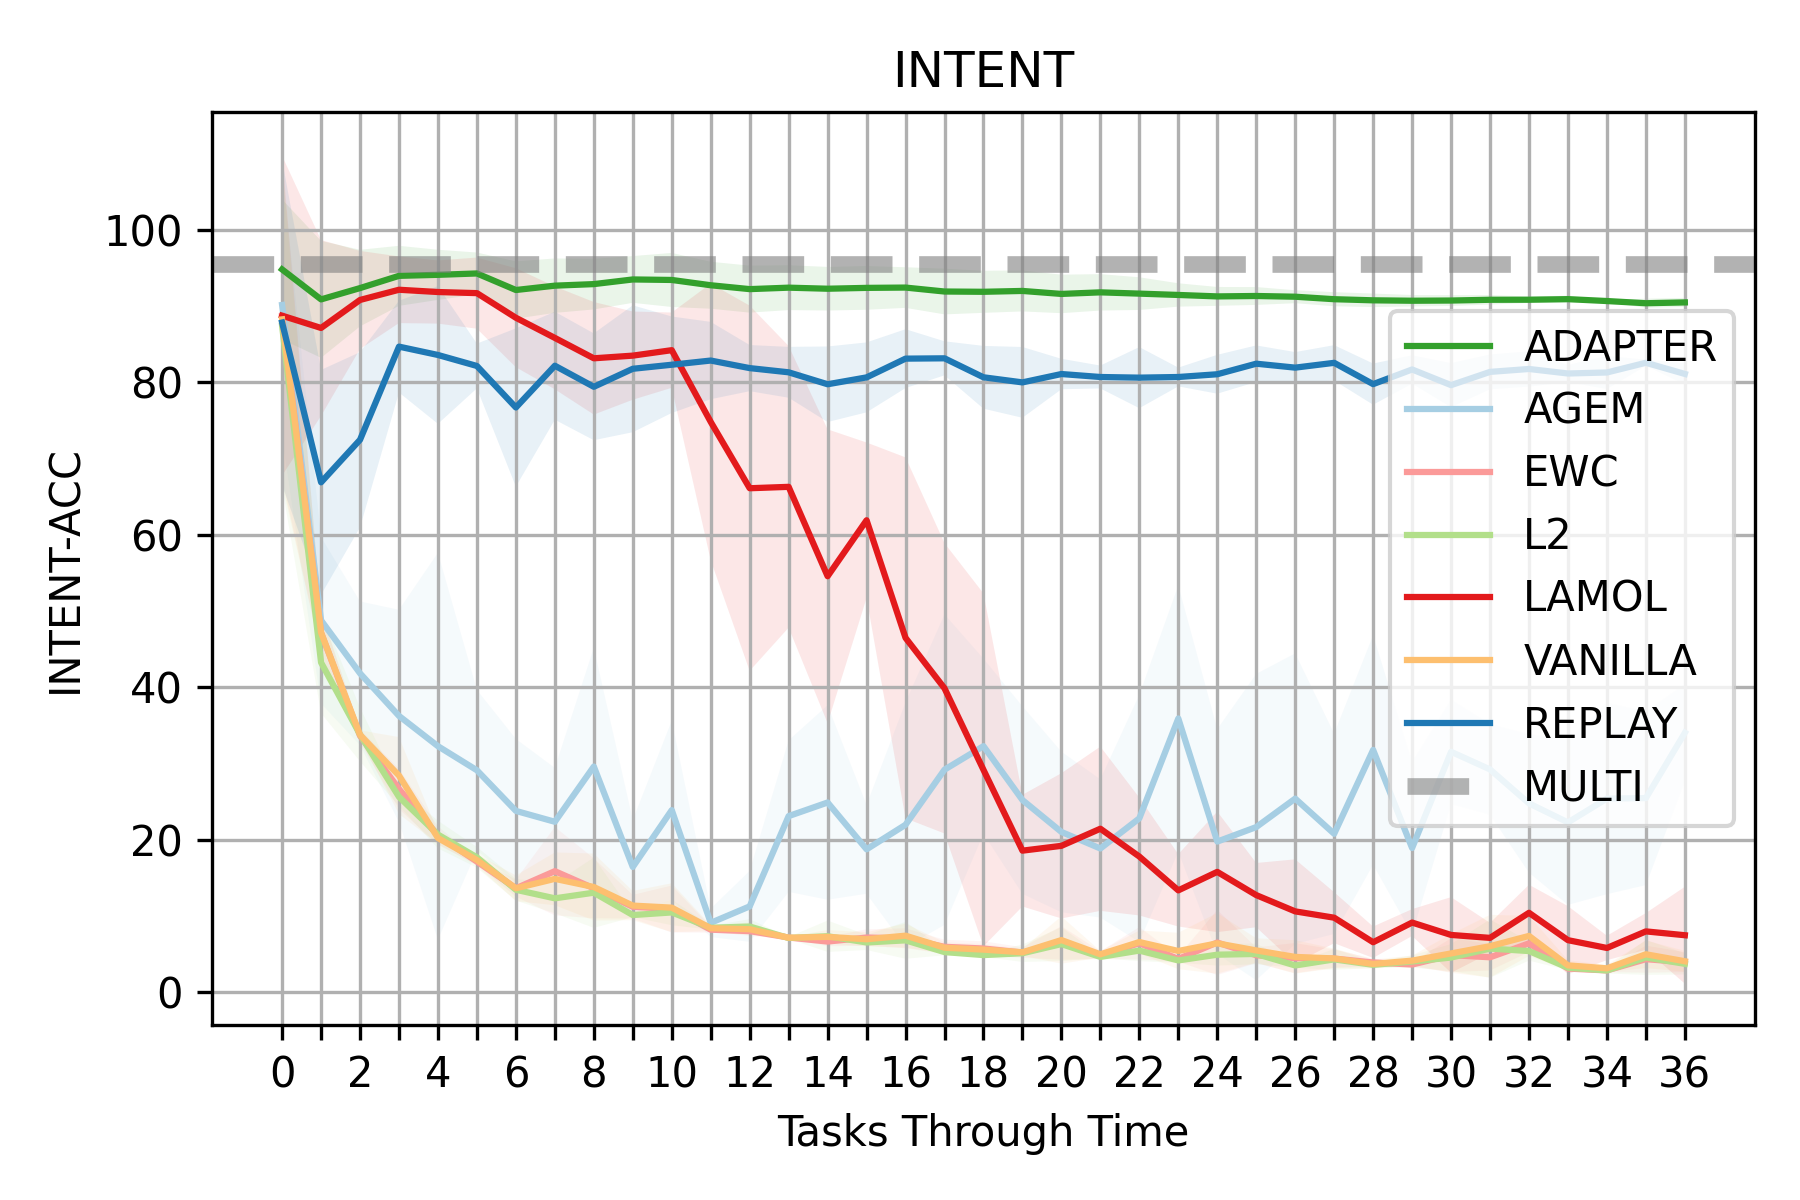}
%     \includegraphics[width=\linewidth]{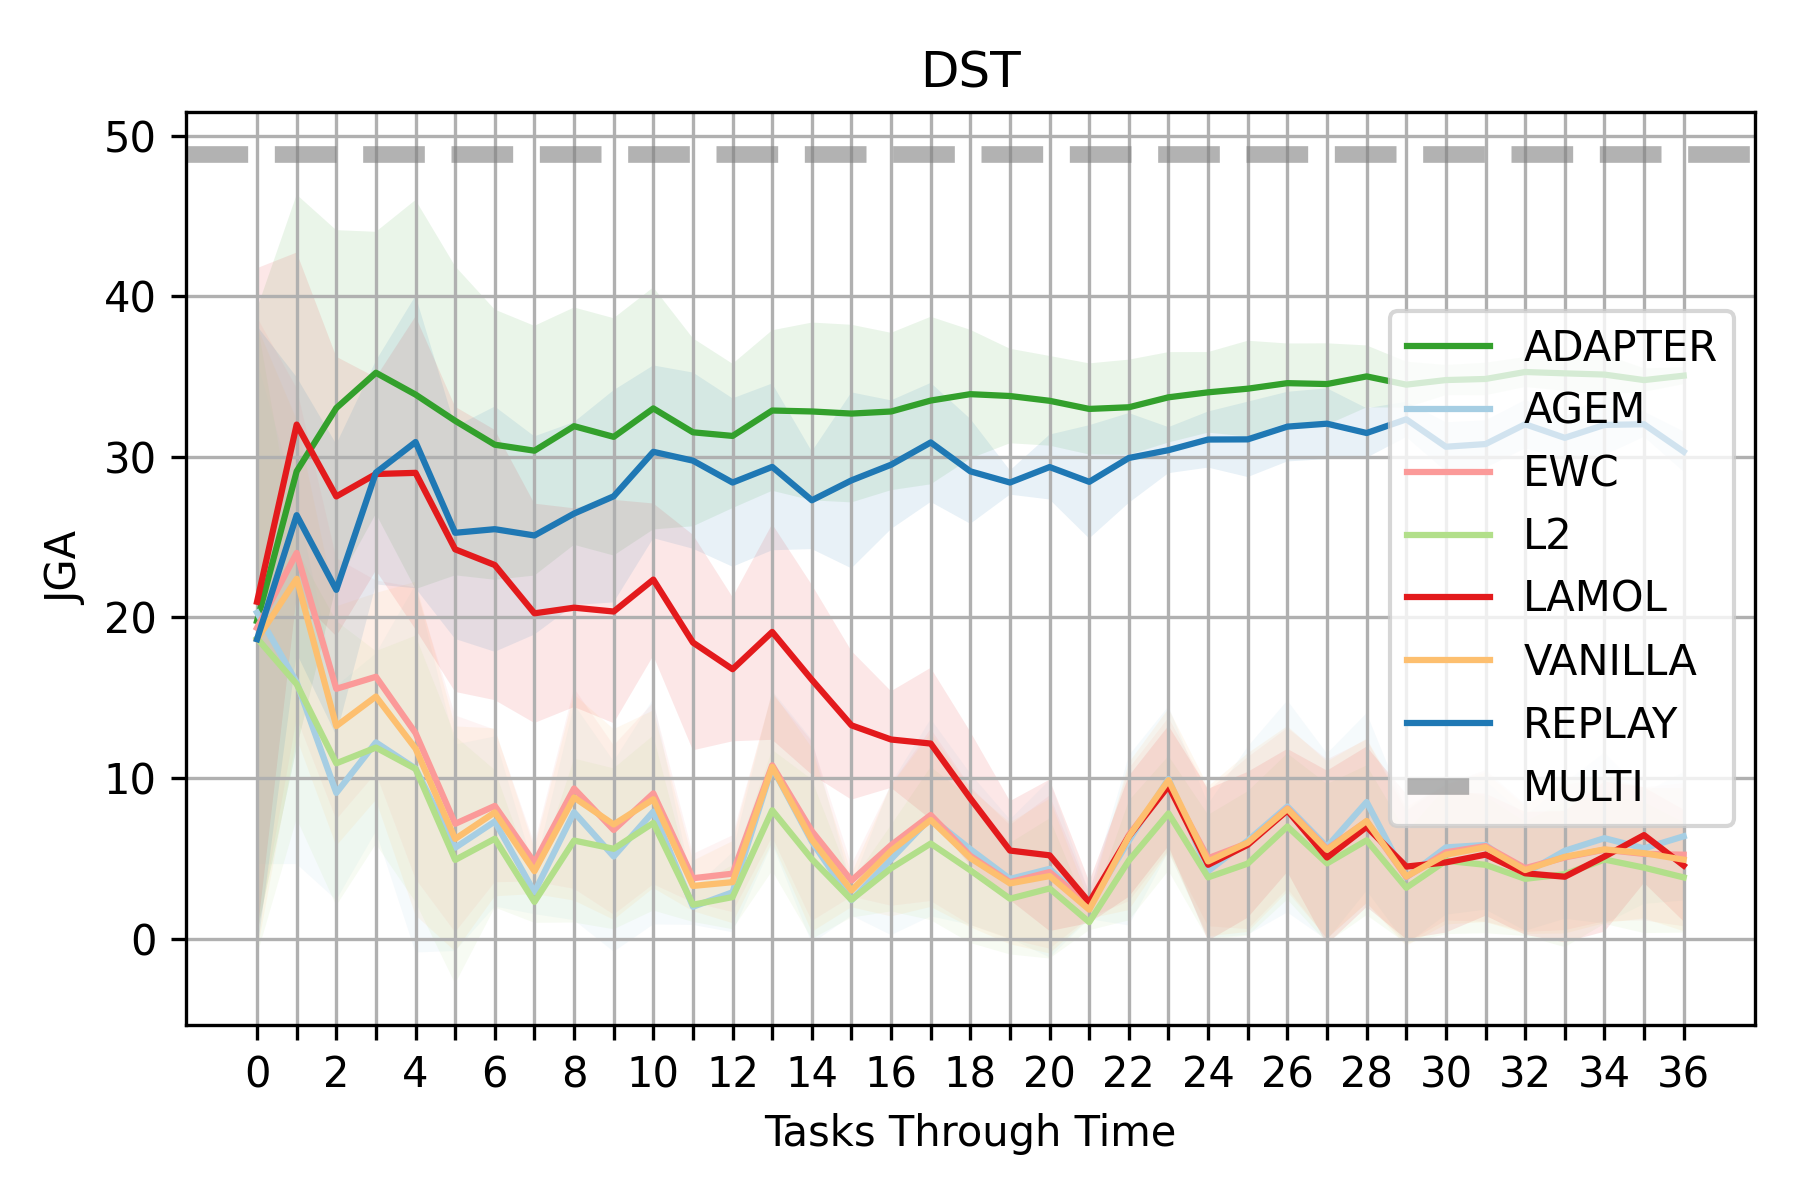}
%     \includegraphics[width=\linewidth]{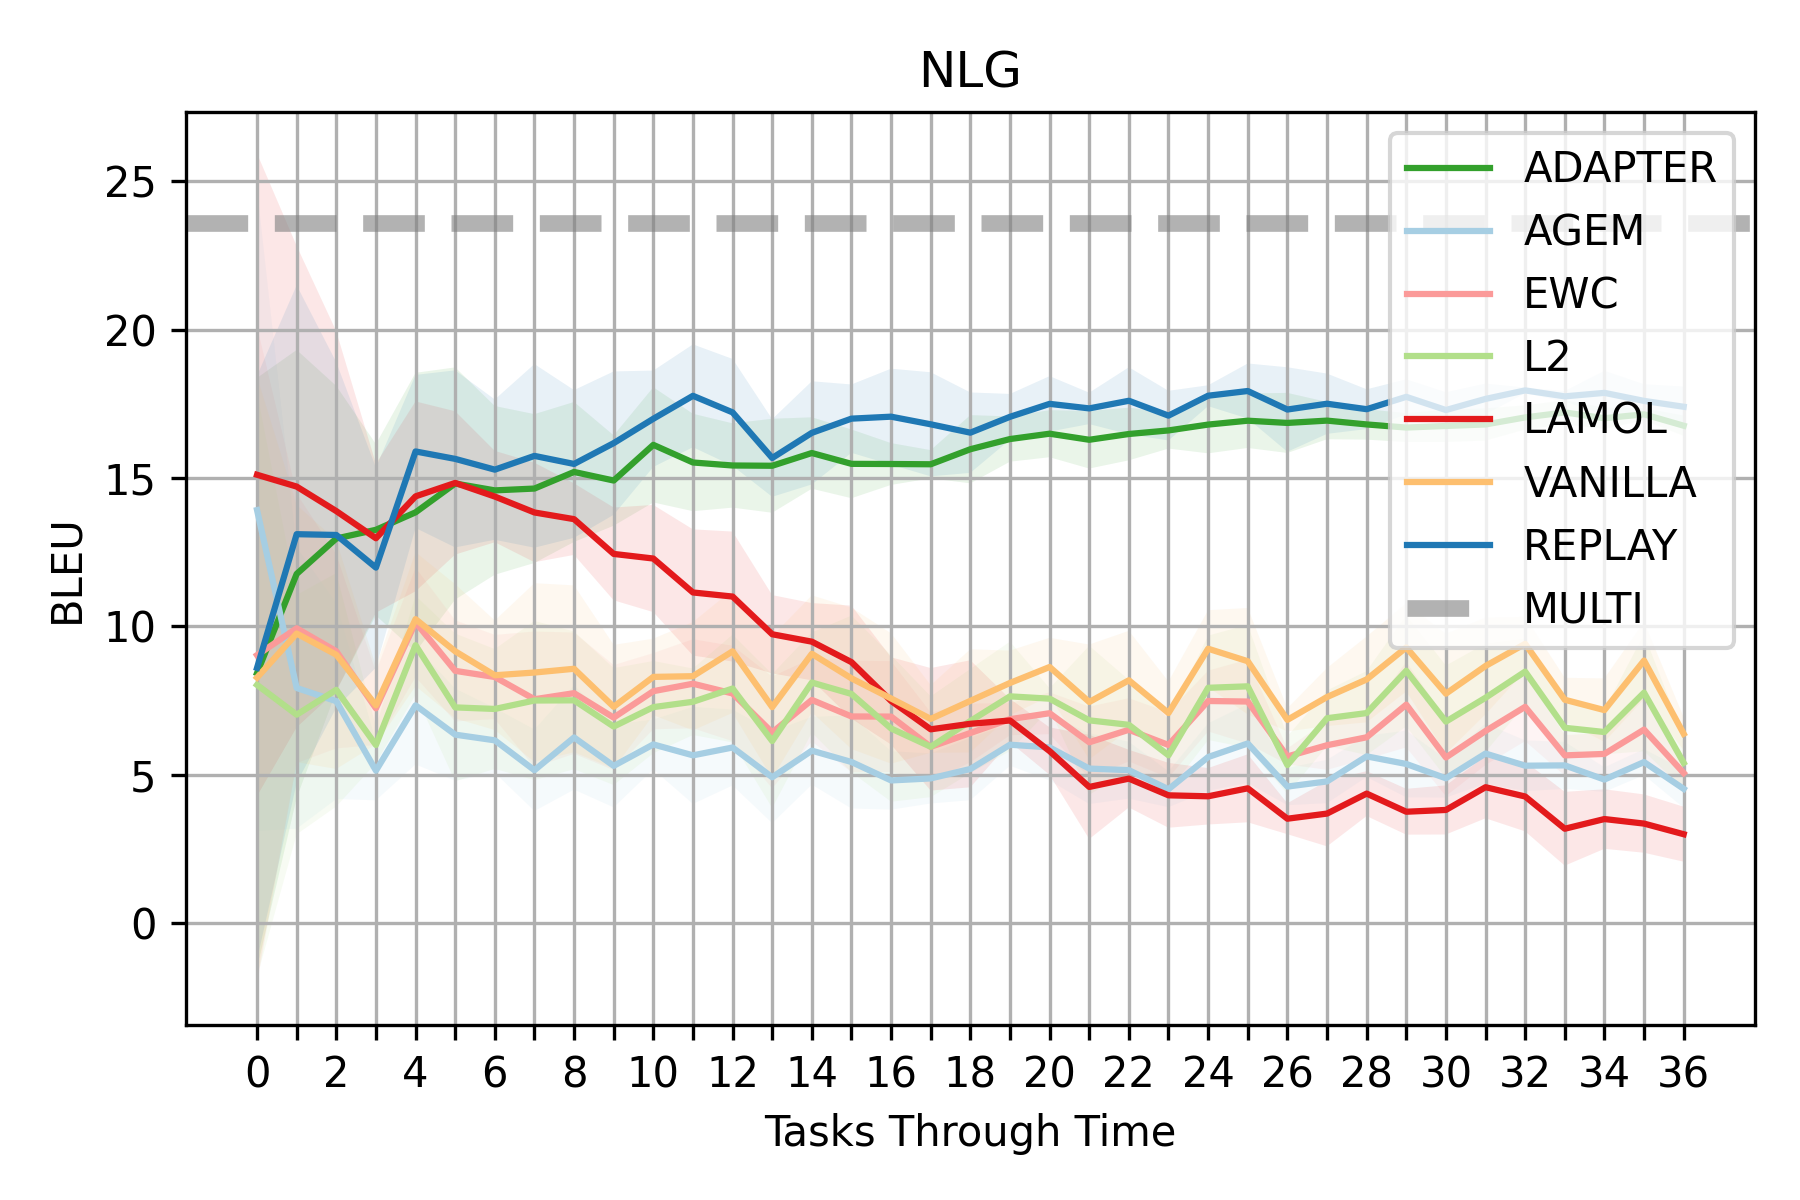}
%     \includegraphics[width=\linewidth]{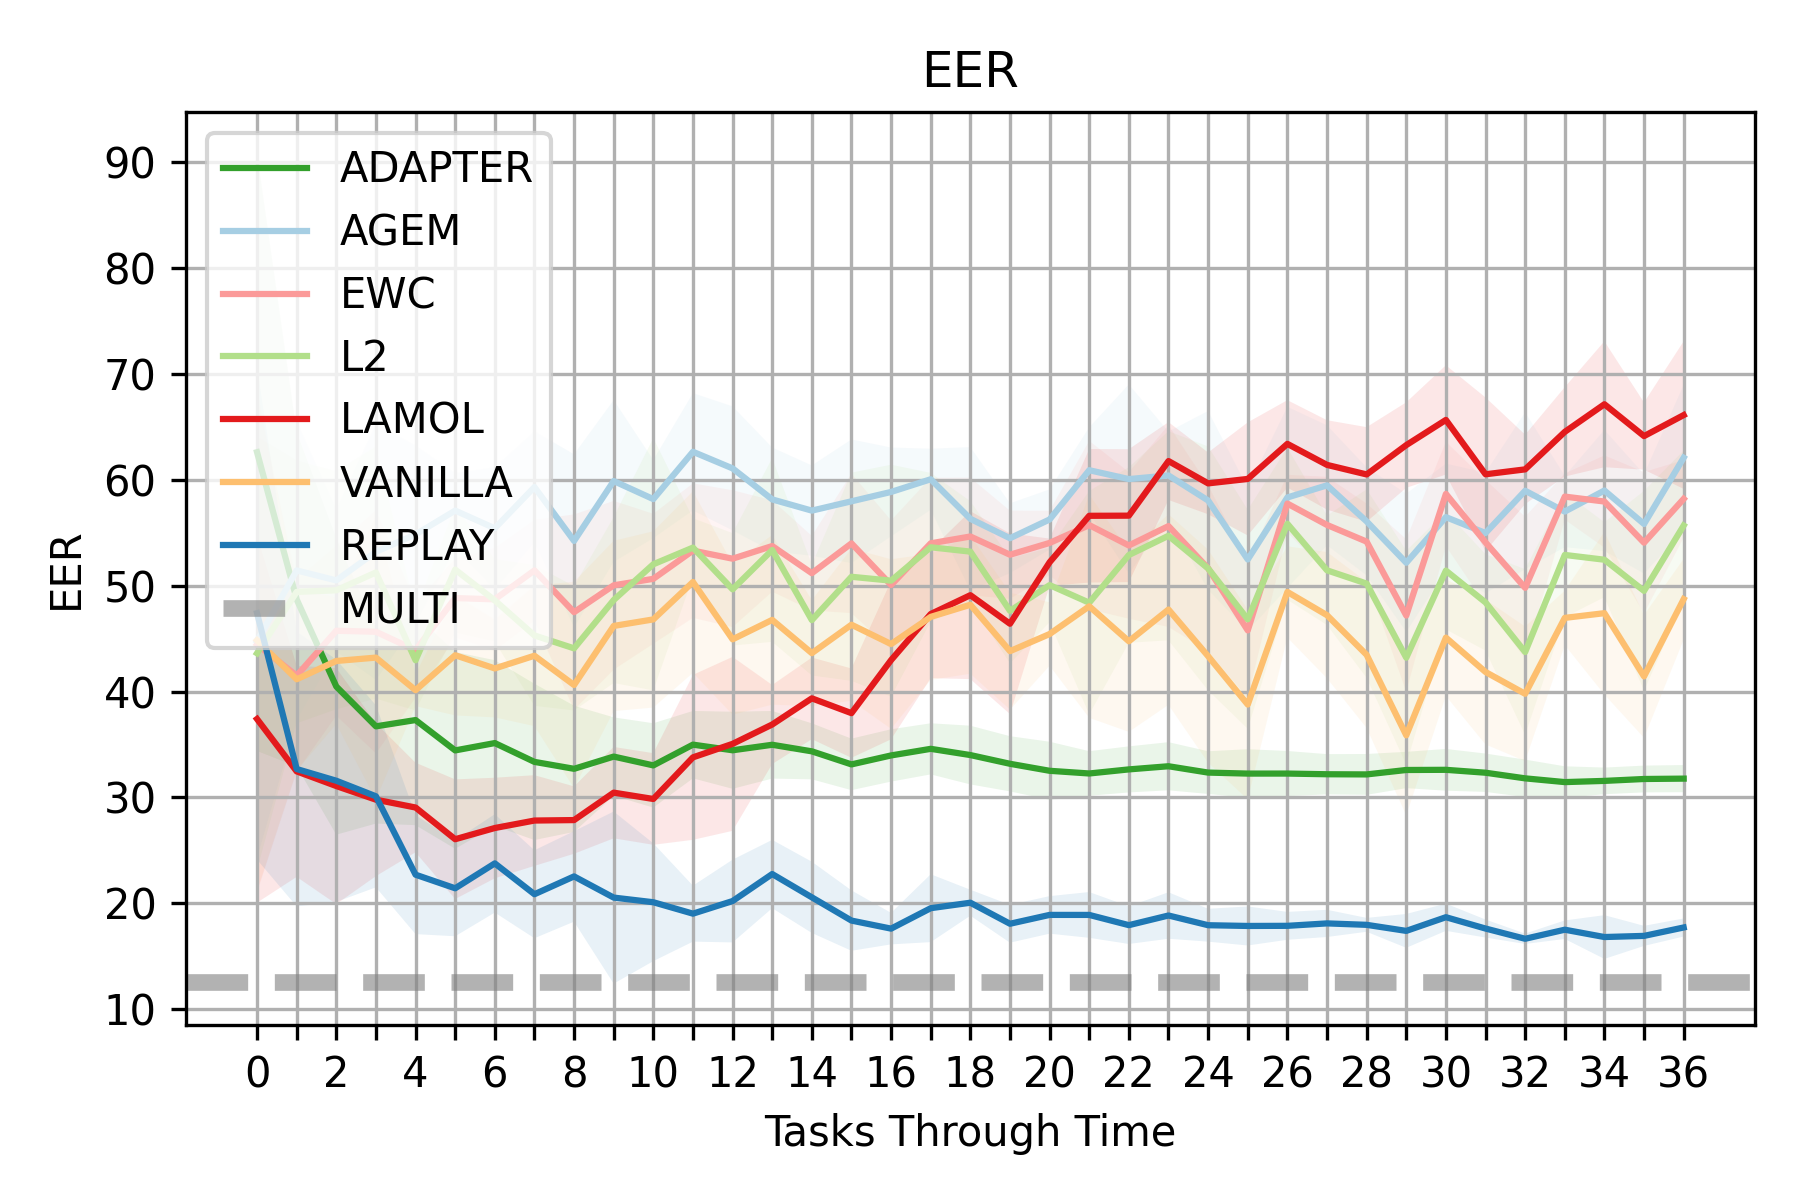}
%     \caption{End-to-end results }
%     \label{fig:E2E}
% \end{figure}

\begin{table*}[t]
\centering
\begin{tabular}{r|cc|c|c|cc}
                                     & \multicolumn{1}{l}{} & \multicolumn{1}{l|}{} & \textbf{INTENT}              & \textbf{DST}            & \multicolumn{2}{c}{\textbf{NLG}}                     \\ \hline
\multicolumn{1}{c|}{\textbf{Method}} & \textbf{+Parm.}      & \textbf{Mem.}         & \textit{Accuracy $\uparrow$} & \textit{JGA $\uparrow$} & \textit{EER $\downarrow$} & \textit{BLEU $\uparrow$} \\ \hline
\textit{VANILLA}              & -           & $\emptyset$           & 3.27  $\pm$ 0.3              & 5.34  $\pm$ 4.4         & 14.81 $\pm$ 7.7           & 11.06 $\pm$ 2.9          \\
\textit{L2}                    & $|\theta|$  & $\emptyset$           & 3.52  $\pm$ 0.7              & 4.95  $\pm$ 4.4         & 12.93 $\pm$ 5.5           & 11.99 $\pm$ 1.4          \\
\textit{EWC}                 & $2|\theta|$ & $\emptyset$           & 3.21  $\pm$ 0.3              & 5.36  $\pm$ 4.3         & 14.2 $\pm$ 6.2            & 11.19 $\pm$ 2.4          \\
\textit{AGEM}                  & -           & $t|M|$                & 9.74  $\pm$ 2.6              & 5.17  $\pm$ 4.0         & 34.2 $\pm$ 8.6            & 5.51 $\pm$ 2.1           \\
\textit{LAMOL}                 & -           & $\emptyset$           & 3.73  $\pm$ 1.0              & 4.03  $\pm$ 3.9         & 29.61 $\pm$ 3.1           & 5.42 $\pm$ 1.7           \\
\textit{REPLAY}                & -           & $t|M|$                & 76.45 $\pm$ 1.5              & \textbf{39.42} $\pm$ 0.2         & \textbf{4.95} $\pm$ 1.5            & \textbf{21.72} $\pm$ 0.3          \\
\textit{ADAPT}                 & $t|\mu|$    & $\emptyset$           & \textbf{85.05} $\pm$ 0.6              & 37.9  $\pm$ 0.6         & 14.36 $\pm$ 0.7           & 21.48 $\pm$ 0.2          \\ \hline
\textit{MULTI}                 & -           & -                     & 87.50 $\pm$ 0.2              & 50.04 $\pm$ 0.1         & 2.84 $\pm$ 0.2            & 26.15 $\pm$ 0.2          \\ \hline
\end{tabular}
    \caption{Modularized Results.}
    \label{tab:modularized_results}
\end{table*}

\begin{table*}[t]
\centering
\begin{tabular}{c|c|c|cc}
\hline
                & \textbf{INTENT}              & \textbf{DST}           & \multicolumn{2}{c}{\textbf{NLG}}                    \\ \hline
$|M|$ & \textit{Accuracy $\uparrow$} & \textit{JGA$\uparrow$} & \textit{EER$\downarrow$} & \textit{BLEU $\uparrow$} \\ \hline
10              & 57.286$\pm$3.80              & 26.63$\pm$1.26         & 8.44$\pm$0.97            & 18.86$\pm$0.68           \\
50              & 76.446$\pm$1.55              & 39.41$\pm$0.28         & 6.63$\pm$0.53            & 21.11$\pm$0.41           \\
100             & 81.496$\pm$0.86              & 43.13$\pm$0.31         & 5.75$\pm$0.19            & 21.71$\pm$0.25           \\
500             & 85.91$\pm$0.55               & 48.22$\pm$0.53         & 4.96$\pm$0.10            & 22.86$\pm$0.25           \\
ALL             & 87.784$\pm$0.16              & 49.97$\pm$0.46         & 4.36$\pm$0.24            & 23.85$\pm$0.12           \\ \hline
MULTI           & 87.5$\pm$0.1                 & 50.04 $\pm$ 0.6        & 3.42$\pm$0.1             & 26.15$\pm$0.1            \\ \hline
\end{tabular}
    \caption{Ablation study over episodic memory size $|\mathcal{M}|$. In the table $|\mathcal{M}|$ represents the number of samples per task kept in memory. }
    \label{tab:ablationmem}
\end{table*}

\begin{table*}[t]
\resizebox{\textwidth}{!}{
\begin{tabular}{r|ccc|ccc|ccc}
\hline
\multicolumn{1}{r}{\textbf{Domains}} & \multicolumn{3}{c}{\textbf{DST-INTENT}}       & \multicolumn{3}{c}{\textbf{NLG}}              & \multicolumn{3}{c}{\textbf{End-to-End}}       \\ \hline
\multicolumn{1}{l}{}                 & \textit{Train} & \textit{Dev} & \textit{Test} & \textit{Train} & \textit{Dev} & \textit{Test} & \textit{Train} & \textit{Dev} & \textit{Test} \\ \hline
\textit{TM19 movie}           & 4733           & 584          & 500           & 3010           & 366          & 341           & 12766          & 1632         & 1481          \\
\textit{TM19 auto}             & 3897           & 448          & 522           & 2128           & 223          & 283           & 10918          & 1248         & 1443          \\
\textit{TM19 restaurant}       & 4434           & 568          & 561           & 2582           & 330          & 333           & 12862          & 1669         & 1630          \\
\textit{TM19 pizza}            & 2883           & 381          & 359           & 1326           & 171          & 171           & 8720           & 1145         & 1083          \\
\textit{TM19 uber}             & 4378           & 535          & 525           & 2418           & 290          & 278           & 11331          & 1362         & 1361          \\
\textit{TM19 coffee}           & 2591           & 302          & 335           & 1381           & 151          & 184           & 7429           & 894          & 936           \\
\textit{TM20 flight}           & 15868          & 1974         & 1940          & 10148          & 1272         & 1245          & 36778          & 4579         & 4569          \\
\textit{TM20 food-ordering}    & 3404           & 411          & 431           & 2394           & 277          & 287           & 7838           & 941          & 986           \\
\textit{TM20 hotel}            & 15029          & 1908         & 1960          & 6590           & 842          & 869           & 35022          & 4400         & 4532          \\
\textit{TM20 music}            & 5917           & 764          & 769           & 4196           & 537          & 523           & 13723          & 1773         & 1787          \\
\textit{TM20 restaurant}       & 13738          & 1761         & 1691          & 8356           & 1063         & 994           & 34560          & 4398         & 4297          \\
\textit{TM20 sport}            & 13072          & 1668         & 1654          & 12044          & 1553         & 1542          & 29391          & 3765         & 3723          \\
\textit{TM20 movie}            & 13221          & 1703         & 1567          & 9406           & 1203         & 1093          & 32423          & 4158         & 3881          \\
\textit{MWOZ taxi}             & 1239           & 234          & 194           & 402            & 71           & 56            & 2478           & 468          & 388           \\
\textit{MWOZ train}            & 1452           & 158          & 160           & 563            & 63           & 59            & 2905           & 316          & 320           \\
\textit{MWOZ restaurant}       & 5227           & 243          & 281           & 3333           & 141          & 177           & 10461          & 486          & 563           \\
\textit{MWOZ hotel}            & 2798           & 289          & 385           & 1924           & 194          & 258           & 5602           & 579          & 771           \\
 \textit{MWOZ attraction}       & 484            & 43           & 42            & 295            & 27           & 26            & 975            & 86           & 85            \\
\textit{sgd restaurants}       & 2686           & 278          & 616           & 1720           & 166          & 386           & 5756           & 606          & 1354          \\
\textit{sgd media}             & 1411           & 230          & 458           & 988            & 167          & 324           & 3114           & 502          & 1005          \\
\textit{sgd events}            & 4881           & 598          & 989           & 3241           & 389          & 590           & 10555          & 1317         & 2197          \\
\textit{sgd music}             & 1892           & 275          & 556           & 1506           & 224          & 464           & 4040           & 597          & 1215          \\
\textit{sgd movies}            & 1665           & 181          & 52            & 996            & 114          & 44            & 3760           & 420          & 126           \\
\textit{sgd flights}           & 4766           & 1041         & 1756          & 2571           & 627          & 982           & 10429          & 2244         & 3833          \\
\textit{sgd ridesharing}       & 652            & 85           & 187           & 377            & 48           & 107           & 1448           & 188          & 418           \\
\textit{sgd rentalcars}        & 1510           & 250          & 469           & 865            & 153          & 280           & 3277           & 538          & 1009          \\
\textit{sgd buses}             & 1862           & 331          & 653           & 1102           & 218          & 412           & 4050           & 709          & 1393          \\
\textit{sgd hotels}            & 3237           & 394          & 948           & 1997           & 243          & 597           & 6983           & 858          & 2053          \\
\textit{sgd services}          & 3328           & 360          & 926           & 2225           & 230          & 611           & 7262           & 803          & 2016          \\
\textit{sgd homes}             & 2098           & 170          & 533           & 1312           & 96           & 338           & 4519           & 394          & 1158          \\
\textit{sgd banks}             & 1188           & 139          & 293           & 723            & 84           & 181           & 2599           & 319          & 667           \\
\textit{sgd calendar}          & 592            & 115          & 236           & 397            & 65           & 133           & 1313           & 246          & 501           \\
\textit{sgd alarm}             & 212            & 34           & 91            & 221            & 30           & 74            & 580            & 82           & 198           \\
\textit{sgd weather}           & 196            & 32           & 80            & 123            & 23           & 59            & 433            & 70           & 169           \\
\textit{sgd travel}            & 186            & 23           & 48            & 121            & 14           & 30            & 420            & 53           & 106           \\
\textit{sgd payment}           & 227            & 21           & 51            & 143            & 14           & 32            & 497            & 44           & 113           \\
\textit{sgd trains}            & 300            & 73           & 128           & 149            & 43           & 66            & 668            & 158          & 274           \\ \hline
\multicolumn{1}{r}{\textbf{Total}}                 & 147254         & 18604        & 22946         & 93273          & 11722        & 14429         & 347885         & 44047        & 53641         \\ \hline
\end{tabular}
}
\caption{All data samples used in the experiments.}
\label{tab:all_data}
\end{table*}

\clearpage
\section*{Chapter 5: Controlling Multi-skill Dialogue Systems}

\section*{A Embedded Representation}
\begin{wrapfigure}{r}{0.5\textwidth}
    \vspace{-30pt}
    % \vspace{-10pt}
  \begin{center}
    \includegraphics[width=\linewidth]{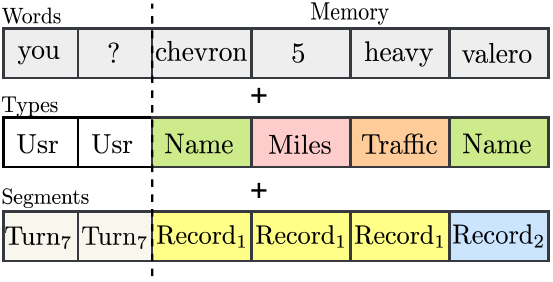}
  \end{center}
    \caption{Positional Embedding of the dialogue history and the memory content.}
    \label{example_position}
    \vspace{-10pt}
\end{wrapfigure}
Since the model input may include structured data (e.g. DB records) we further define another embedding matrix for encoding the types and the segments as $P\in \mathbb{R}^{d \times |S|}$ where $S$ is the set of positional tokens and $|S|$ its cardinality. $P$ is used to inform the model of the token types such as speaker information (e.g. \textit{Sys} and \textit{Usr}), the data-type for the memory content (e.g. \textit{Miles}, \textit{Traffic} etc.), and segment types like dialogue turn information and database record index~\citep{wolf2019transfertransfo}. Figure~\ref{example_position} shows an example of the embedded representation of the input. Hence, we denote $X_T$ and $X_R$ as the type and segment tokens for each token in input $X$, respectively. 

\section*{B Data Pre-Processing}
As mentioned in the main article, we convert MultiWOZ into an end-to-end trainable dataset. This requires to add sql-syntax queries when the system includes particular entities. To do so we leverage two annotations such as the state-tracker and the speech acts. The first is used to generate the a well-formed query, including key and attribute, the second instead to decide when to include the query. More details on the dialogue state-tracker slots and slots value, and the different speech acts can be found in \citep{budzianowski2018multiwoz}. 

A query is create by the slots, and its values, that has been updated in the latest turn. The SQL query uses the following syntax:
\begin{equation}
    \textrm{\textbf{SELECT}} * \textrm{\textbf{FROM }} \textrm{\textit{domain}} \textrm{\textbf{ WHERE }} [\textrm{\textit{slot\_type}}=\textrm{\textit{slot\_value}}]^*  \nonumber
\end{equation}
Similarly for the booking api BOOK the syntax is the following:
\begin{equation}
    \textrm{\textbf{BOOK FROM }} \textrm{\textit{domain}} \textrm{\textbf{ WHERE }} [\textrm{\textit{slot\_type}}=\textrm{\textit{slot\_value}}]^*  \nonumber
\end{equation}
In both cases the slot values are kept as real entities. 

More challenging is to decide when to issue such apis. Speech acts are used to decide by using the "INFORM-DOMAIN" and "RECOMMEND-DOMAIN" tag. Thus any response that include those speech tag will trigger an api if and only if:
\begin{itemize}[leftmargin=*]
    \item there has been a change in the state-tracker from the previous turn
    \item the produced query has never been issued before
\end{itemize}
By a manual checking, this strategy results to be effective. However, as reported by \citep{budzianowski2018multiwoz} the speech act annotation includes some noise, which is reflected also into our dataset. 

The results from the SQL query can be of more that 1K records with multiple attributes. Following \citep{budzianowski2018multiwoz} we use the following strategy:
\begin{itemize}
    \item If no speech act INFORM or RECOMMEND and the number of records are more than 5, we use a special token in the memory $<TM>$.
    \item If no speech act INFORM or RECOMMEND and the number of records are less or equal than 5, we put all the records in memory. 
    \item If any speech act INFORM or RECOMMEND, we filter the records to include based on the act value. Notice that this is a fair strategy, since all the resulting record are correct possible answers and the annotators pick-up on of the record randomly~\citep{budzianowski2018multiwoz}.
\end{itemize} 
 Notice that the answer of a booking call instead, is only one record containing the booking information (e.g. reference number, taxi plate etc.) or "Not Available" token in case the booking cannot made.
 
\section*{C Hyper-parameters and Training}
We used a standard Transformer architecture~\citep{vaswani2017attention} with pre-trained Glove embedding~\citep{pennington2014glove}. For the both Seq2Seq and MoE we use Adam~\citep{kingma2014adam} optimizer with a learning rate of $1\times10^{-3}$, where instead for the Transformer we used a warm-up learning rate strategy as in ~\citep{vaswani2017attention}. In both \textit{AoP} and \textit{AoR} we use an additional transformer layer on top the output of the model. Figure~\ref{fig:moe},\ref{fig:aor},\ref{fig:aop} shows the high level design MoE, AoR and AoP respectively. 
In all the model we used a batch size of 16, and we early stopped the model using the Validation set. All the experiments has been conducted using a single Nvidia 1080ti.

We used a small grid-search for tuning each model. The selected hyper-parameters are reported in Table \ref{Hyper-Paramer}, and we run each experiment 3 times and report the mean and standard deviation of each result.
\begin{table}[ht]
\caption{Hyper-Parameters used for the evaluations.}
\label{Hyper-Paramer}
\resizebox{\textwidth}{!}{
\begin{tabular}{r|cccccccc}
\hline
\multicolumn{1}{l|}{\textit{\textbf{Model}}} & \multicolumn{1}{l}{\textit{\textbf{d}}} & \multicolumn{1}{l}{\textit{\textbf{d$_{model}$}}} & \multicolumn{1}{l}{\textit{\textbf{Layers}}} & \multicolumn{1}{l}{\textit{\textbf{Head}}} & \multicolumn{1}{l}{\textit{\textbf{Depth}}} & \multicolumn{1}{l}{\textit{\textbf{Filter}}} & \multicolumn{1}{l}{\textit{\textbf{GloVe}}} & \multicolumn{1}{l}{\textit{\textbf{Experts}}} \\ \hline
\textit{Seq2Seq} & 100 & 100 & 1 & - & - & - & Yes & - \\ \hline
\textit{TRS} & 300 & 300 & 1 & 2 & 40 & 50 & Yes & - \\ \hline
\textit{MoE} & 100 & 100 & 2 & - & - & - & Yes & 13 \\ \hline
\textit{AoP/AoR}& 300 & 300 & 1 & 2 & 40 & 50 & Yes & 13 \\\hline
\textit{TRS/AoP+U}& 300 & 300 & 6 & 2 & 40 & 50 & Yes & 13 \\\hline
\end{tabular}}
\end{table}

\section*{D MWOZ and SMD with Std.}
\begin{table}[H]
\centering
\resizebox{\textwidth}{!}{%
\begin{tabular}{r|cc|cc|cc}
\hline
\multicolumn{1}{c|}{\textbf{Model}} & \textbf{F1} & \textbf{BLEU} & \textbf{SQL$_{Acc}$} & \textbf{SQL$_{BLEU}$} & \textbf{BOOK$_{Acc}$} & \textbf{BOOK$_{BLEU}$} \\ \hline
\textit{Seq2Seq}        & 38.37 $\pm$ 1.69 &	9.42 $\pm$ 0.38    & 49.97 $\pm$ 3.49 &	81.75 $\pm$ 2.54 & 39.05 $\pm$ 9.52 & 79.00 $\pm$ 3.63 \\ \hline
\textit{TRS}            & 36.91 $\pm$ 1.24 &	9.92 $\pm$ 0.43  & 61.96 $\pm$ 3.95 &	89.08 $\pm$ 1.23 & 46.51 $\pm$ 5.46 & 78.41 $\pm$ 2.03 \\ \hline
\textit{MoE}            & 38.64 $\pm$ 1.11 &	9.47 $\pm$ 0.59   & 53.60 $\pm$ 4.62 &	85.38 $\pm$ 2.68 & 37.23 $\pm$ 3.89 & 78.55 $\pm$ 2.62 \\ \hline
\textit{AoR}        & 40.36 $\pm$ 1.39 &	10.66 $\pm$ 0.34 &	69.39 $\pm$ 1.05 &	90.64 $\pm$ 0.83 &	52.15 $\pm$ 2.22 &	81.15 $\pm$ 0.32             \\ \hline
\textit{AoP}  & \textbf{42.26} $\pm$ 2.39 &	\textbf{11.14} $\pm$ 0.39  &\textbf{71.1} $\pm$ 0.47 &	\textbf{90.90} $\pm$ 0.81 & \textbf{56.31} $\pm$ 0.46 & \textbf{84.08} $\pm$ 0.99 \\ \hline \hline
\textit{TRS + U}        & 39.39 $\pm$ 1.23 &9.29	$\pm$  0.71  & 61.80$\pm$ 4.82 &89.70	$\pm$ 1.40& 50.16$\pm$1.18 & 79.05$\pm$ 1.42 \\ \hline
\textit{AoP + U}        & \textbf{44.04} $\pm$ 0.92 &	\textbf{11.26} $\pm$ 0.07 &	\textbf{74.83} $\pm$ 0.79 &	\textbf{91.90} $\pm$ 1.03 &	\textbf{56.37} $\pm$ 0.92 &	\textbf{84.15} $\pm$ 0.32             \\ \hline \hline
\textit{AoP w/o $\mathcal{L}_{V}$}        & 38.50 $\pm$ 1.15 &	10.50 $\pm$ 0.55    & 61.47 $\pm$ 0.15 &	88.28 $\pm$ 0.50 & 52.61 $\pm$ 0.56 & 80.34 $\pm$ 0.21 \\ \hline
\textit{AoP+O}   & \textit{46.36} $\pm$ 0.92 &	\textit{11.99} $\pm$ 0.03  & \textit{73.41} $\pm$ 0.59 &	\textit{93.81} $\pm$ 0.16 & \textit{56.18}$\pm$ 1.55 & \textit{86.42} $\pm$ 0.92 \\ \hline
\end{tabular}
}
\end{table}

\section*{E Persona Result with Std}
\begin{table}[H]
    \centering
\begin{tabular}{r|cccc}
% \centering
\hline

\textbf{Model} & \textbf{Ppl.} & \textbf{F1} & \textbf{C} & \textbf{BLEU} \\ \hline
\textit{Seq2Seq}         & 39.42 $\pm$ 1.54 &	6.33 $\pm$ 0.58 &	0.11 $\pm$ 0.06 &	2.80 $\pm$ 0.09 \\ \hline
\textit{TRS}             & 43.12 $\pm$ 1.46 &	7.00 $\pm$ 0.00 &	0.07 $\pm$ 0.16 &	2.56 $\pm$ 0.07 \\ \hline
\textit{MoE}             & \textbf{38.63} $\pm$ 0.20 &   \textbf{7.33} $\pm$ 0.05 &	0.19 $\pm$ 0.16 &	2.92 $\pm$ 0.48 \\ \hline
\textit{AoR}             & 40.18 $\pm$ 0.74 &	6.66 $\pm$ 0.05 &	0.12 $\pm$ 0.14 &	2.69 $\pm$ 0.34 \\ \hline
\textit{AoP}             & 39.14 $\pm$ 0.48 &	7.00 $\pm$ 0.00 &	\textbf{0.21} $\pm$ 0.05 &	\textbf{3.06} $\pm$ 0.08 \\ \hline \hline

\textit{TRS + U}         & 43.04$\pm$ 1.78 &	\textbf{7.33}$\pm$ 0.57 & 0.15$\pm$ 0.02 &	2.66$\pm$0.43  \\ \hline
\textit{AoP + U}         & \textbf{37.40}$\pm$0.08  &	7.00$\pm$0.00  &	\textbf{0.29}$\pm$ 0.07 &	\textbf{3.22}$\pm$ 0.04 \\ \hline  \hline
\textit{AoP w/o $\mathcal{L}_{V}$}       & 42.81$\pm$0.01  &	6.66$\pm$0.57  &	0.12$\pm$ 0.04 &	2.85$\pm$ 0.21 \\ \hline
\textit{AoP + O}         & \textit{40.16} $\pm$ 0.56 &	\textit{7.33} $\pm$ 0.58 &	\textit{0.21} $\pm$ 0.14 &	\textit{2.98} $\pm$ 0.05 \\ \hline
\end{tabular}
\end{table}

\section*{F Domain F1-Score}

\begin{table}[H]
\centering
% \resizebox{\textwidth}{!}{%
\begin{tabular}{rccccccc}
\hline
\multicolumn{1}{c|}{\textbf{Sentence}} & \textbf{Seq2Seq} & \textbf{MoE} & \textbf{TRS} & \textbf{AoR} &  \multicolumn{1}{c|}{\textbf{AoP}} & \textbf{Aop+O} \\ \hline
\multicolumn{1}{r|}{\textit{Taxi}} & 71.77 & 75.97 & 73.92 & 76.07  & \multicolumn{1}{c|}{\textbf{76.58}} & 78.30 \\ \hline
\multicolumn{1}{r|}{\textit{Police}} & 49.73 & 49.95 & 50.24 & 51.95  & \multicolumn{1}{c|}{\textbf{56.61}} & 52.05 \\ \hline
\multicolumn{1}{r|}{\textit{Restaurant}} & 50.20 & 49.59 & 48.34 & \textbf{50.58}  & \multicolumn{1}{c|}{50.47} & 50.90 \\ \hline
\multicolumn{1}{r|}{\textit{Hotel}} & \textbf{46.82} & 45.37 & 43.38 & 45.51  & \multicolumn{1}{c|}{46.40} & 44.47 \\ \hline

\multicolumn{1}{r|}{\textit{Attraction}} & 37.87 & 35.21 & 33.10 & 36.97  & \multicolumn{1}{c|}{\textbf{38.79}} & 37.51\\ \hline
\multicolumn{1}{r|}{\textit{Train}} & 46.02 & 41.72 & 41.28 & 44.33  & \multicolumn{1}{c|}{\textbf{46.32}} & 45.93 \\ \hline
\multicolumn{1}{r|}{\textit{Weather}} & 40.38 & 27.06 & 18.97 & 44.77  & \multicolumn{1}{c|}{\textbf{51.94}} & 55.23 \\ \hline
\multicolumn{1}{r|}{\textit{Schedule}} & 35.98 & 43.94 & 38.95 & 32.90 & \multicolumn{1}{c|}{\textbf{54.18}} & 52.99 \\ \hline
\multicolumn{1}{r|}{\textit{Navigate}} & 18.57 & \textbf{21.34} & 6.96 & 12.69  & \multicolumn{1}{c|}{12.18} & 16.56 \\ \hline
\multicolumn{7}{c}{\textbf{BOOK}} \\ \hline
\multicolumn{1}{r|}{\textit{Taxi}} & 23.16 & 32.28 & 30.70 & 41.93  & \multicolumn{1}{c|}{\textbf{46.66}} & 43.15 \\ \hline
\multicolumn{1}{r|}{\textit{Restaurant}} & 45.02 & 28.26 & 49.72 & 55.70  & \multicolumn{1}{c|}{\textbf{58.51}} & 57.70 \\ \hline
\multicolumn{1}{r|}{\textit{Hotel}} & 49.22 & 31.48 & 41.61 & 51.46 &  \multicolumn{1}{c|}{\textbf{56.62}} & 57.41 \\ \hline
\multicolumn{1}{r|}{\textit{Train}} & 55.86 & 56.38 & 57.51 & 57.51  & \multicolumn{1}{c|}{\textbf{59.15}} & 60.80 \\ \hline
\multicolumn{7}{c}{\textbf{SQL}} \\ \hline
\multicolumn{1}{r|}{\textit{Police}} & 81.33 & 0.00 & 90.66& 76.00  &  \multicolumn{1}{c|}{\textbf{93.33}} & 100.0 \\ \hline
\multicolumn{1}{r|}{\textit{Restaurant}} & 71.58 & 68.00 & 75.90 & \textbf{81.27}  & \multicolumn{1}{c|}{80.43} & 84.15 \\ \hline
\multicolumn{1}{r|}{\textit{Hospital}} & 62.22 & 15.55 & 58.89 & 71.11 &  \multicolumn{1}{c|}{\textbf{76.67}} & 83.33 \\ \hline
\multicolumn{1}{r|}{\textit{Hotel}} & 45.25 & 42.09 & 48.61 & 56.69 &  \multicolumn{1}{c|}{\textbf{59.75}} & 63.75 \\ \hline
\multicolumn{1}{r|}{\textit{Attraction}} & 65.48 & 67.69 & 65.91 & 70.61 & \multicolumn{1}{c|}{\textbf{76.22}} & 74.93 \\ \hline
\multicolumn{1}{r|}{\textit{Train}} & 30.02 & 41.01 & 55.67 & 66.61  & \multicolumn{1}{c|}{\textbf{67.34}} & 69.50 \\ \hline
\end{tabular}
% }
\caption{Per Domain F1 Score.}
\end{table}

\begin{figure}[t]
    \centering
    \includegraphics[width=0.98\linewidth]{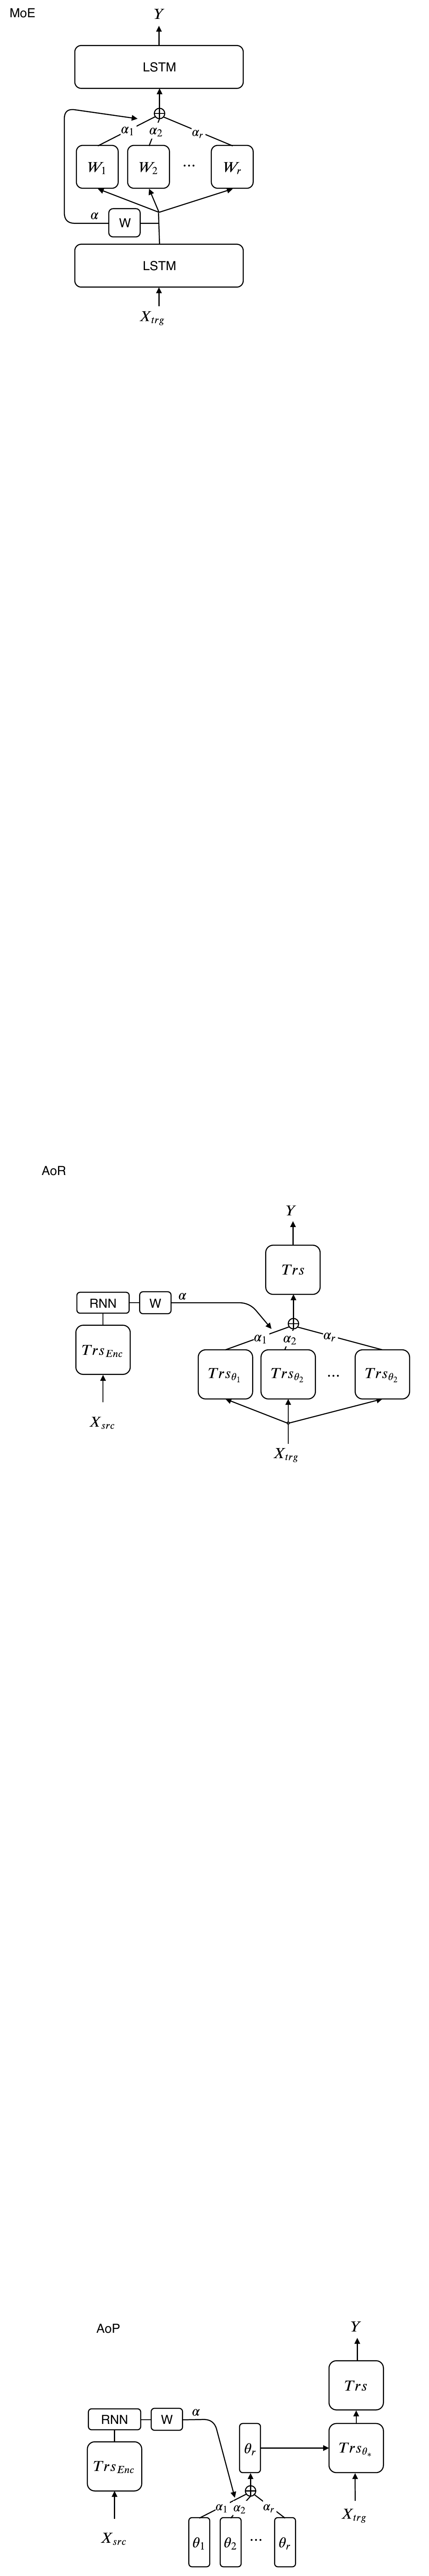}
    \caption{Mixture of Experts (MoE)~\citep{shazeer2017outrageously} model consist of $r$ feed-forward neural network (experts) which are embedded between two LSTM layers, a trainable gating network to select experts.}
    \label{fig:moe}
\end{figure}

\begin{figure}[t]
    \centering
    \includegraphics[width=0.98\linewidth]{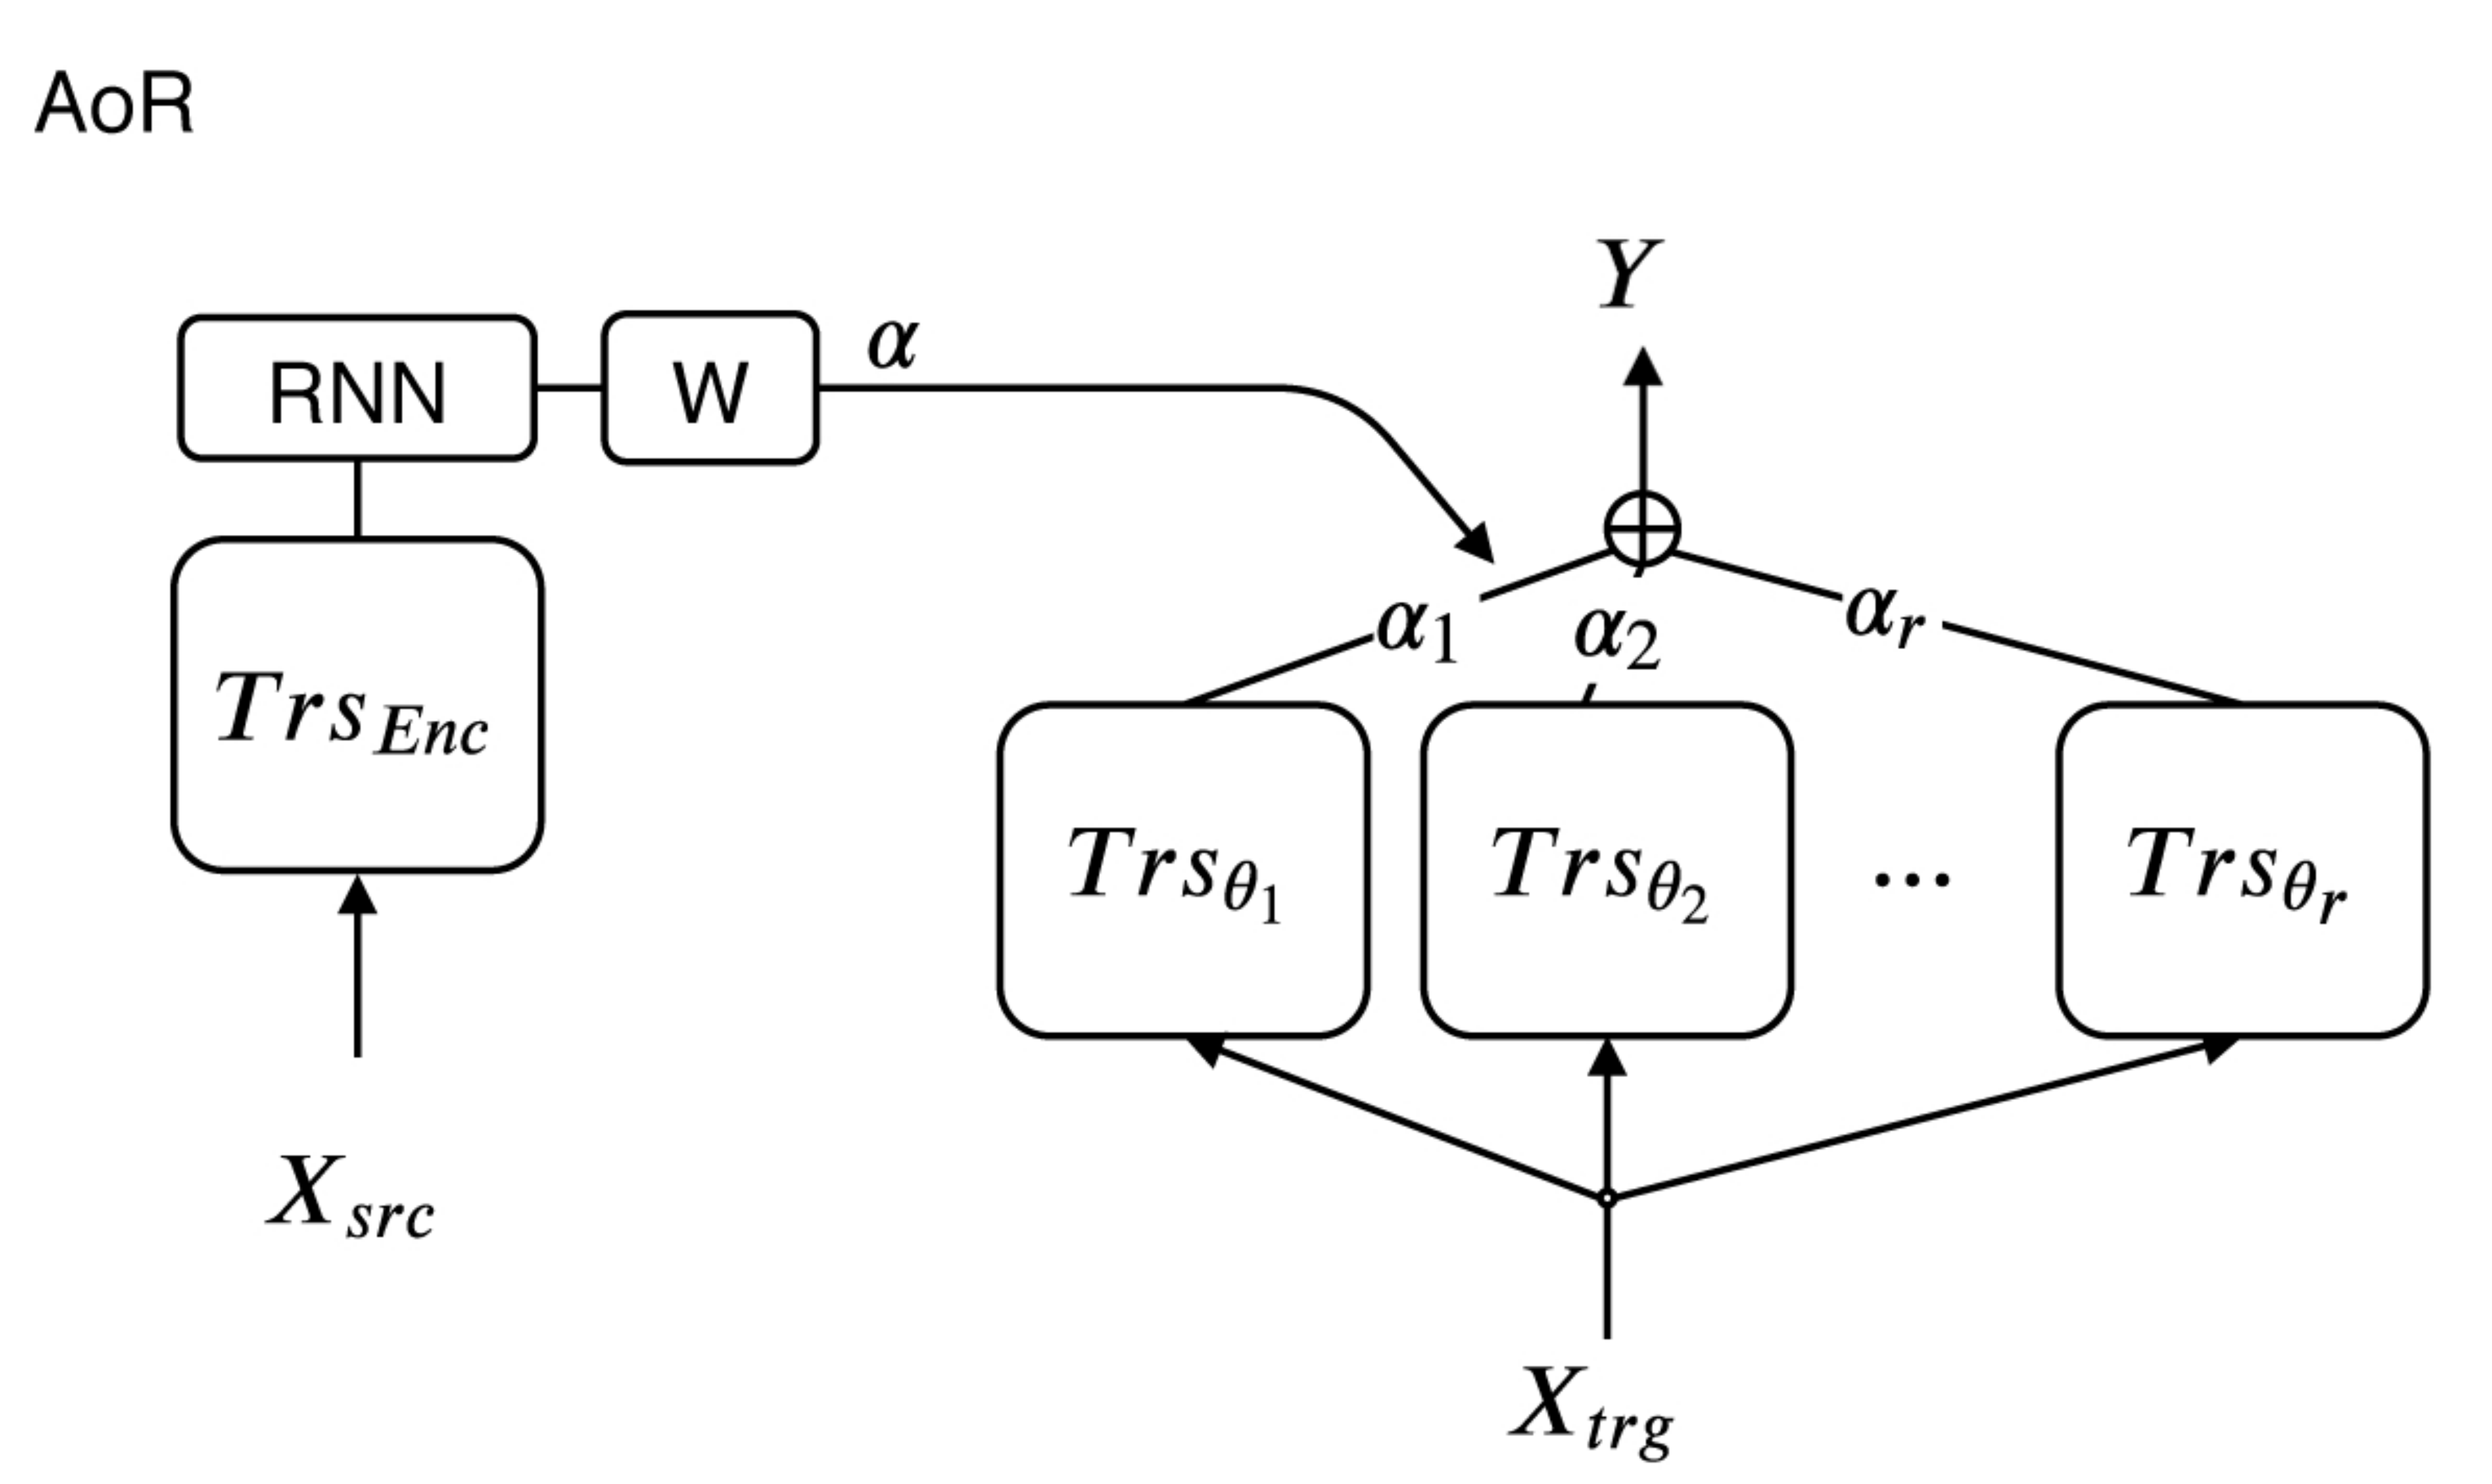}
    \caption{Attention over Representation (AoR) consist of a transformer encoder which encode the source input and compute the attention over the skills. Then $r$ transformer decoder layers computes $r$ specialized representation and the output response is generated based on the weighted sum the representation. In the figure, we omitted the output layer.}
    \label{fig:aor}
\end{figure}

\begin{figure}[t]
    \centering
    \includegraphics[width=0.98\linewidth]{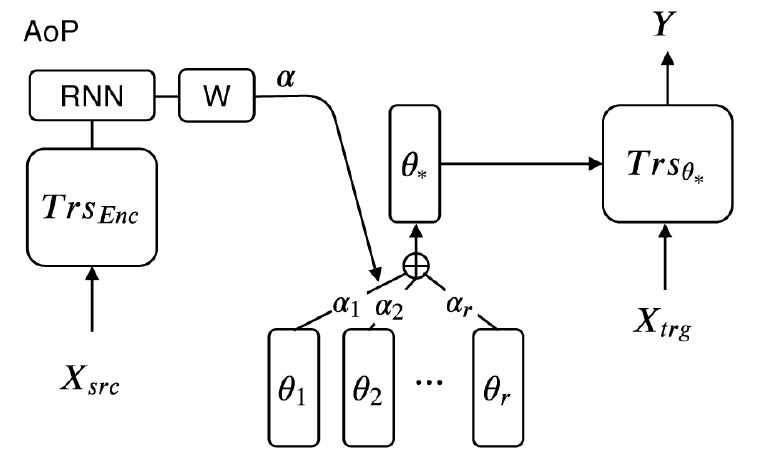}
    \caption{Attention over Parameters (AoP) consist of a transformer encoder which encode the source input and compute the attention over the skills. Then, $r$ specialized transformer decoder layers and a dummy transformer decoder layer parameterized by the weighted sum of the $r$ specialized transformer decoder layers parameters. In the figure, we omitted the output layer.}
    \label{fig:aop}
\end{figure}
